# Supplementary material for: Representational Continuity for Unsupervised Continual Learning
Source: arXiv:2110.06976 source file (2022-04-05)
Supplement: Supplementary file 1 [file 7_appendix_table_1.tex]

\begin{table}[t]
\caption{Continual learning comparison.}
\label{tab:unlabel}
\setlength{\tabcolsep}{3pt} % 
\resizebox{\textwidth}{!}{
\begin{tabular}{ll@{\hspace{6pt}}ccccccc}
\toprule
& {\textbf{Method}}&\multicolumn{2}{c}{\textbf{Split CIFAR-10}} &\multicolumn{2}{c}{\textbf{Split CIFAR-100}}&\multicolumn{2}{c}{\textbf{Mini-ImageNet}} \\
\midrule
& & Accuracy & Forgetting & Accuracy & Forgetting & Accuracy & Forgetting\\
\midrule
& \multicolumn{7}{c}{Linear Classifier} \\
\midrule
\parbox[t]{2mm}{\multirow{7}{*}{\rotatebox[origin=c]{90}{\small  Supervised}}}
& FINETUNE & 
{85.73} \scriptsize($\pm$ 1.58) & {11.34} \scriptsize($\pm$ 1.51) & 
{71.70} \scriptsize($\pm$ 1.05) & {20.21} \scriptsize($\pm$ 1.34) & 
{xx.xx} \scriptsize($\pm$ x.xx) & {x.xx} \scriptsize($\pm$ x.xx) \\

& SI~\citep{zenke17si} & 
{90.44} \scriptsize($\pm$ 0.43) & {~~6.10} \scriptsize($\pm$ 0.40) & 
{75.97} \scriptsize($\pm$ 1.53) & {15.45} \scriptsize($\pm$ 1.63) & 
{xx.xx} \scriptsize($\pm$ x.xx) & {x.xx} \scriptsize($\pm$ x.xx) \\

& A-GEM~\citep{chaudhry2018efficient} & 
{84.63} \scriptsize($\pm$ 2.89) & {11.65} \scriptsize($\pm$ 2.94) & 
{71.50} \scriptsize($\pm$ 0.59) & {19.06} \scriptsize($\pm$ 0.64) & 
{xx.xx} \scriptsize($\pm$ x.xx) & {x.xx} \scriptsize($\pm$ x.xx) \\

& GSS~\citep{aljundi2019gradient} & 
{\bf 92.73} \scriptsize($\pm$ 0.63) & {\bf ~~4.26} \scriptsize($\pm$ 0.40) & 
{78.23} \scriptsize($\pm$ 1.21) & {13.68} \scriptsize($\pm$ 1.21) & 
{xx.xx} \scriptsize($\pm$ x.xx) & {x.xx} \scriptsize($\pm$ x.xx) \\

& DER~\citep{buzzega2020dark} & 
{92.52} \scriptsize($\pm$ 4.36) & {~~4.36} \scriptsize($\pm$ 1.02) & 
{81.84} \scriptsize($\pm$ 1.60) & {\bf 10.04} \scriptsize($\pm$ 1.34) & 
{xx.xx} \scriptsize($\pm$ x.xx) & {x.xx} \scriptsize($\pm$ x.xx) \\

& Uniform & 
{91.54} \scriptsize($\pm$ 0.78) & {~~5.57} \scriptsize($\pm$ 0.71) & 
{\bf 81.87} \scriptsize($\pm$ 0.99) & {10.67} \scriptsize($\pm$ 0.95) & 
{xx.xx} \scriptsize($\pm$ x.xx) & {x.xx} \scriptsize($\pm$ x.xx) \\
\cmidrule{2-9}
& MULTITASK & {97.11} \scriptsize($\pm$ 0.35) & $-$ & {94.43} \scriptsize($\pm$ 0.08) & $-$ \\
\midrule
\parbox[t]{2mm}{\multirow{6}{*}{\rotatebox[origin=c]{90}{\small Unsupervised}}}
& FINETUNE & 
{89.15} \scriptsize($\pm$ 1.14) & {~~5.73} \scriptsize($\pm$ 2.15) & 
{74.04} \scriptsize($\pm$ 0.74) & {10.91} \scriptsize($\pm$ 1.03) & 
{xx.xx} \scriptsize($\pm$ x.xx) & {x.xx} \scriptsize($\pm$ x.xx) \\

& SI~\citep{zenke17si} & 
{84.33} \scriptsize($\pm$ 2.91) & {~~8.75} \scriptsize($\pm$ 2.05) & 
\modified{80.30} \scriptsize($\pm$ 0.xx) & \modified{~~0.68} \scriptsize($\pm$ x.xx) & %lambda=100
%{74.14} \scriptsize($\pm$ 0.88) & {~~9.93} \scriptsize($\pm$ 1.12) & 
{xx.xx} \scriptsize($\pm$ x.xx) & {x.xx} \scriptsize($\pm$ x.xx) \\

& Uniform & 
{\bf 89.67} \scriptsize($\pm$ 1.48) & {~~5.04} \scriptsize($\pm$ 0.83) & 
{65.11} \scriptsize($\pm$ 3.59) & {18.32} \scriptsize($\pm$ 2.86) & 
{xx.xx} \scriptsize($\pm$ x.xx) & {x.xx} \scriptsize($\pm$ x.xx) \\

& DER & {88.29} \scriptsize($\pm$ 2.78) & {~~4.08} \scriptsize($\pm$ 2.65) & {59.93} \scriptsize($\pm$ 1.09) & {24.24} \scriptsize($\pm$ 0.82) \\

& MIXUP & {84.12} \scriptsize($\pm$ 1.64) & {\bf ~~2.14} \scriptsize($\pm$ 1.24) & {\bf 75.50} \scriptsize($\pm$ 1.45) & {\bf ~~2.24} \scriptsize($\pm$ 0.83) \\
\cmidrule{2-9}
& MULTITASK & {96.04} \scriptsize($\pm$ 0.26) & $-$ & {87.75} \scriptsize($\pm$ 0.36) & $-$ \\
\midrule

& \multicolumn{7}{c}{K-Nearest Neighbours} \\
\midrule
\parbox[t]{2mm}{\multirow{7}{*}{\rotatebox[origin=c]{90}{\small Supervised}}}
& FINETUNE & 
{82.87} \scriptsize($\pm$ 0.47) & {14.26} \scriptsize($\pm$ 0.52) &
{61.08} \scriptsize($\pm$ 0.04) & {31.23} \scriptsize($\pm$ 0.41) &
{xx.xx} \scriptsize($\pm$ x.xx) & {x.xx} \scriptsize($\pm$ x.xx) \\

& SI~\citep{zenke17si} & 
%\modified{93.76} \scriptsize($\pm$ x.xx) & \modified{~~1.62} \scriptsize($\pm$ 0.xx) & %lambda=100
{85.18} \scriptsize($\pm$ 0.65) & {11.39} \scriptsize($\pm$ 0.77) & 
%\modified{69.55} \scriptsize($\pm$ 0.37) & \modified{~-0.20} \scriptsize($\pm$ 0.34) & %lambda=100
{63.58} \scriptsize($\pm$ 0.37) & {27.98} \scriptsize($\pm$ 0.34) & 
{xx.xx} \scriptsize($\pm$ x.xx) & {x.xx} \scriptsize($\pm$ x.xx) \\

& A-GEM~\citep{chaudhry2018efficient} & 
{82.41} \scriptsize($\pm$ 1.24) & {13.82} \scriptsize($\pm$ 1.27) &
{59.81} \scriptsize($\pm$ 1.07) & {30.08} \scriptsize($\pm$ 0.91) & 
{xx.xx} \scriptsize($\pm$ x.xx) & {x.xx} \scriptsize($\pm$ x.xx) \\

& GSS~\citep{aljundi2019gradient} & 
{89.49} \scriptsize($\pm$ 1.75) & {~~7.50} \scriptsize($\pm$ 1.52) & 
{70.78} \scriptsize($\pm$ 1.67) & {21.28} \scriptsize($\pm$ 1.52) & 
{xx.xx} \scriptsize($\pm$ x.xx) & {x.xx} \scriptsize($\pm$ x.xx) \\

& DER~\citep{buzzega2020dark} & 
{91.35} \scriptsize($\pm$ 0.46) & {~~5.65} \scriptsize($\pm$ 0.35) & 
{79.52} \scriptsize($\pm$ 1.88) & {12.80} \scriptsize($\pm$ 1.47) & 
{xx.xx} \scriptsize($\pm$ x.xx) & {x.xx} \scriptsize($\pm$ x.xx) \\

& Uniform & 
{\bf 92.15} \scriptsize($\pm$ 0.77) & {\bf ~~4.99} \scriptsize($\pm$ 0.53) & 
{\bf 81.21} \scriptsize($\pm$ 0.91) & {\bf 11.52} \scriptsize($\pm$ 0.91) & 
{xx.xx} \scriptsize($\pm$ x.xx) & {x.xx} \scriptsize($\pm$ x.xx) \\

\cmidrule{2-9}
& MULTITASK & {97.77} \scriptsize($\pm$ 0.15) & $-$ & {93.89} \scriptsize($\pm$ 0.78) & $-$ \\
\midrule
\parbox[t]{2mm}{\multirow{6}{*}{\rotatebox[origin=c]{90}{\small Unsupervised}}}
& FINETUNE & 
{90.11} \scriptsize($\pm$ 0.12) & {~~5.42} \scriptsize($\pm$ 0.08) & 
{\bf 75.42} \scriptsize($\pm$ 0.78) & {10.19} \scriptsize($\pm$ 0.37) & 
{xx.xx} \scriptsize($\pm$ x.xx) & {x.xx} \scriptsize($\pm$ x.xx) \\

& SI~\citep{zenke17si} & 
\modified{92.73} \scriptsize($\pm$ x.xx) & \modified{~~2.09} \scriptsize($\pm$ x.xx) & %lambda=100
%\TBD{85.78} \scriptsize($\pm$ 1.31) & \TBD{~~7.63} \scriptsize($\pm$ 1.11) & 
\modified{78.84} \scriptsize($\pm$ x.xx) & \modified{~~5.40} \scriptsize($\pm$ x.xx) & %lambda=100
%\TBD{74.80} \scriptsize($\pm$ 1.17) & \TBD{10.66} \scriptsize($\pm$ 0.91) &
{xx.xx} \scriptsize($\pm$ x.xx) & {x.xx} \scriptsize($\pm$ x.xx) \\
 
& Uniform & 
{\bf 91.06} \scriptsize($\pm$ 0.34) & {~~3.41} \scriptsize($\pm$ 0.27) & 
\modified{79.46} \scriptsize($\pm$ x.xx) & \modified{~~5.23} \scriptsize($\pm$ x.xx) & %lambda=0.1
%\TBD{65.51} \scriptsize($\pm$ 3.40) & \TBD{17.86} \scriptsize($\pm$ 3.16) & 
{xx.xx} \scriptsize($\pm$ x.xx) & {x.xx} \scriptsize($\pm$ x.xx) \\

& DER & 
{87.39} \scriptsize($\pm$ 0.54) & {~~1.27} \scriptsize($\pm$ 0.19) & 
{69.11} \scriptsize($\pm$ 1.26) & {13.00} \scriptsize($\pm$ 0.89) & 
{xx.xx} \scriptsize($\pm$ x.xx) & {x.xx} \scriptsize($\pm$ x.xx) \\

& MIXUP & 
{85.14} \scriptsize($\pm$ 2.41) & {\bf ~~0.57} \scriptsize($\pm$ 0.51) & 
\modified{81.23} \scriptsize($\pm$ 0.xx) & \modified{~~0.62} \scriptsize($\pm$ 0.xx) & %lambda=1
%\TBD{69.29} \scriptsize($\pm$ 0.33) & \TBD{\bf ~~0.56} \scriptsize($\pm$ 0.08) & 
{xx.xx} \scriptsize($\pm$ x.xx) & {x.xx} \scriptsize($\pm$ x.xx) \\
& MIXUP-Reservoir & 
{xx.xx} \scriptsize($\pm$ x.xx) & {~~x.xx} \scriptsize($\pm$ x.xx) & 
\modified{78.03} \scriptsize($\pm$ x.xx) & \modified{~~6.88} \scriptsize($\pm$ x.xx) & % lambda=10
%\TBD{xx.xx} \scriptsize($\pm$ x.xx) & \TBD{~~x.xx} \scriptsize($\pm$ x.xx) & 
{xx.xx} \scriptsize($\pm$ x.xx) & {x.xx} \scriptsize($\pm$ x.xx) \\

\cmidrule{2-9}
& MULTITASK & {95.76} \scriptsize($\pm$ 0.08) & $-$ & {86.31} \scriptsize($\pm$ 0.38) & $-$ \\
\bottomrule
\end{tabular}}
\end{table}
