# Supplementary material for: Representational Continuity for Unsupervised Continual Learning
Source: arXiv:2110.06976 source file (2022-04-05)
Supplement: Supplementary file 2 [file 7_appendix_table_2.tex]

\begin{table}[t]
\caption{Evaluation on OOD tasks.}
\label{tab:unlabel}

\setlength{\tabcolsep}{3pt} % 
\resizebox{\textwidth}{!}{
\begin{tabular}{ll@{\hspace{6pt}}ccccccccccc}
\toprule
& {\textbf{In-Class}}&\multicolumn{4}{c}{\textbf{Split CIFAR-100}} &\multicolumn{4}{c}{\textbf{Split CIFAR-10}} \\
% \cmidrule{3-7} \cmidrule{8-12}
\cmidrule(l{3pt}r{3pt}){1-2} \cmidrule(l{3pt}r{3pt}){3-6} \cmidrule(l{3pt}r{3pt}){6-9}
& {\bf Out-of-Class} & MNIST & FMNIST & SVHN & CIFAR-10 &  MNIST & FMNIST & SVHN\\
\midrule
& \multicolumn{8}{c}{Linear Classifier} \\
\midrule
\parbox[t]{2mm}{\multirow{7}{*}{\rotatebox[origin=c]{90}{\small  Supervised}}}
& \textsc{Finetune} & 
{ 94.01} (\scriptsize $\pm$ 1.81) & {83.44} (\scriptsize $\pm$ 2.87) & 
{52.73} (\scriptsize $\pm$ 3.01) & {46.76} (\scriptsize $\pm$ 1.93) & 
{ xx.xx} (\scriptsize $\pm$ x.xx) & { x.xx} (\scriptsize $\pm$ x.xx) \\

& \textsc{SI}~\citep{zenke17si} & 
{ 94.72} (\scriptsize $\pm$ 1.71) & {\bf 84.68} (\scriptsize $\pm$ 2.32) & 
{\bf 57.11} (\bf \scriptsize $\pm$ 2.77) & {45.93} (\scriptsize $\pm$ 3.09) & 
{ xx.xx} (\scriptsize $\pm$ x.xx) & { x.xx} (\scriptsize $\pm$ x.xx) \\
 
 & \textsc{AGEM}~\citep{chaudhry2018efficient} & 
{94.82} (\bf \scriptsize $\pm$ 2.07) & {83.96} (\scriptsize $\pm$ 2.18) & 
{52.48} (\scriptsize $\pm$ 1.76) & {47.16} (\scriptsize $\pm$ 2.87) & 
{ xx.xx} (\scriptsize $\pm$ x.xx) & { x.xx} ($\pm$ x.xx) \\

& \textsc{GSS}~\citep{aljundi2019gradient} & 
{ 92.70} (\scriptsize $\pm$ 2.07) & {79.98} (\scriptsize $\pm$ 3.11) & 
{48.69} (\scriptsize $\pm$ 3.96) & {49.41} (\scriptsize $\pm$ 1.81) & 
{ xx.xx} (\scriptsize $\pm$ x.xx) & { x.xx} (\scriptsize $\pm$ x.xx) \\

& \textsc{DER}~\citep{buzzega2020dark} & 
{\bf 95.05} (\scriptsize $\pm$ 0.85) & {81.37} (\scriptsize $\pm$ 2.57) & 
{44.54} (\scriptsize $\pm$ 3.86) & {\bf 59.07} (\scriptsize $\pm$ 1.06) & 
{ xx.xx} (\scriptsize $\pm$ x.xx) & { x.xx} (\scriptsize $\pm$ x.xx) \\

& \textsc{Uniform} & 
{93.48} (\scriptsize $\pm$ 2.38) & {79.87} (\bf \scriptsize $\pm$ 0.15) & 
{46.30} (\scriptsize $\pm$ 3.26) & {57.71} (\scriptsize $\pm$ 1.81) & 
{ xx.xx} (\scriptsize $\pm$ x.xx) & { x.xx} (\scriptsize $\pm$ x.xx) \\

\cmidrule(l{3pt}r{3pt}){2-2} \cmidrule(l{3pt}r{3pt}){3-7} \cmidrule(l{3pt}r{3pt}){8-12}
& \textsc{Multitask} & { 95.50} (\scriptsize $\pm$ 1.58) & {87.05} (\scriptsize $\pm$ 0.40) & { 54.04} (\scriptsize $\pm$ 3.68) & {73.18} (\scriptsize $\pm$ 1.70) \\
\midrule
\parbox[t]{2mm}{\multirow{4}{*}{\rotatebox[origin=c]{90}{ \small Unsupervised}}}
& \textsc{Finetune} & 
{\bf 94.46} (\bf \scriptsize $\pm$ 1.80) & {79.09} (\scriptsize $\pm$ 0.58) & 
{\bf 58.72} (\bf \scriptsize $\pm$ 2.10) & {\bf 61.22} (\scriptsize $\pm$ 3.11) & 
{ xx.xx} (\scriptsize $\pm$ x.xx) & { x.xx} (\scriptsize $\pm$ x.xx) \\

& \textsc{Si}~\citep{zenke17si} & 
{ 92.52} (\scriptsize $\pm$ 0.69) & {\bf 80.03} (\bf \scriptsize $\pm$ 1.06) & 
{ 39.01} (\scriptsize $\pm$ 0.13) & {53.04} (\scriptsize $\pm$ 3.83) & 
{ xx.xx} (\scriptsize $\pm$ x.xx) & { x.xx} (\scriptsize $\pm$ x.xx) \\
 
& \textsc{Uniform} & 
{ 86.83} (\scriptsize $\pm$ 1.83) & { 61.72} (\scriptsize $\pm$ 2.07) & 
{ 37.65} (\scriptsize $\pm$ 0.49) & {48.09} (\scriptsize $\pm$ 3.27) & 
{ xx.xx} (\scriptsize $\pm$ x.xx) & { x.xx} (\scriptsize $\pm$ x.xx) \\

& \textsc{DER} & 
{82.56} (\scriptsize $\pm$ 3.54) & {74.78} (\scriptsize $\pm$ 0.09) & 
{37.53} (\scriptsize $\pm$ 0.66) & {43.23} (\scriptsize $\pm$ 4.48) & 
{ xx.xx} (\scriptsize $\pm$ x.xx) & { x.xx} (\scriptsize $\pm$ x.xx) \\

& \textsc{Mixup} & 
{82.56} (\scriptsize $\pm$ 3.54) & {74.78} (\scriptsize $\pm$ 0.09) & 
{37.53} (\scriptsize $\pm$ 0.66) & {52.73} (\scriptsize $\pm$ 4.08) & 
{ xx.xx} (\scriptsize $\pm$ x.xx) & { x.xx} (\scriptsize $\pm$ x.xx) \\

\cmidrule(l{3pt}r{3pt}){2-2} \cmidrule(l{3pt}r{3pt}){3-7} \cmidrule(l{3pt}r{3pt}){8-12}
& \textsc{Multitask} & { 92.29} (\scriptsize $\pm$ 3.37) & {86.12} (\scriptsize $\pm$ 1.86) & {54.95} (\scriptsize $\pm$ 1.77) & {73.62} (\scriptsize $\pm$ 0.06)\\
\midrule
\
& \multicolumn{7}{c}{K-Nearest Neighbours} \\
\midrule
\parbox[t]{2mm}{\multirow{7}{*}{\rotatebox[origin=c]{90}{\small Supervised}}}
& \textsc{Finetune} & 
{75.02} (\scriptsize $\pm$ 3.97) & {62.37} (\scriptsize $\pm$ 3.20) & 
{38.05} (\scriptsize $\pm$ 0.73) & {39.18} (\scriptsize $\pm$ 0.83) & 
{ xx.xx} (\scriptsize $\pm$ x.xx) & { x.xx} (\scriptsize $\pm$ x.xx) \\

& \textsc{SI}~\citep{zenke17si} & 
{79.96} (\scriptsize $\pm$ 2.63) & {63.71} (\scriptsize $\pm$ 1.36) & 
{40.92} (\scriptsize $\pm$ 1.64) & {40.41} (\scriptsize $\pm$ 1.71) & 
{ xx.xx} (\scriptsize $\pm$ x.xx) & { x.xx} (\scriptsize $\pm$ x.xx) \\
 
& \textsc{AGEM}~\citep{chaudhry2018efficient} & 
{77.56} (\scriptsize $\pm$ 3.21) & {64.16} (\scriptsize $\pm$ 2.29) & 
{37.48} (\scriptsize $\pm$ 1.73) & 
{37.91} (\scriptsize $\pm$ 1.33) & { x.xx} (\scriptsize $\pm$ x.xx) \\

& \textsc{GSS}~\citep{aljundi2019gradient} & 
{76.54} (\scriptsize $\pm$ 0.46) & {65.31} (\scriptsize $\pm$ 1.72) & 
{35.72} (\scriptsize $\pm$ 2.37) & {49.41} (\scriptsize $\pm$ 1.81) & 
{ xx.xx} (\scriptsize $\pm$ x.xx) & { x.xx} (\scriptsize $\pm$ x.xx) \\

& \textsc{DER}~\citep{buzzega2020dark} & 
{\bf 87.71} (\bf \scriptsize $\pm$ 2.23) & {\bf 75.97} (\bf \scriptsize $\pm$ 1.29) & 
{\bf 50.26} (\bf \scriptsize $\pm$ 0.95) & {\bf 59.07} (\bf \scriptsize $\pm$ 1.06) & 
{ xx.xx} (\scriptsize $\pm$ x.xx) & { x.xx} (\scriptsize $\pm$ x.xx) \\

& \textsc{Uniform} & 
{85.14} (\scriptsize $\pm$ 1.20) & { 74.74} (\scriptsize $\pm$ 1.41) & 
{48.98} (\scriptsize $\pm$ 0.71) & {55.27} (\scriptsize $\pm$ 0.59) & 
{ xx.xx} (\scriptsize $\pm$ x.xx) & { x.xx} (\scriptsize $\pm$ x.xx) \\

\cmidrule(l{3pt}r{3pt}){2-2} \cmidrule(l{3pt}r{3pt}){3-7} \cmidrule(l{3pt}r{3pt}){8-12}
 & \textsc{multitask} & { 92.29} (\scriptsize $\pm$ 3.37) & {86.12} (\scriptsize $\pm$ 1.87) & { 54.94} (\scriptsize $\pm$ 1.77) & { 54.04} (\scriptsize $\pm$ 3.68) \\
 
\midrule
\parbox[t]{2mm}{\multirow{6}{*}{\rotatebox[origin=c]{90}{ \small Unsupervised}}}
& \textsc{Finetune} & 
{85.99} (\scriptsize $\pm$ 0.86) & {76.90} (\scriptsize $\pm$ 0.11) & 
{\bf 50.09} (\bf \scriptsize $\pm$ 1.41) & {57.15} (\scriptsize $\pm$ 0.96) & 
{ xx.xx} (\scriptsize $\pm$ x.xx) & { x.xx} (\scriptsize $\pm$ x.xx) \\

& \textsc{SI}~\citep{zenke17si} & 
{85.76} (\scriptsize $\pm$ 0.51) & {77.00} (\scriptsize $\pm$ 0.11) & 
{49.23} (\scriptsize $\pm$ 1.14) & {\bf 57.37} (\bf \scriptsize $\pm$ 0.97) & 
{ xx.xx} (\scriptsize $\pm$ x.xx) & { x.xx} (\scriptsize $\pm$ x.xx) \\
 
& \textsc{Uniform} & 
{82.56} (\scriptsize $\pm$ 3.54) & {74.78} (\scriptsize $\pm$ 0.09) & 
{37.53} (\scriptsize $\pm$ 0.66) & {47.58} (\scriptsize $\pm$ 3.45) & 
{ xx.xx} (\scriptsize $\pm$ x.xx) & { x.xx} (\scriptsize $\pm$ x.xx) \\

& \textsc{DER} & 
{83.08} (\scriptsize $\pm$ 1.26) & {76.21} (\scriptsize $\pm$ 0.62) & 
{44.01} (\scriptsize $\pm$ 2.21) & {54.68} (\scriptsize $\pm$ 0.32) & 
{ xx.xx} (\scriptsize $\pm$ x.xx) & { x.xx} (\scriptsize $\pm$ x.xx) \\

& \textsc{Mixup} & 
{\bf 87.07} (\bf \scriptsize $\pm$ 1.58) & {\bf 78.91} (\bf \scriptsize $\pm$ 1.38) & 
{38.93} (\scriptsize $\pm$ 0.79) & {52.95} (\scriptsize $\pm$ 0.42) & 
{ xx.xx} (\scriptsize $\pm$ x.xx) & { x.xx} (\scriptsize $\pm$ x.xx) \\

\cmidrule(l{3pt}r{3pt}){2-2} \cmidrule(l{3pt}r{3pt}){3-7} \cmidrule(l{3pt}r{3pt}){8-12}
 & \textsc{Multitask} & { 90.35} (\scriptsize $\pm$ 0.24) & {81.11} (\scriptsize $\pm$ 1.86) & { 52.20} (\scriptsize $\pm$ 0.61) & $-$  \\
\bottomrule
\end{tabular}}
\end{table}
