# Supplementary material for: Representational Continuity for Unsupervised Continual Learning
Source: arXiv:2110.06976 source file (2022-04-05)
Supplement: Supplementary file 3 [file 7_appendix_figure_1.tex]

\begin{figure*}[t!]
\small
\begin{minipage}[t]{1.05\linewidth}
\resizebox{\linewidth}{!}{%
\begin{tabular}{c cccc ccc}
\hspace{-0.2in}
\rb{\includegraphics[width=0.13\textwidth]{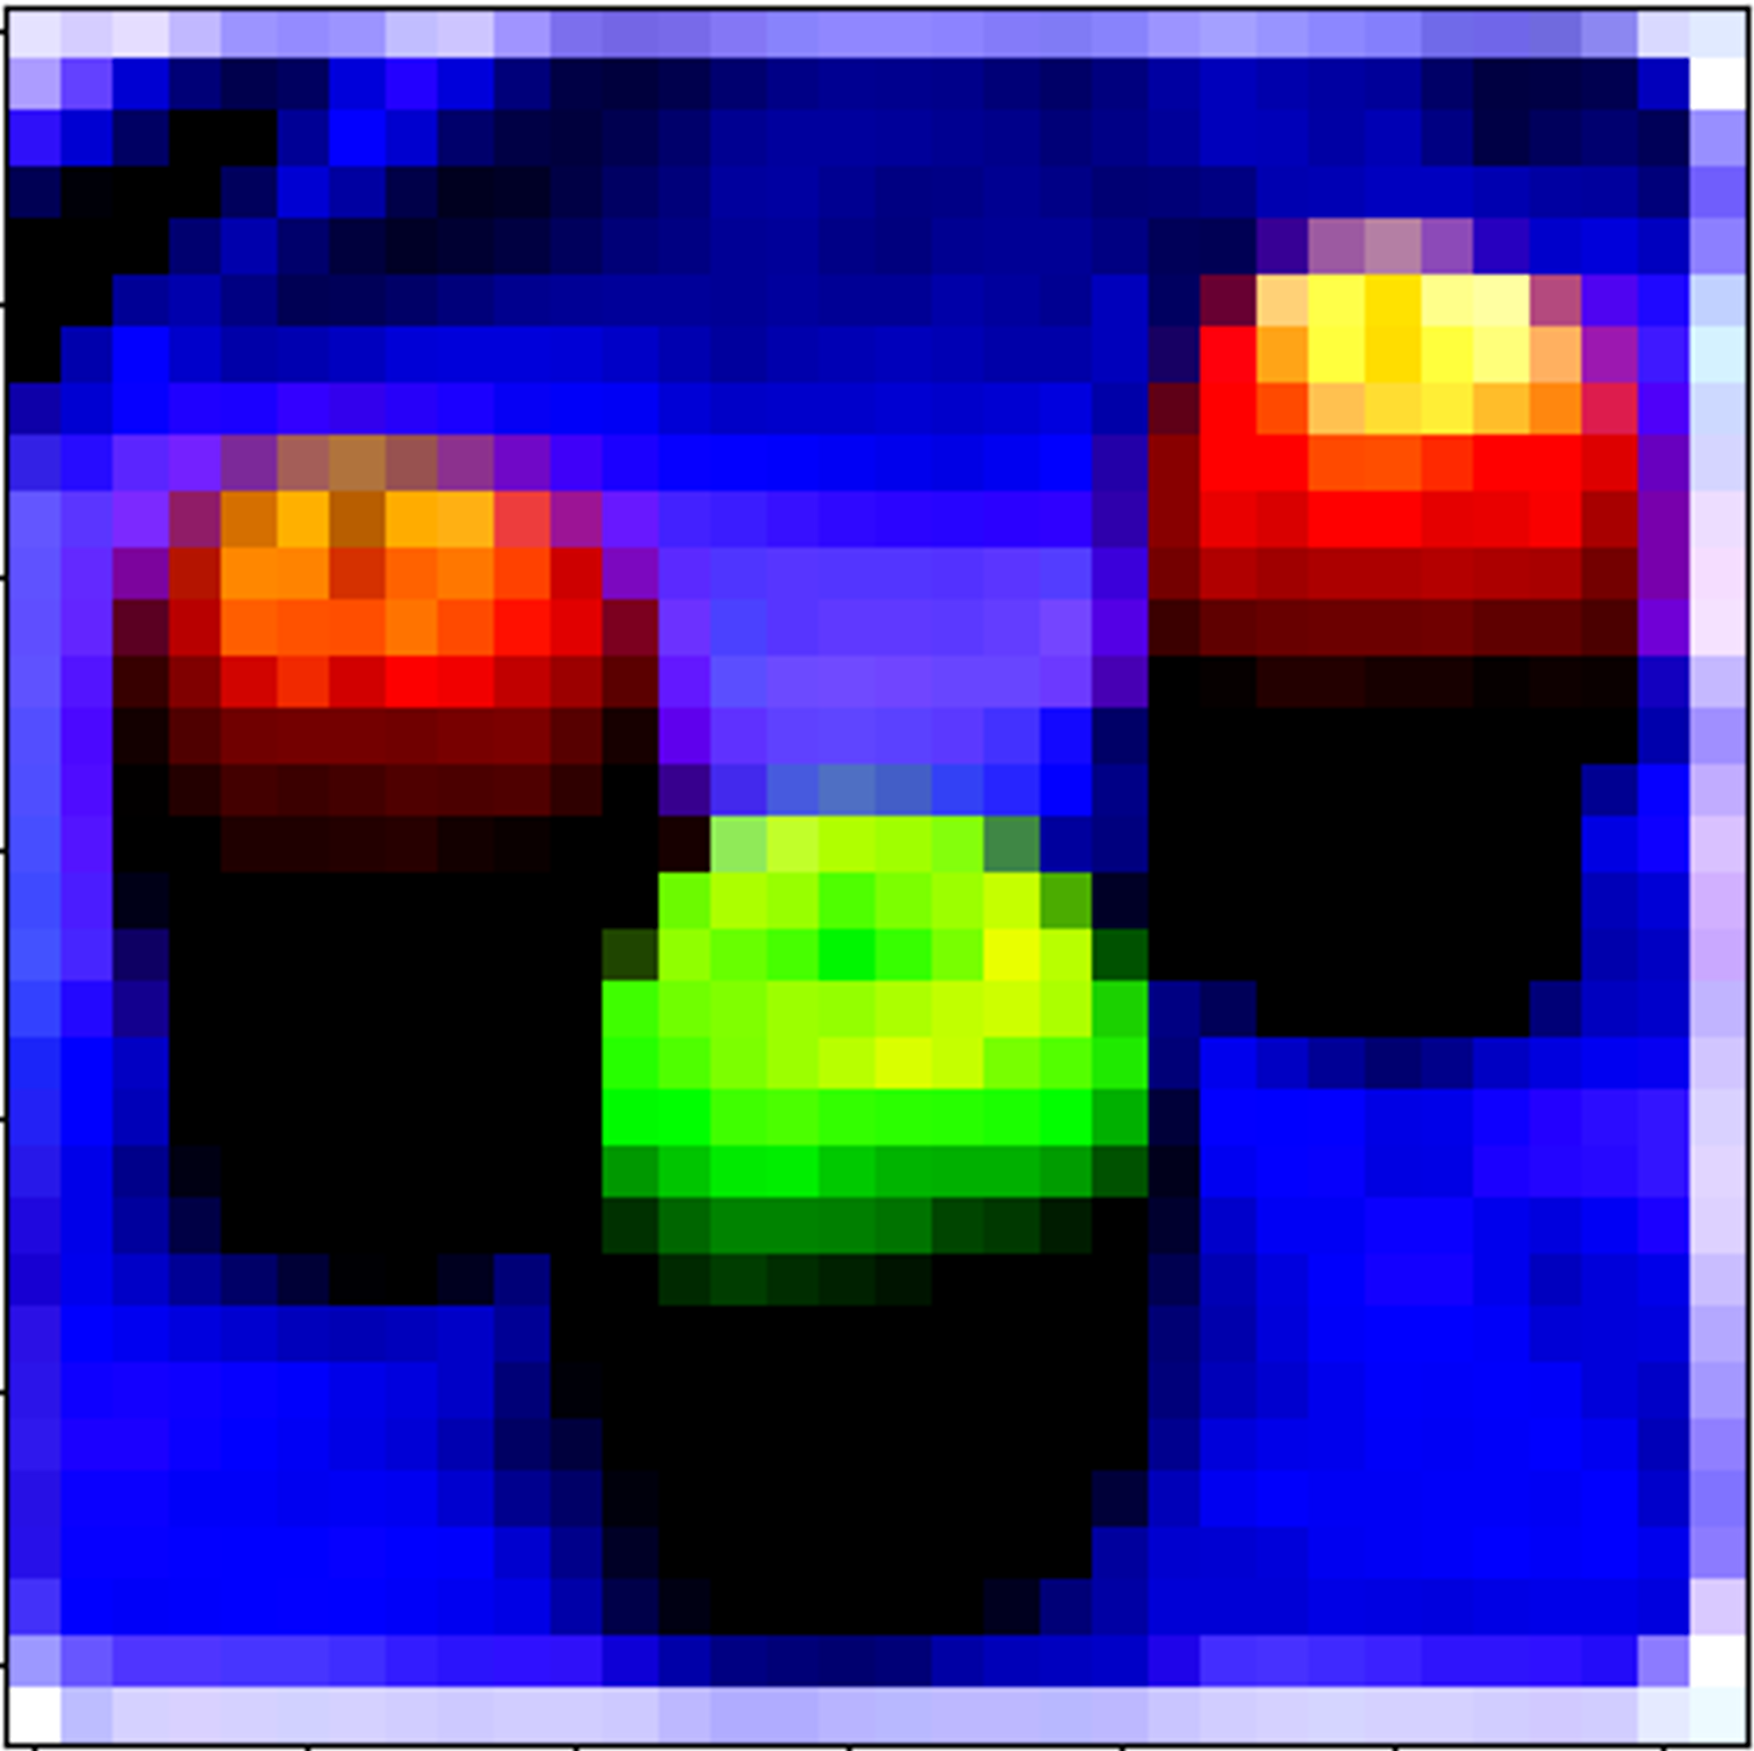}}&
\includegraphics[width=0.17\textwidth]{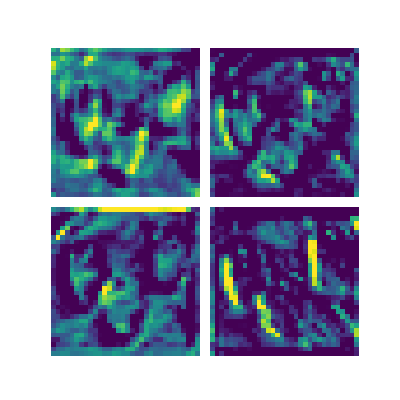} & \hspace{-0.3in}
\includegraphics[width=0.17\textwidth]{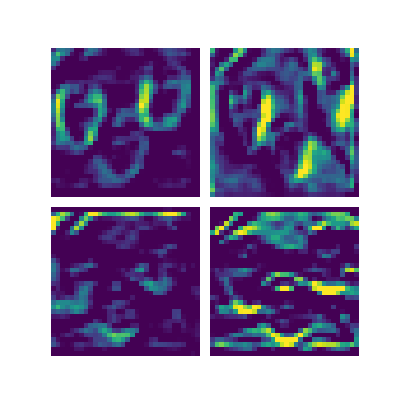} & \hspace{-0.3in}
\includegraphics[width=0.17\textwidth]{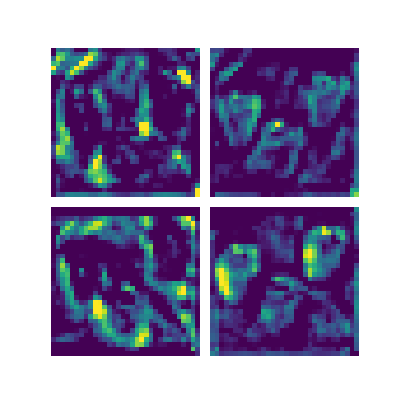} & \hspace{-0.3in}
\includegraphics[width=0.17\textwidth]{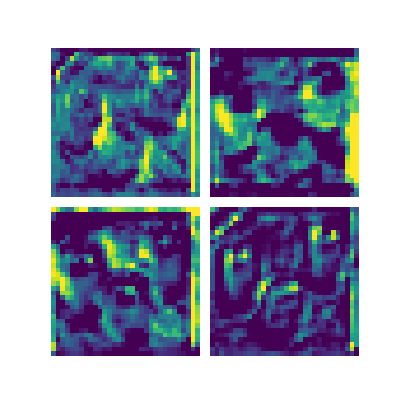} & \hspace{-0.2in}
\includegraphics[width=0.17\textwidth]{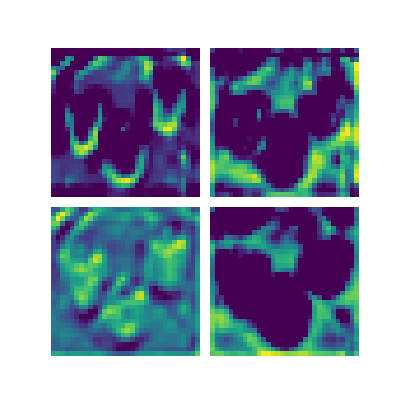} & \hspace{-0.3in}
\includegraphics[width=0.17\textwidth]{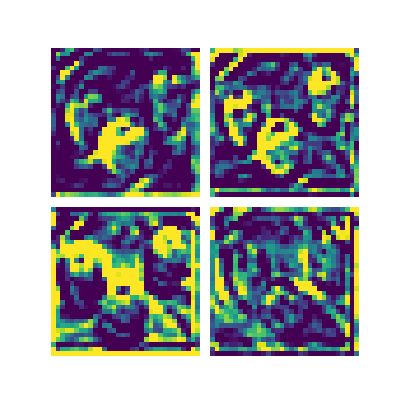} & \hspace{-0.3in}
\includegraphics[width=0.17\textwidth]{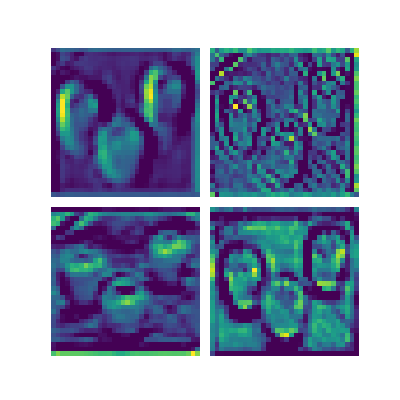} \vspace{-0.1in}\\
%\hspace{-0.2in} \specialcell{\textsc{Apple}\\$t=0$}& \textsc{Scl-Si} & \hspace{-0.3in} \textsc{Scl-Gss} & \hspace{-0.3in} \textsc{Scl-Der} & \hspace{-0.2in} \textsc{Ucl-Finetune} & \hspace{-0.3in} \textsc{Ucl-Si}& \hspace{-0.3in} \textsc{Lump (Ours)}\\
\hspace{-0.2in} \textsc{Apple} ($t_0$) & \specialcell{\textsc{Scl-Finetune}\\{\scriptsize Acc:$00.00\pm 0.00$}} & \hspace{-0.2in} \hspace{-0.2in} \specialcell{\textsc{Scl-Si}\\{\scriptsize Acc:$00.00\pm 0.00$}} & \hspace{-0.3in} \specialcell{\textsc{Scl-Gss}\\{\scriptsize Acc:$00.00\pm 0.00$}} & \hspace{-0.3in} \specialcell{\textsc{Scl-Der}\\{\scriptsize Acc:$00.00\pm 0.00$}} & \hspace{-0.2in} \specialcell{\textsc{Ucl-Finetune}\\{\scriptsize Acc:$00.00\pm 0.00$}} & \hspace{-0.3in} \specialcell{\textsc{Ucl-Si}\\{\scriptsize Acc:$00.00\pm 0.00$}}& \hspace{-0.3in} \specialcell{\textsc{Lump (Ours)}\\{\scriptsize Acc:$00.00\pm 0.00$}}\\
\end{tabular}}
\end{minipage}
\begin{minipage}[t]{1.05\linewidth}
\resizebox{\linewidth}{!}{%
\begin{tabular}{c cccc ccc}
\hspace{-0.2in}
\rb{\includegraphics[width=0.13\textwidth]{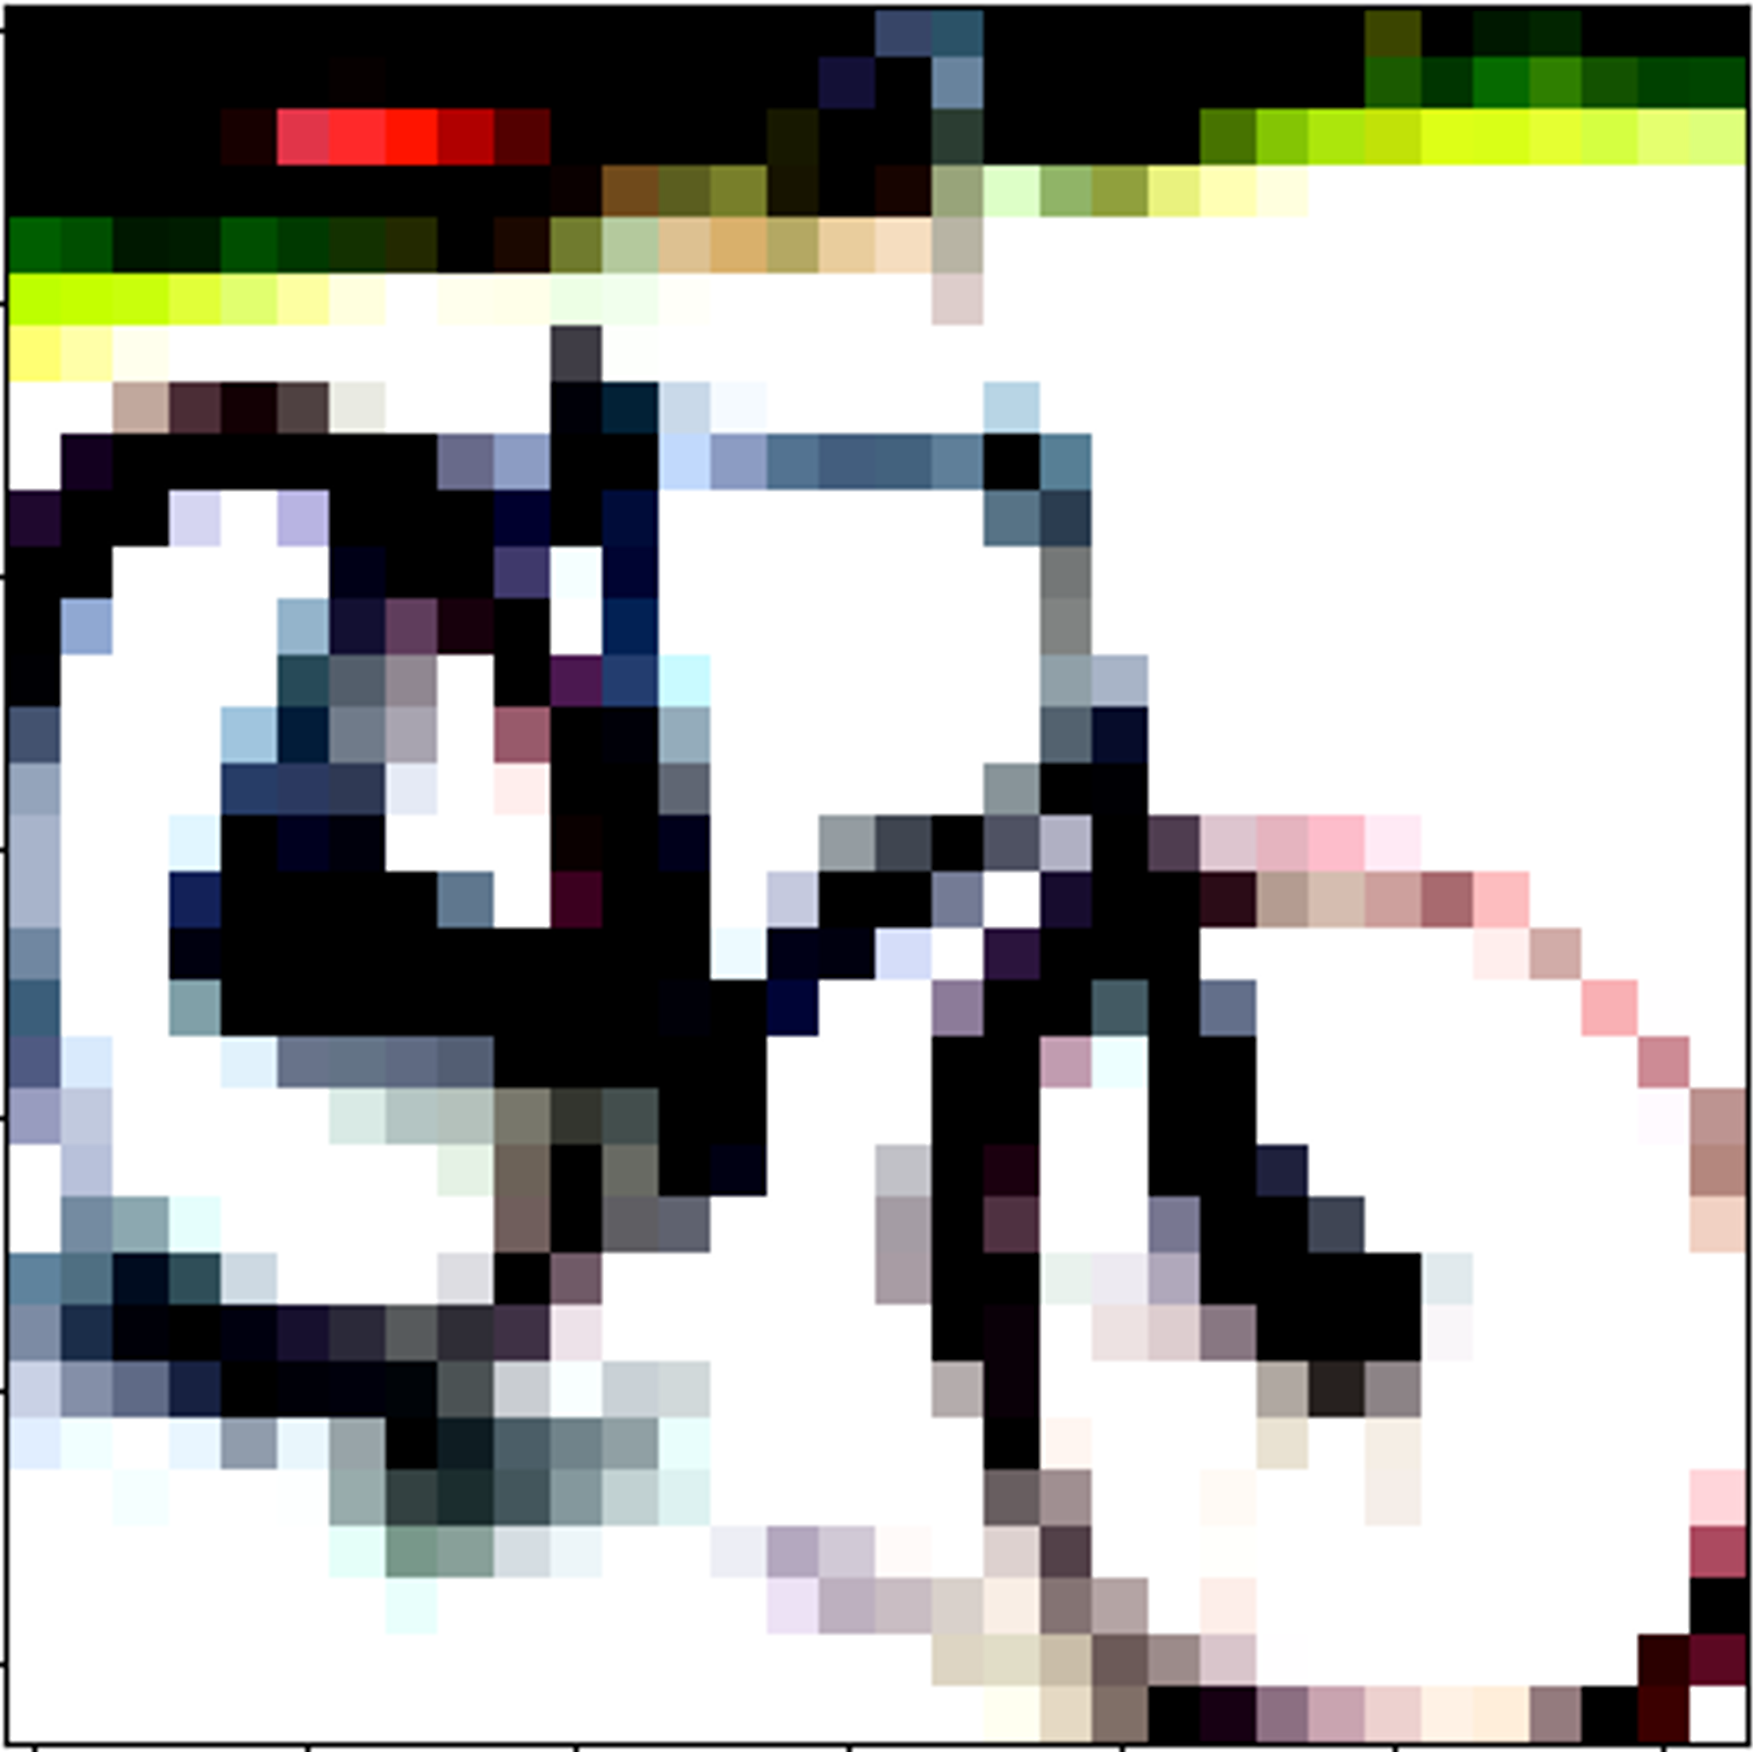}}&
\includegraphics[width=0.17\textwidth]{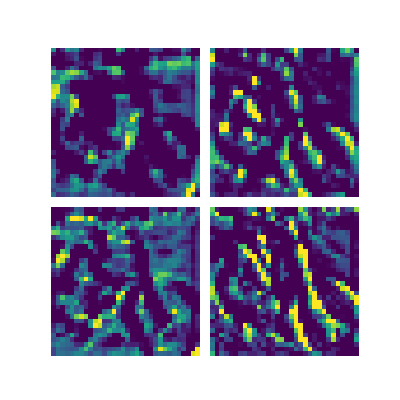} & \hspace{-0.3in}
\includegraphics[width=0.17\textwidth]{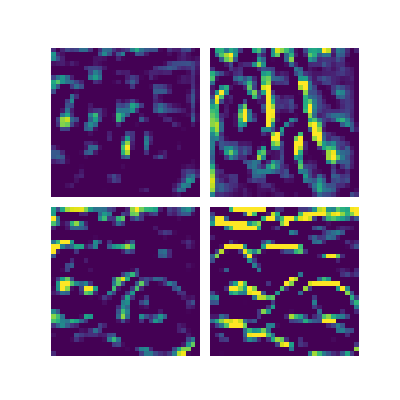} & \hspace{-0.3in}
\includegraphics[width=0.17\textwidth]{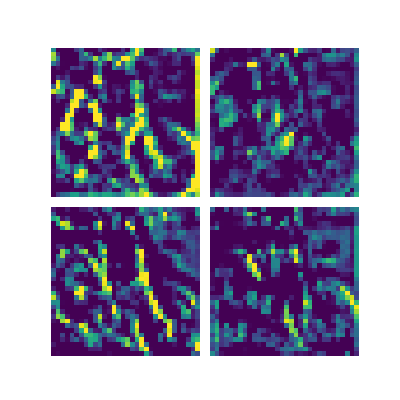} & \hspace{-0.3in}
\includegraphics[width=0.17\textwidth]{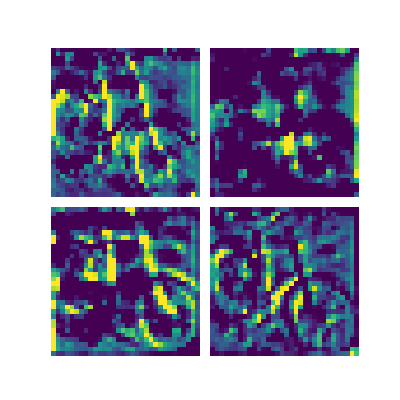} & \hspace{-0.2in}
\includegraphics[width=0.17\textwidth]{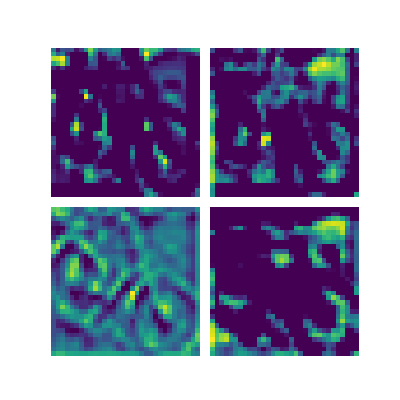} & \hspace{-0.3in}
\includegraphics[width=0.17\textwidth]{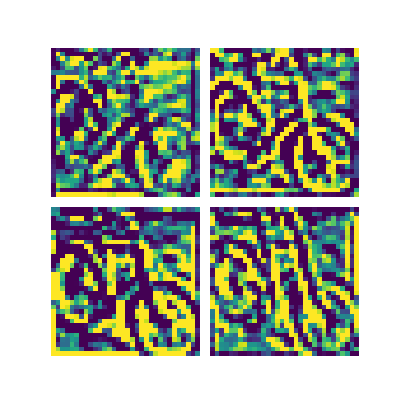} & \hspace{-0.3in}
\includegraphics[width=0.17\textwidth]{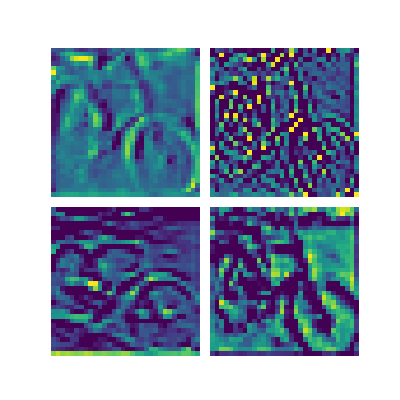} \vspace{-0.1in}\\
%\hspace{-0.2in} \specialcell{\textsc{Bicycle}\\$t=1$}& \textsc{Scl-Si} & \hspace{-0.3in} \textsc{Scl-Gss} & \hspace{-0.3in} \textsc{Scl-Der} & \hspace{-0.2in} \textsc{Ucl-Finetune} & \hspace{-0.3in} \textsc{Ucl-Si}& \hspace{-0.3in} \textsc{Lump (Ours)}\\
\hspace{-0.2in} \textsc{Bicycle} ($t_1$) & \specialcell{\textsc{Scl-Finetune}\\{\scriptsize Acc:$00.00\pm 0.00$}} & \hspace{-0.2in} \hspace{-0.2in} \specialcell{\textsc{Scl-Si}\\{\scriptsize Acc:$00.00\pm 0.00$}} & \hspace{-0.3in} \specialcell{\textsc{Scl-Gss}\\{\scriptsize Acc:$00.00\pm 0.00$}} & \hspace{-0.3in} \specialcell{\textsc{Scl-Der}\\{\scriptsize Acc:$00.00\pm 0.00$}} & \hspace{-0.2in} \specialcell{\textsc{Ucl-Finetune}\\{\scriptsize Acc:$00.00\pm 0.00$}} & \hspace{-0.3in} \specialcell{\textsc{Ucl-Si}\\{\scriptsize Acc:$00.00\pm 0.00$}}& \hspace{-0.3in} \specialcell{\textsc{Lump (Ours)}\\{\scriptsize Acc:$00.00\pm 0.00$}}\\
\end{tabular}}
\end{minipage}
\begin{minipage}[t]{1.05\linewidth}
\resizebox{\linewidth}{!}{%
\begin{tabular}{c cccc ccc}
\hspace{-0.2in}
\rb{\includegraphics[width=0.13\textwidth]{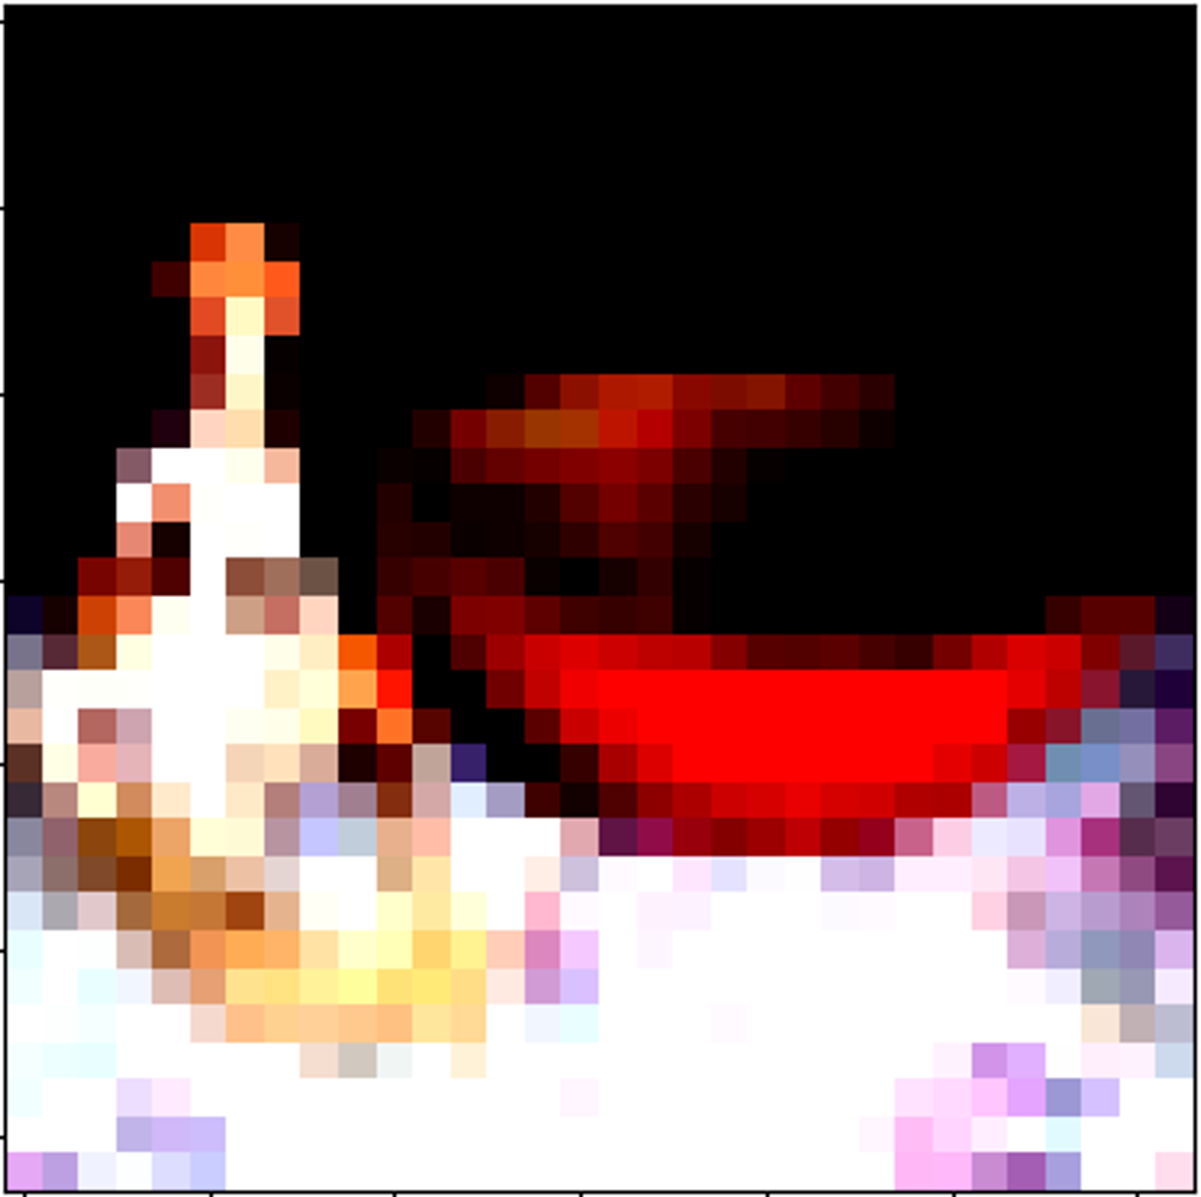}}&
\includegraphics[width=0.17\textwidth]{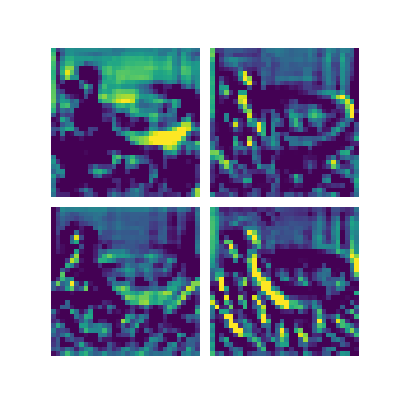} & \hspace{-0.3in}
\includegraphics[width=0.17\textwidth]{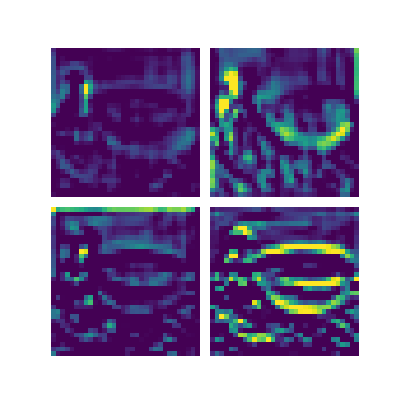} & \hspace{-0.3in}
\includegraphics[width=0.17\textwidth]{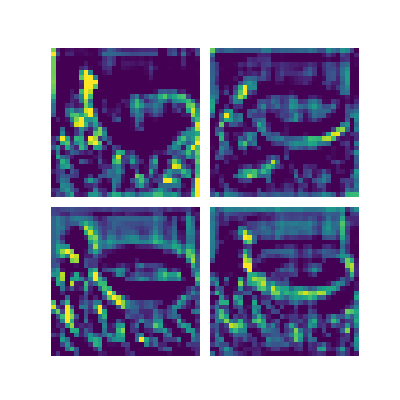} & \hspace{-0.3in}
\includegraphics[width=0.17\textwidth]{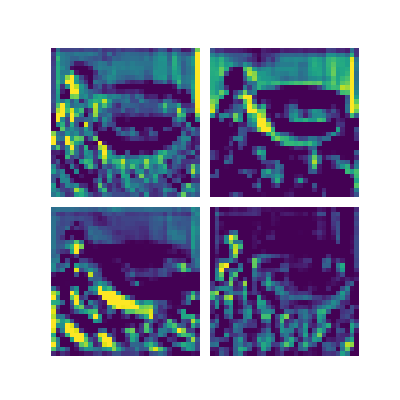} & \hspace{-0.2in}
\includegraphics[width=0.17\textwidth]{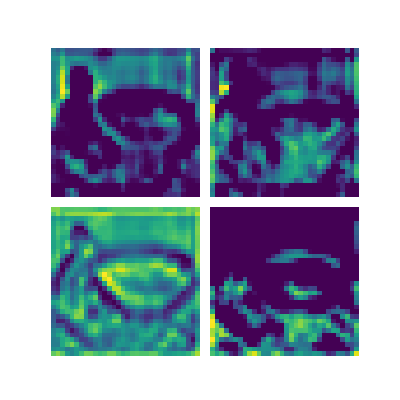} & \hspace{-0.3in}
\includegraphics[width=0.17\textwidth]{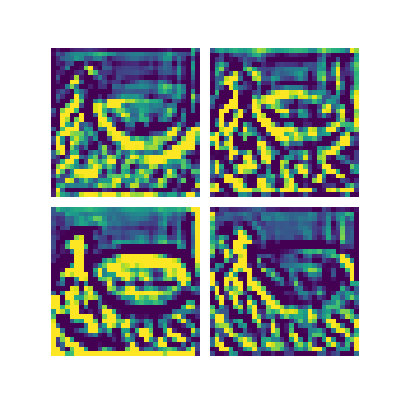} & \hspace{-0.3in}
\includegraphics[width=0.17\textwidth]{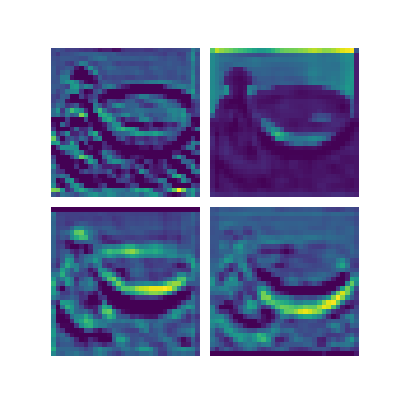} \vspace{-0.1in}\\
%\hspace{-0.2in} \specialcell{\textsc{Bowl}\\$t=2$}& \textsc{Scl-Si} & \hspace{-0.3in} \textsc{Scl-Gss} & \hspace{-0.3in} \textsc{Scl-Der} & \hspace{-0.2in} \textsc{Ucl-Finetune} & \hspace{-0.3in} \textsc{Ucl-Si}& \hspace{-0.3in} \textsc{Lump (Ours)}\\
\hspace{-0.2in} \textsc{Bowl} ($t_2$) & \specialcell{\textsc{Scl-Finetune}\\{\scriptsize Acc:$00.00\pm 0.00$}} & \hspace{-0.2in} \hspace{-0.2in} \specialcell{\textsc{Scl-Si}\\{\scriptsize Acc:$00.00\pm 0.00$}} & \hspace{-0.3in} \specialcell{\textsc{Scl-Gss}\\{\scriptsize Acc:$00.00\pm 0.00$}} & \hspace{-0.3in} \specialcell{\textsc{Scl-Der}\\{\scriptsize Acc:$00.00\pm 0.00$}} & \hspace{-0.2in} \specialcell{\textsc{Ucl-Finetune}\\{\scriptsize Acc:$00.00\pm 0.00$}} & \hspace{-0.3in} \specialcell{\textsc{Ucl-Si}\\{\scriptsize Acc:$00.00\pm 0.00$}}& \hspace{-0.3in} \specialcell{\textsc{Lump (Ours)}\\{\scriptsize Acc:$00.00\pm 0.00$}}\\
\end{tabular}}
\end{minipage}
\begin{minipage}[t]{1.05\linewidth}
\resizebox{\linewidth}{!}{%
\begin{tabular}{c cccc ccc}
\hspace{-0.2in}
\rb{\includegraphics[width=0.13\textwidth]{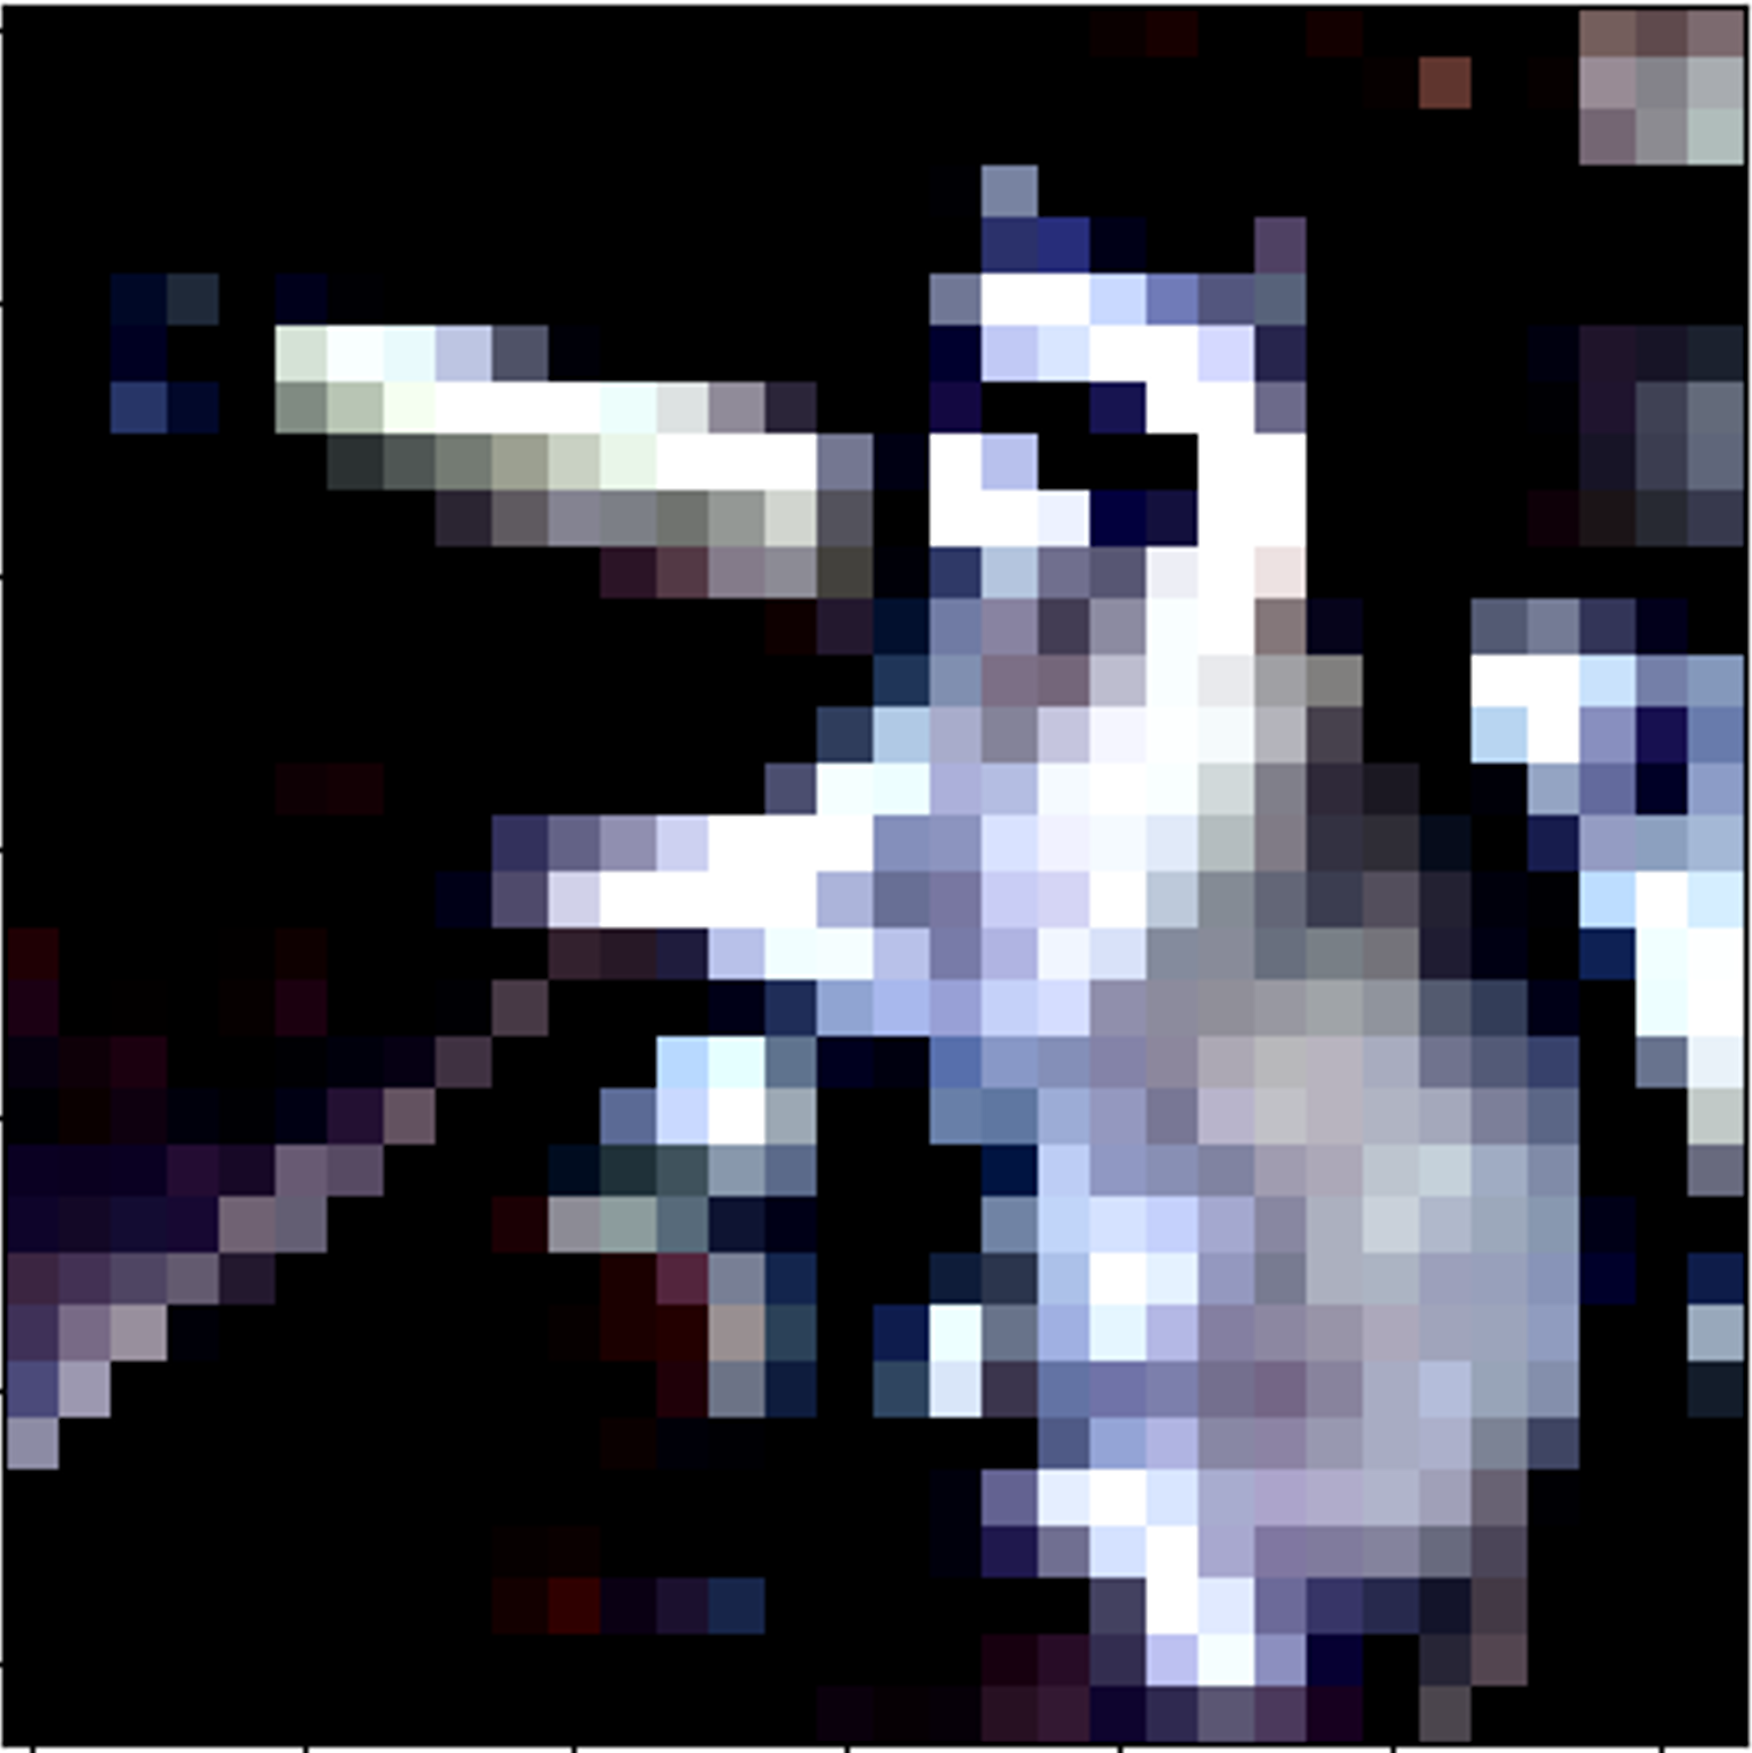}}&
\includegraphics[width=0.17\textwidth]{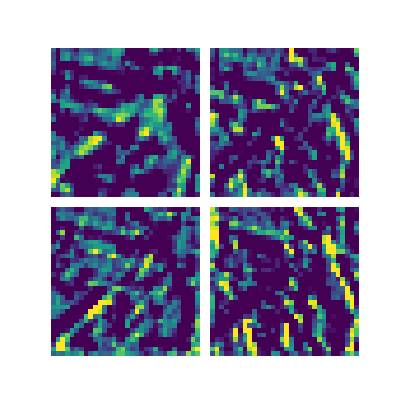} & \hspace{-0.3in}
\includegraphics[width=0.17\textwidth]{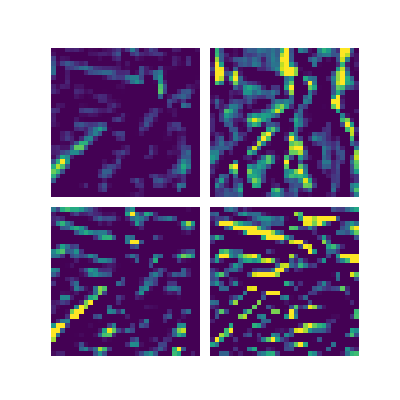} & \hspace{-0.3in}
\includegraphics[width=0.17\textwidth]{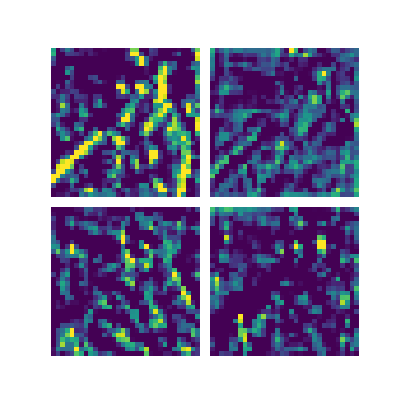} & \hspace{-0.3in}
\includegraphics[width=0.17\textwidth]{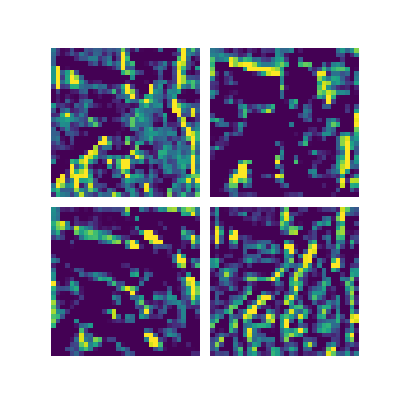} & \hspace{-0.2in}
\includegraphics[width=0.17\textwidth]{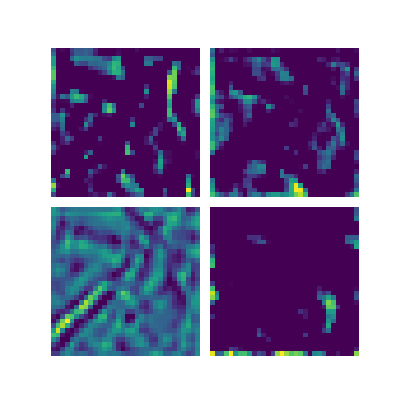} & \hspace{-0.3in}
\includegraphics[width=0.17\textwidth]{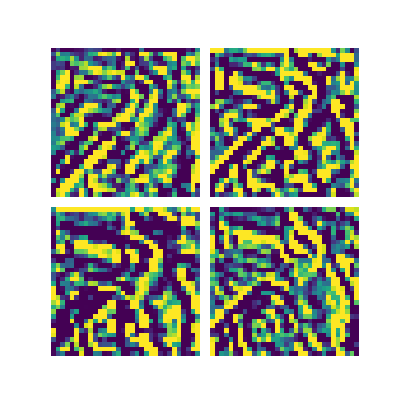} & \hspace{-0.3in}
\includegraphics[width=0.17\textwidth]{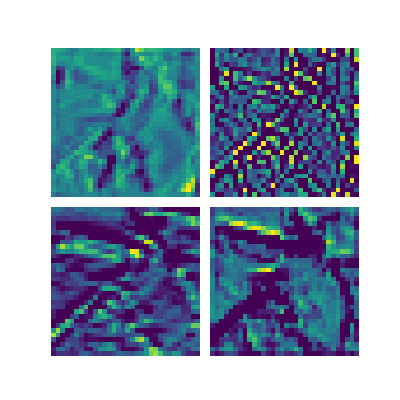} \vspace{-0.1in}\\
%\hspace{-0.2in} \specialcell{\textsc{Raccoon}\\{$t=13$}}& \textsc{Scl-Si} & \hspace{-0.3in} \textsc{Scl-Gss} & \hspace{-0.3in} \textsc{Scl-Der} & \hspace{-0.2in} \textsc{Ucl-Finetune} & \hspace{-0.3in} \textsc{Ucl-Si}& \hspace{-0.3in} \textsc{Lump (Ours)}\\
\hspace{-0.2in} {\scriptsize \textsc{Raccoon} ($t_{13}$)} & \specialcell{\textsc{Scl-Finetune}\\{\scriptsize Acc:$00.00\pm 0.00$}} & \hspace{-0.2in} \hspace{-0.2in} \specialcell{\textsc{Scl-Si}\\{\scriptsize Acc:$00.00\pm 0.00$}} & \hspace{-0.3in} \specialcell{\textsc{Scl-Gss}\\{\scriptsize Acc:$00.00\pm 0.00$}} & \hspace{-0.3in} \specialcell{\textsc{Scl-Der}\\{\scriptsize Acc:$00.00\pm 0.00$}} & \hspace{-0.2in} \specialcell{\textsc{Ucl-Finetune}\\{\scriptsize Acc:$00.00\pm 0.00$}} & \hspace{-0.3in} \specialcell{\textsc{Ucl-Si}\\{\scriptsize Acc:$00.00\pm 0.00$}}& \hspace{-0.3in} \specialcell{\textsc{Lump (Ours)}\\{\scriptsize Acc:$00.00\pm 0.00$}}\\
\end{tabular}}
\captionof{figure}{second block feature map visualization after the completion of continual learning for CIFAR-100 ($n=20$).}
\vspace{-0.15in}
\end{minipage}
\label{fig:visualize}
\end{figure*}
