# Supplementary material for: Representational Continuity for Unsupervised Continual Learning
Source: arXiv:2110.06976 source file (2022-04-05)
Supplement: Supplementary file 4 [file 7_appendix_figure_2.tex]

\begin{figure*}[t!]
\begin{minipage}[t]{1.05\linewidth}
\resizebox{\linewidth}{!}{%
\begin{tabular}{cccccc}
\small
\hspace{-0.15in}\rowlegend{~~~~$t=0$}
    \includegraphics[width=0.16\textwidth]{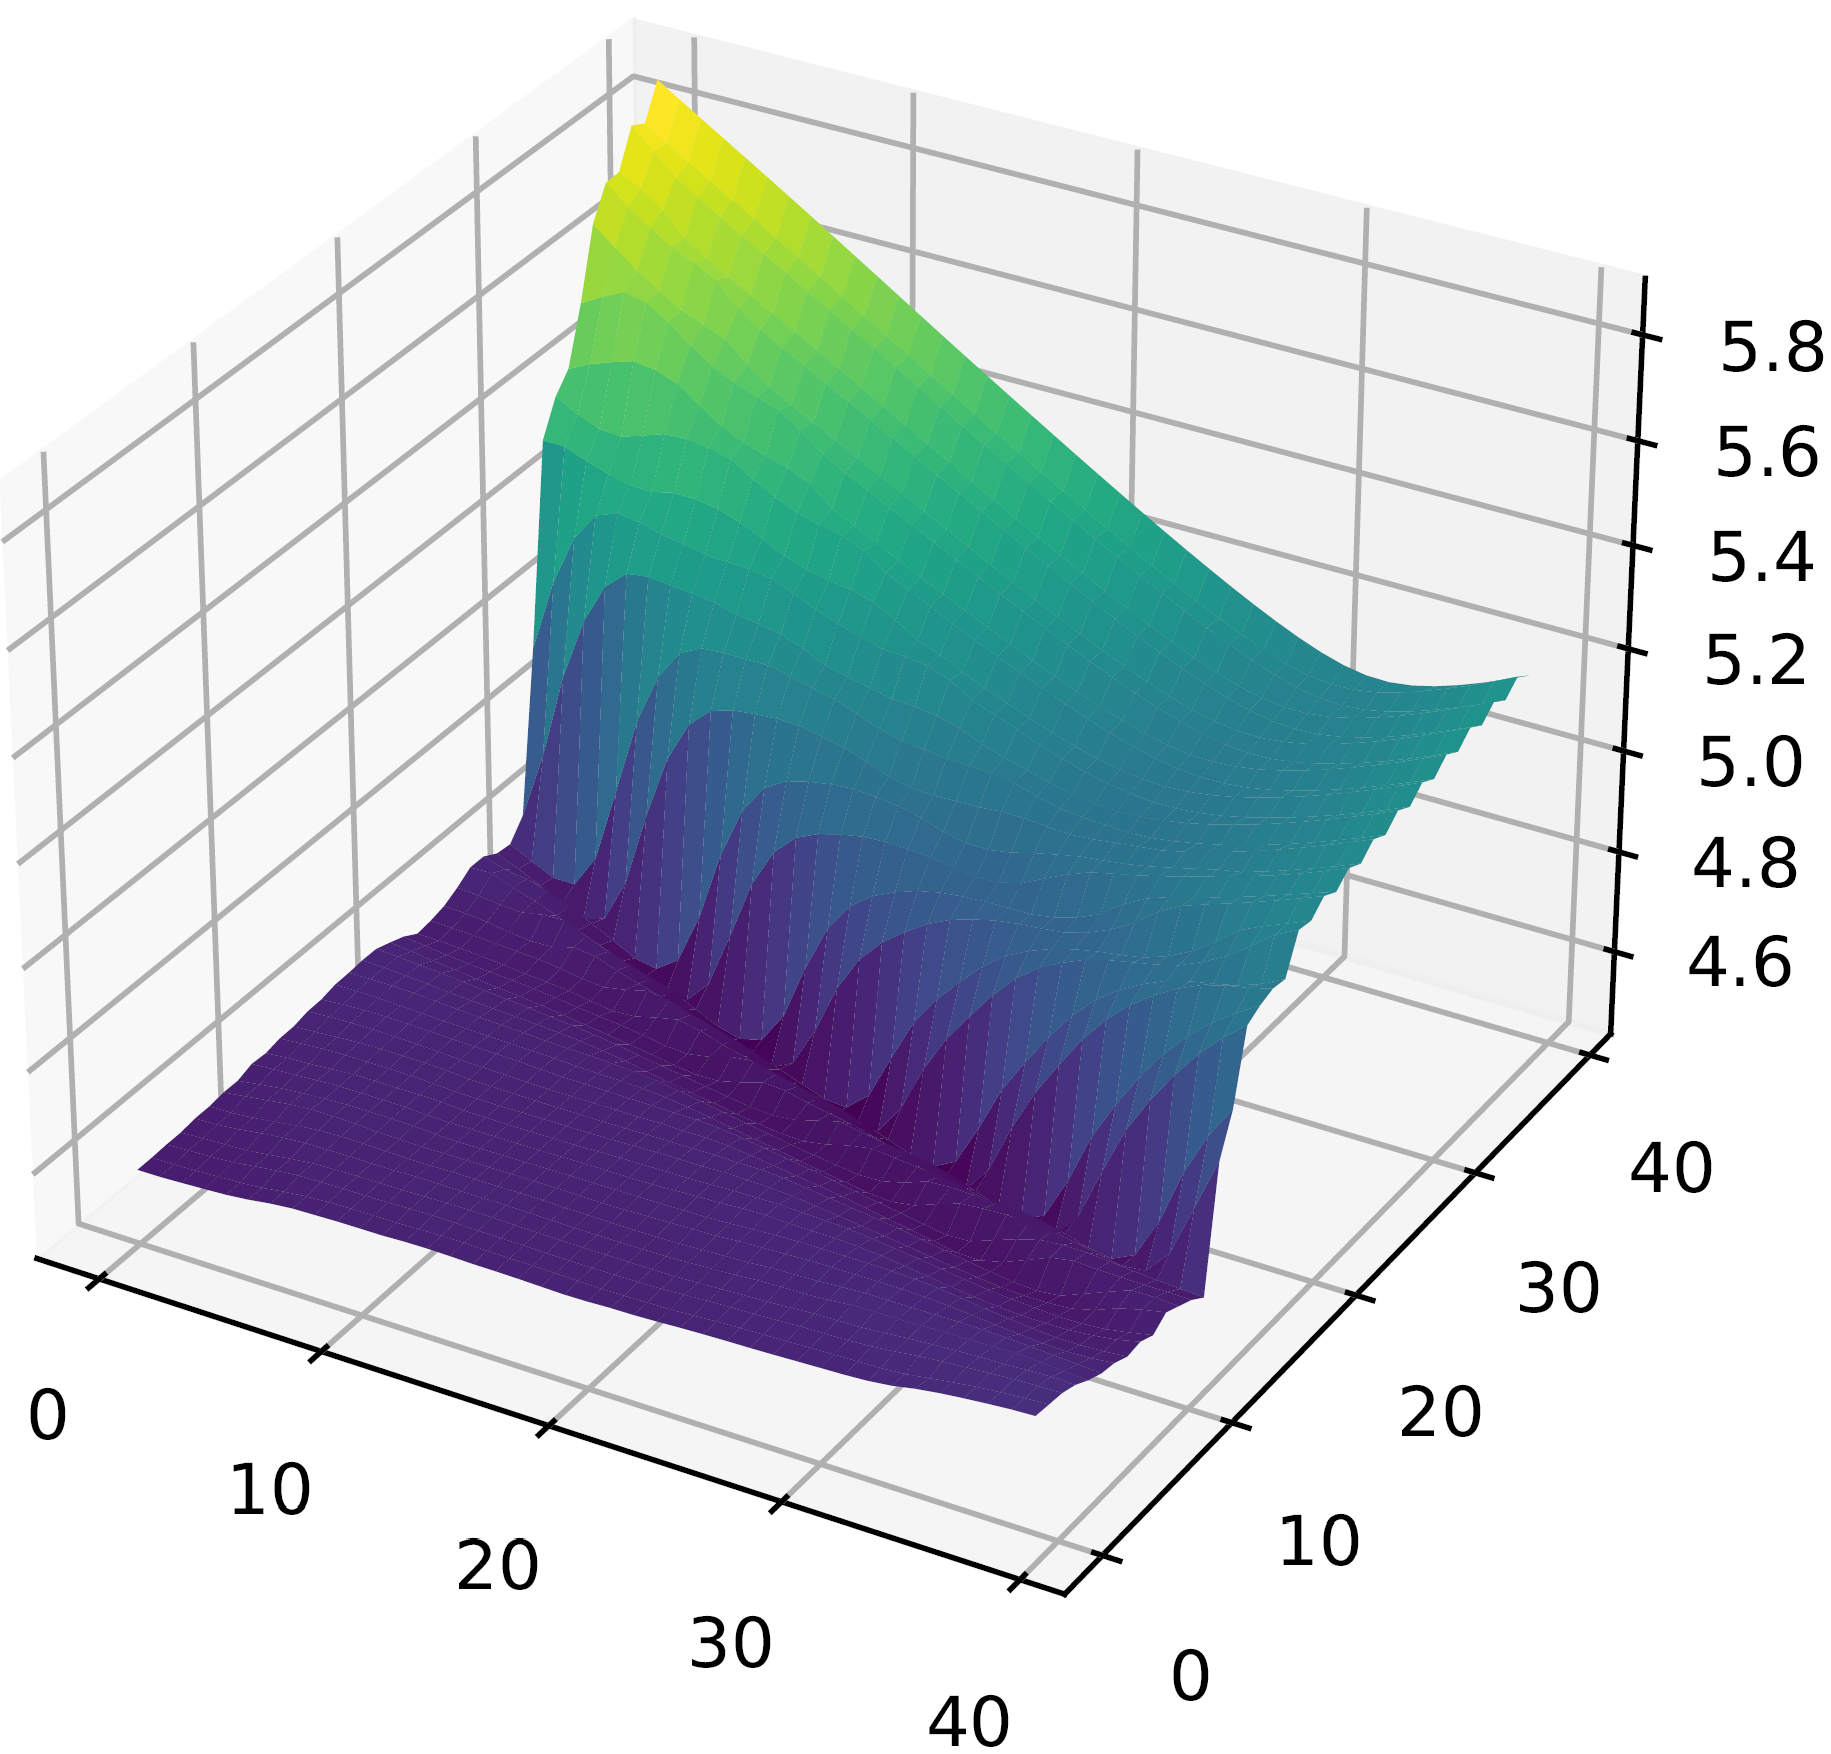} & \hspace{-0.15in}
    \includegraphics[width=0.16\textwidth]{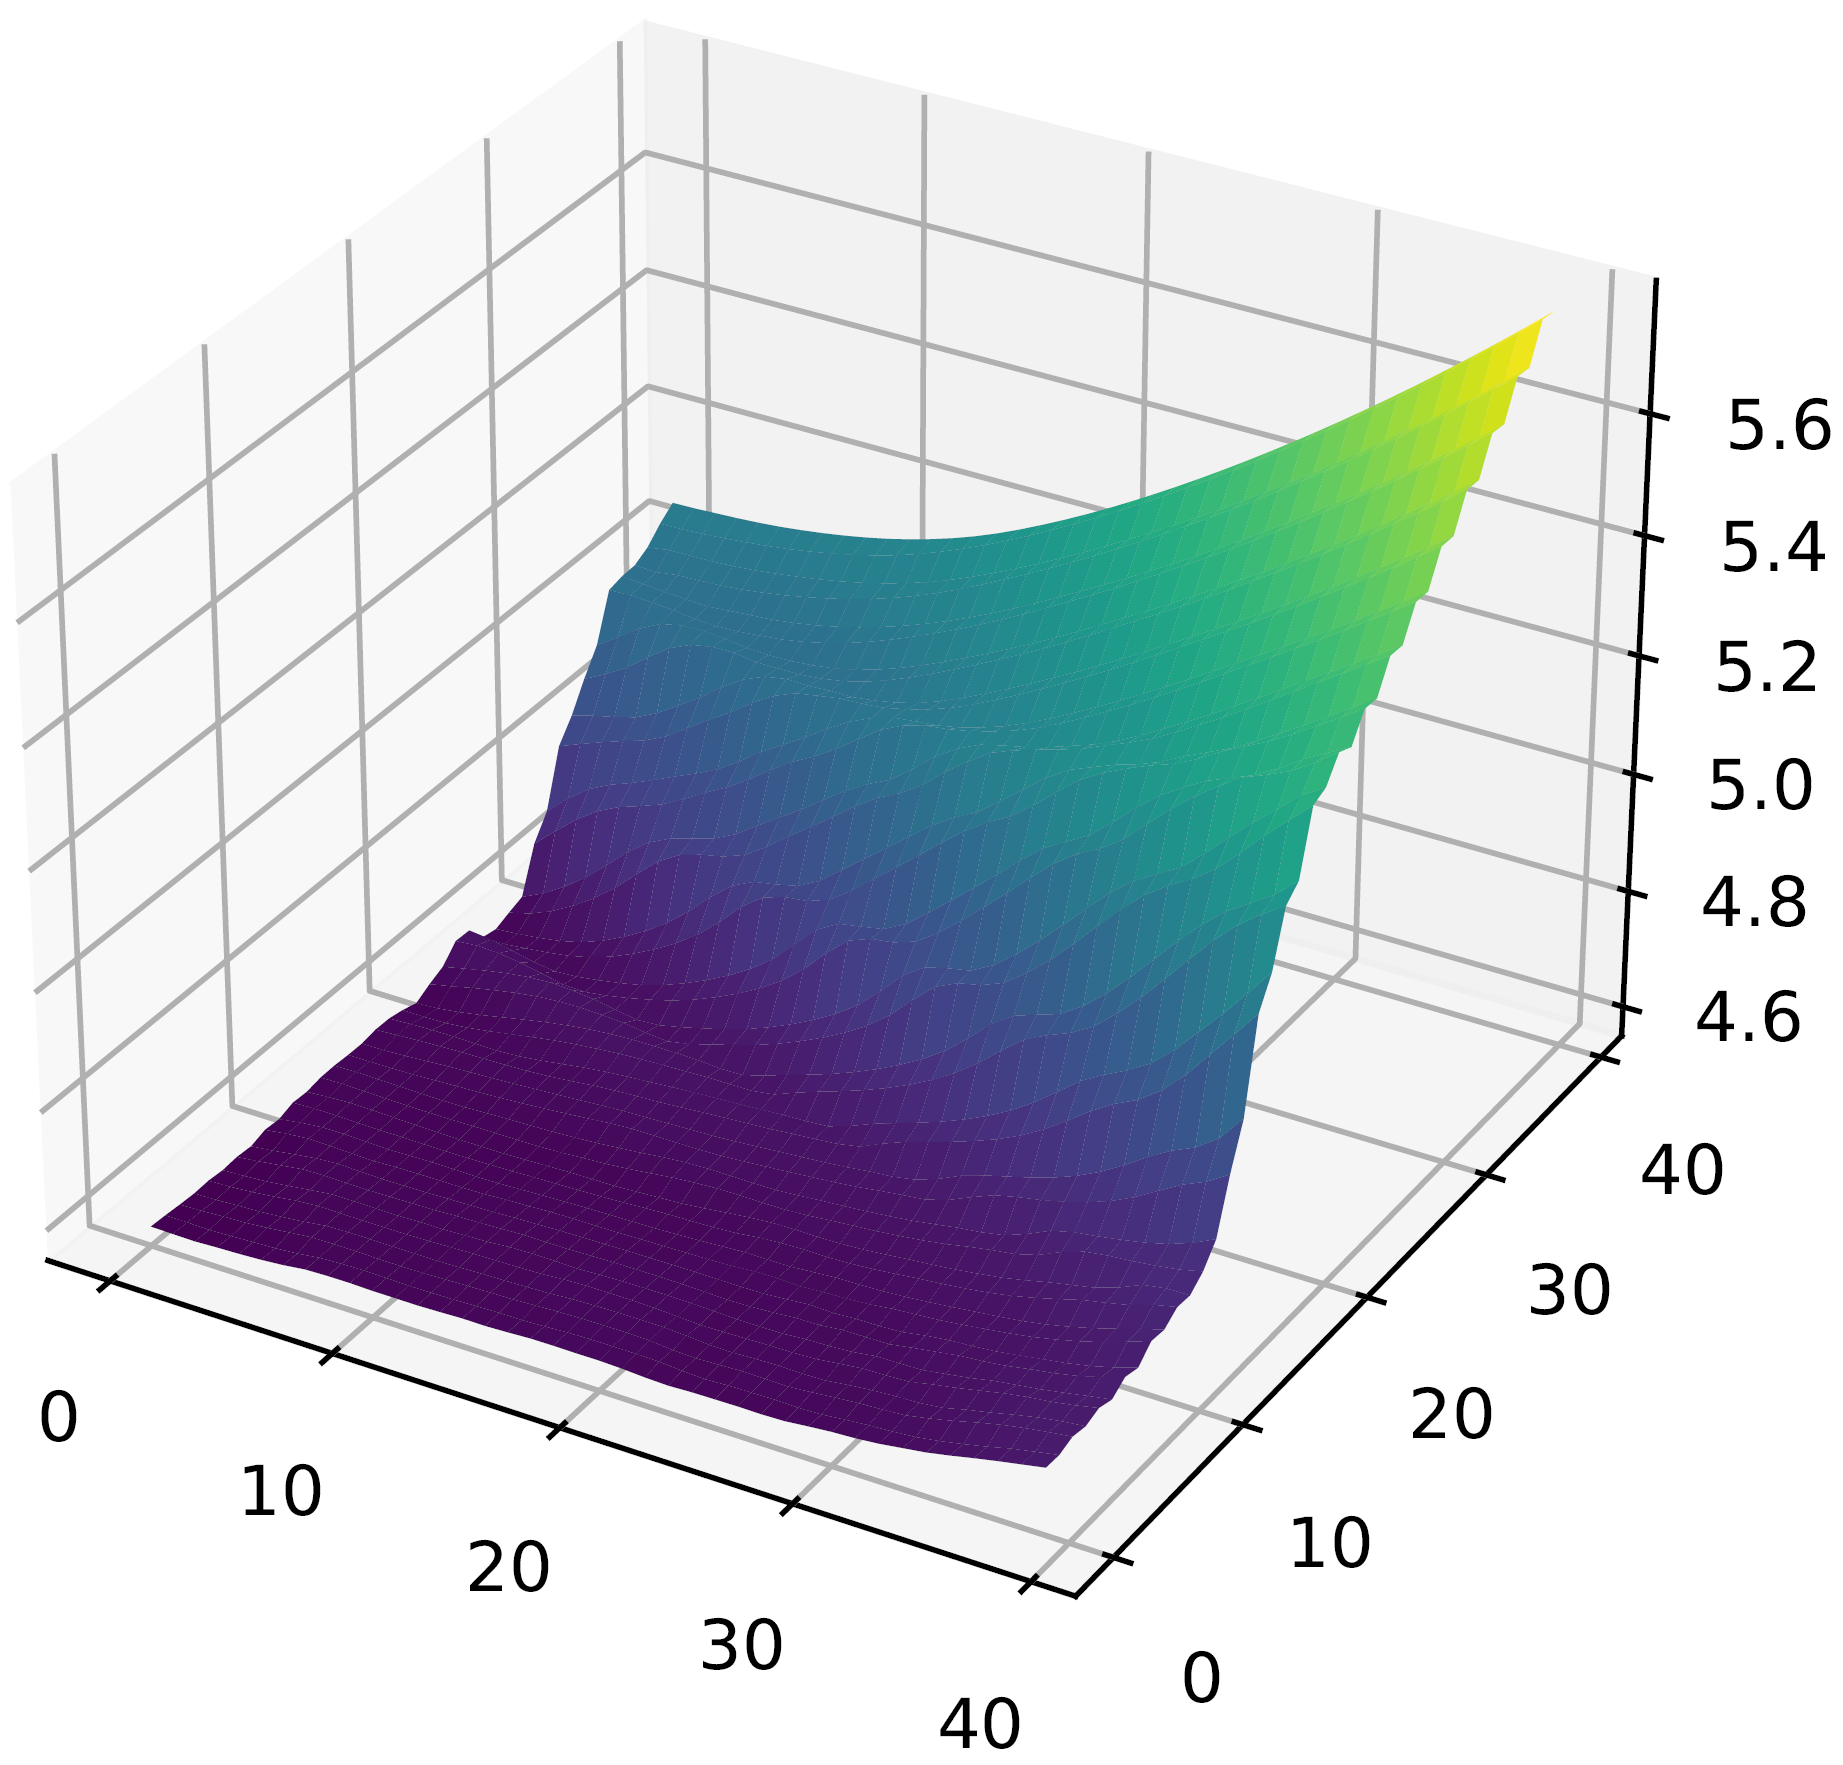} & \hspace{-0.15in}
    \includegraphics[width=0.16\textwidth]{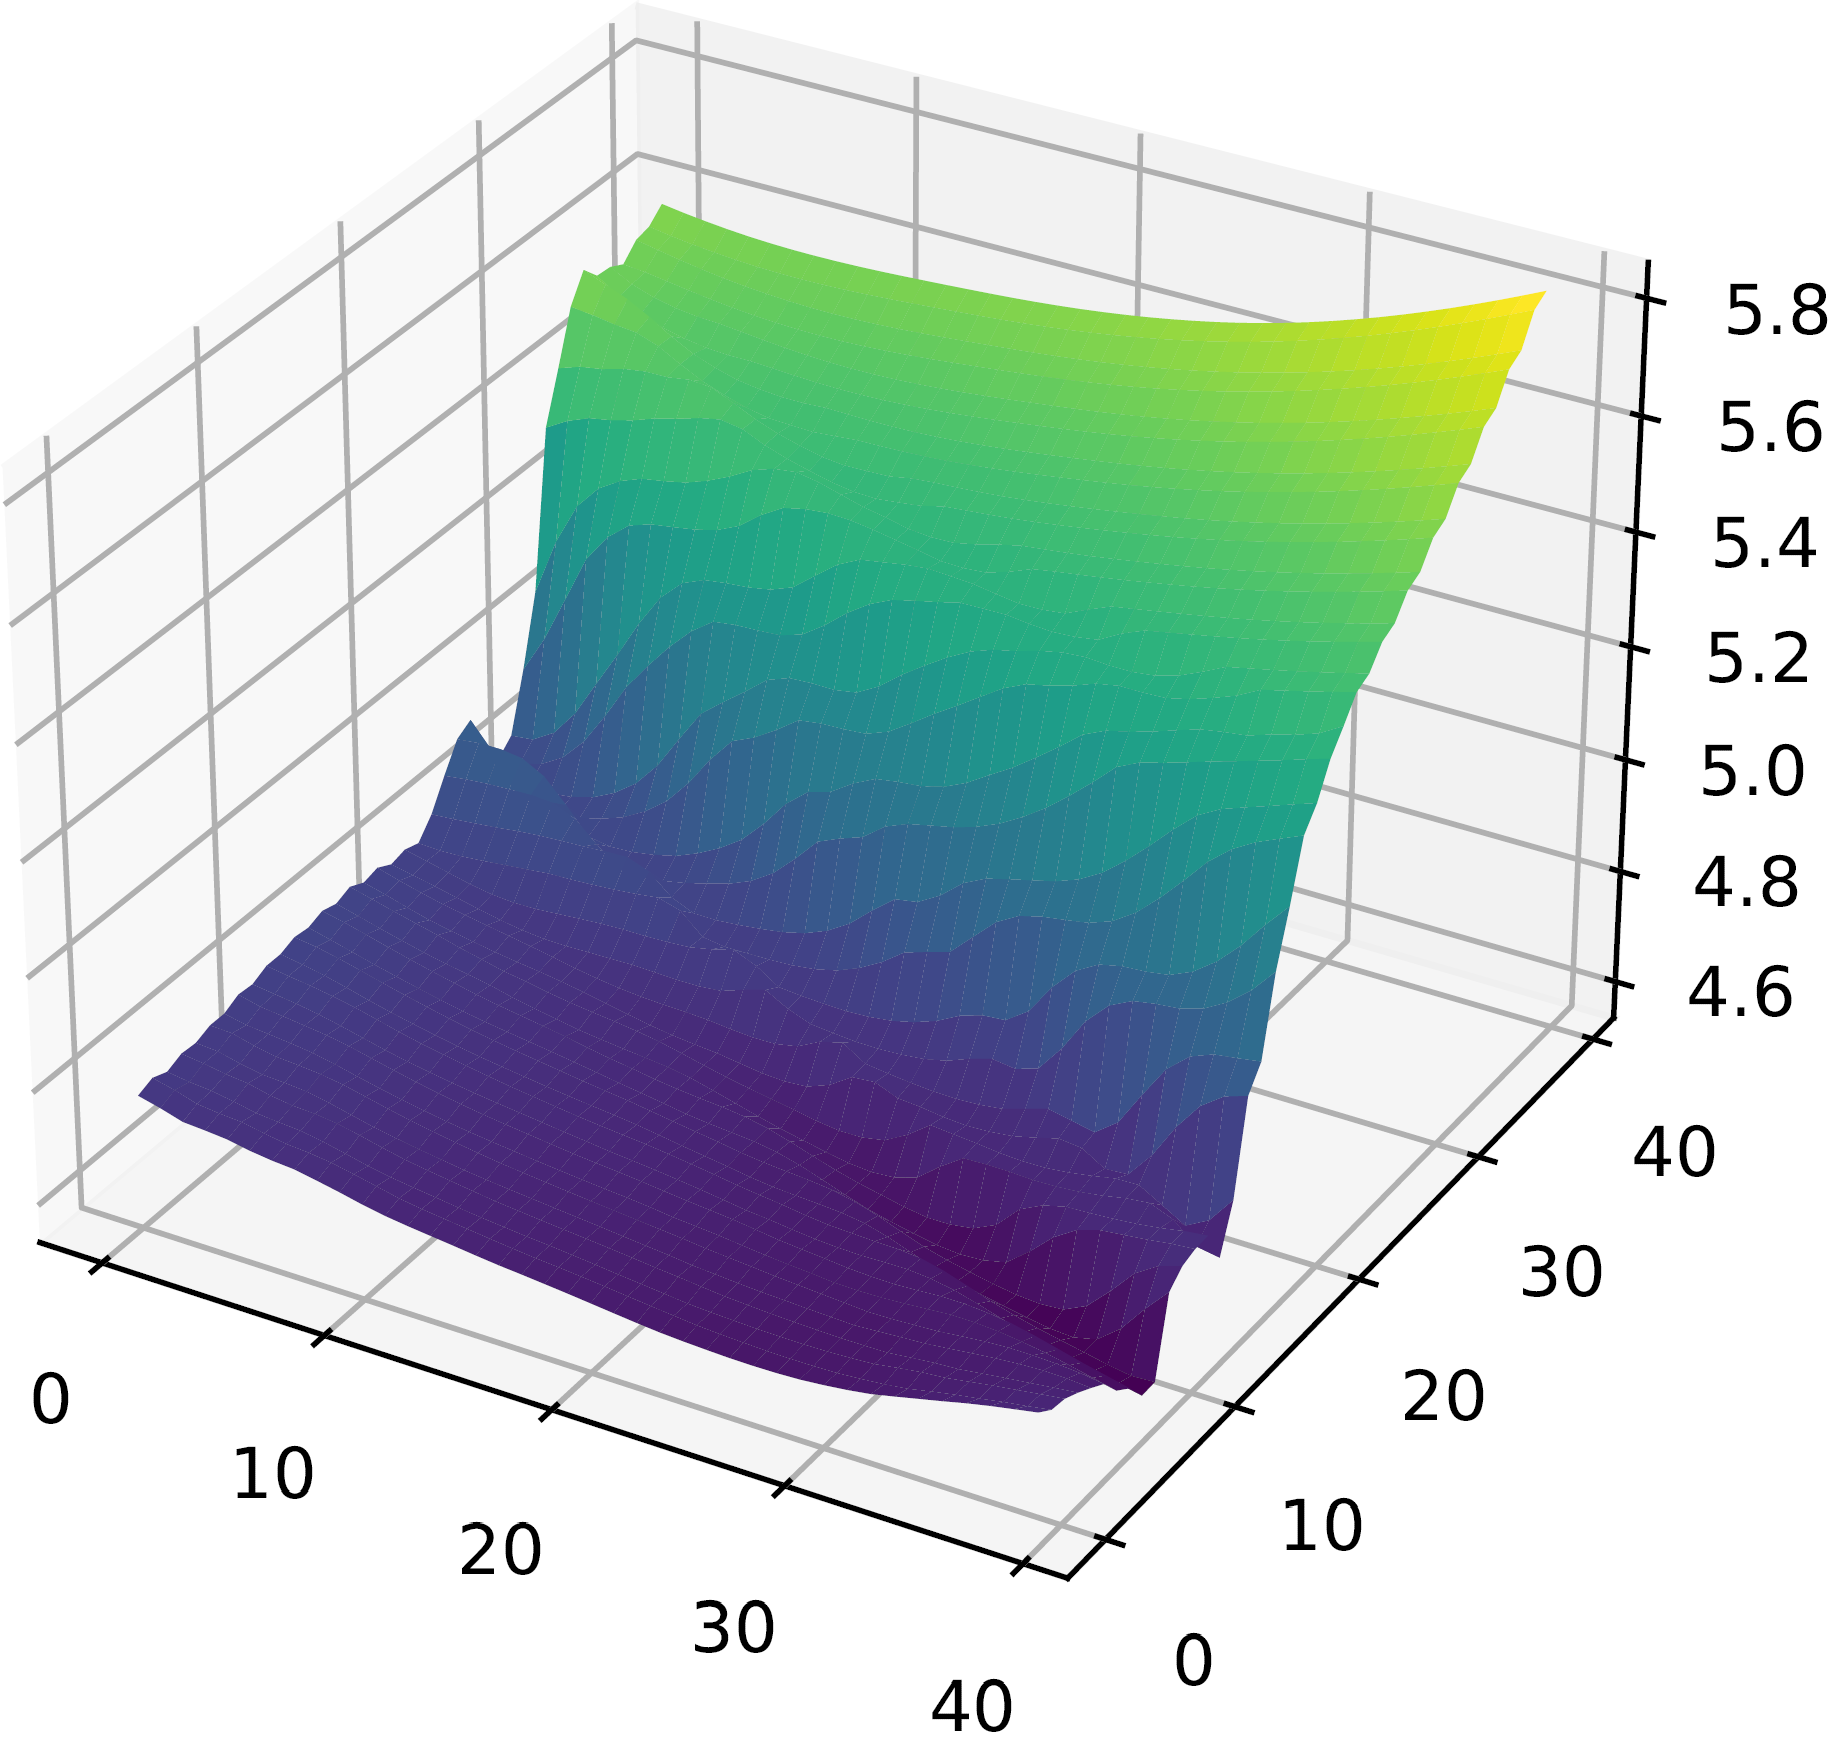} & \hspace{-0.15in}
    \includegraphics[width=0.16\textwidth]{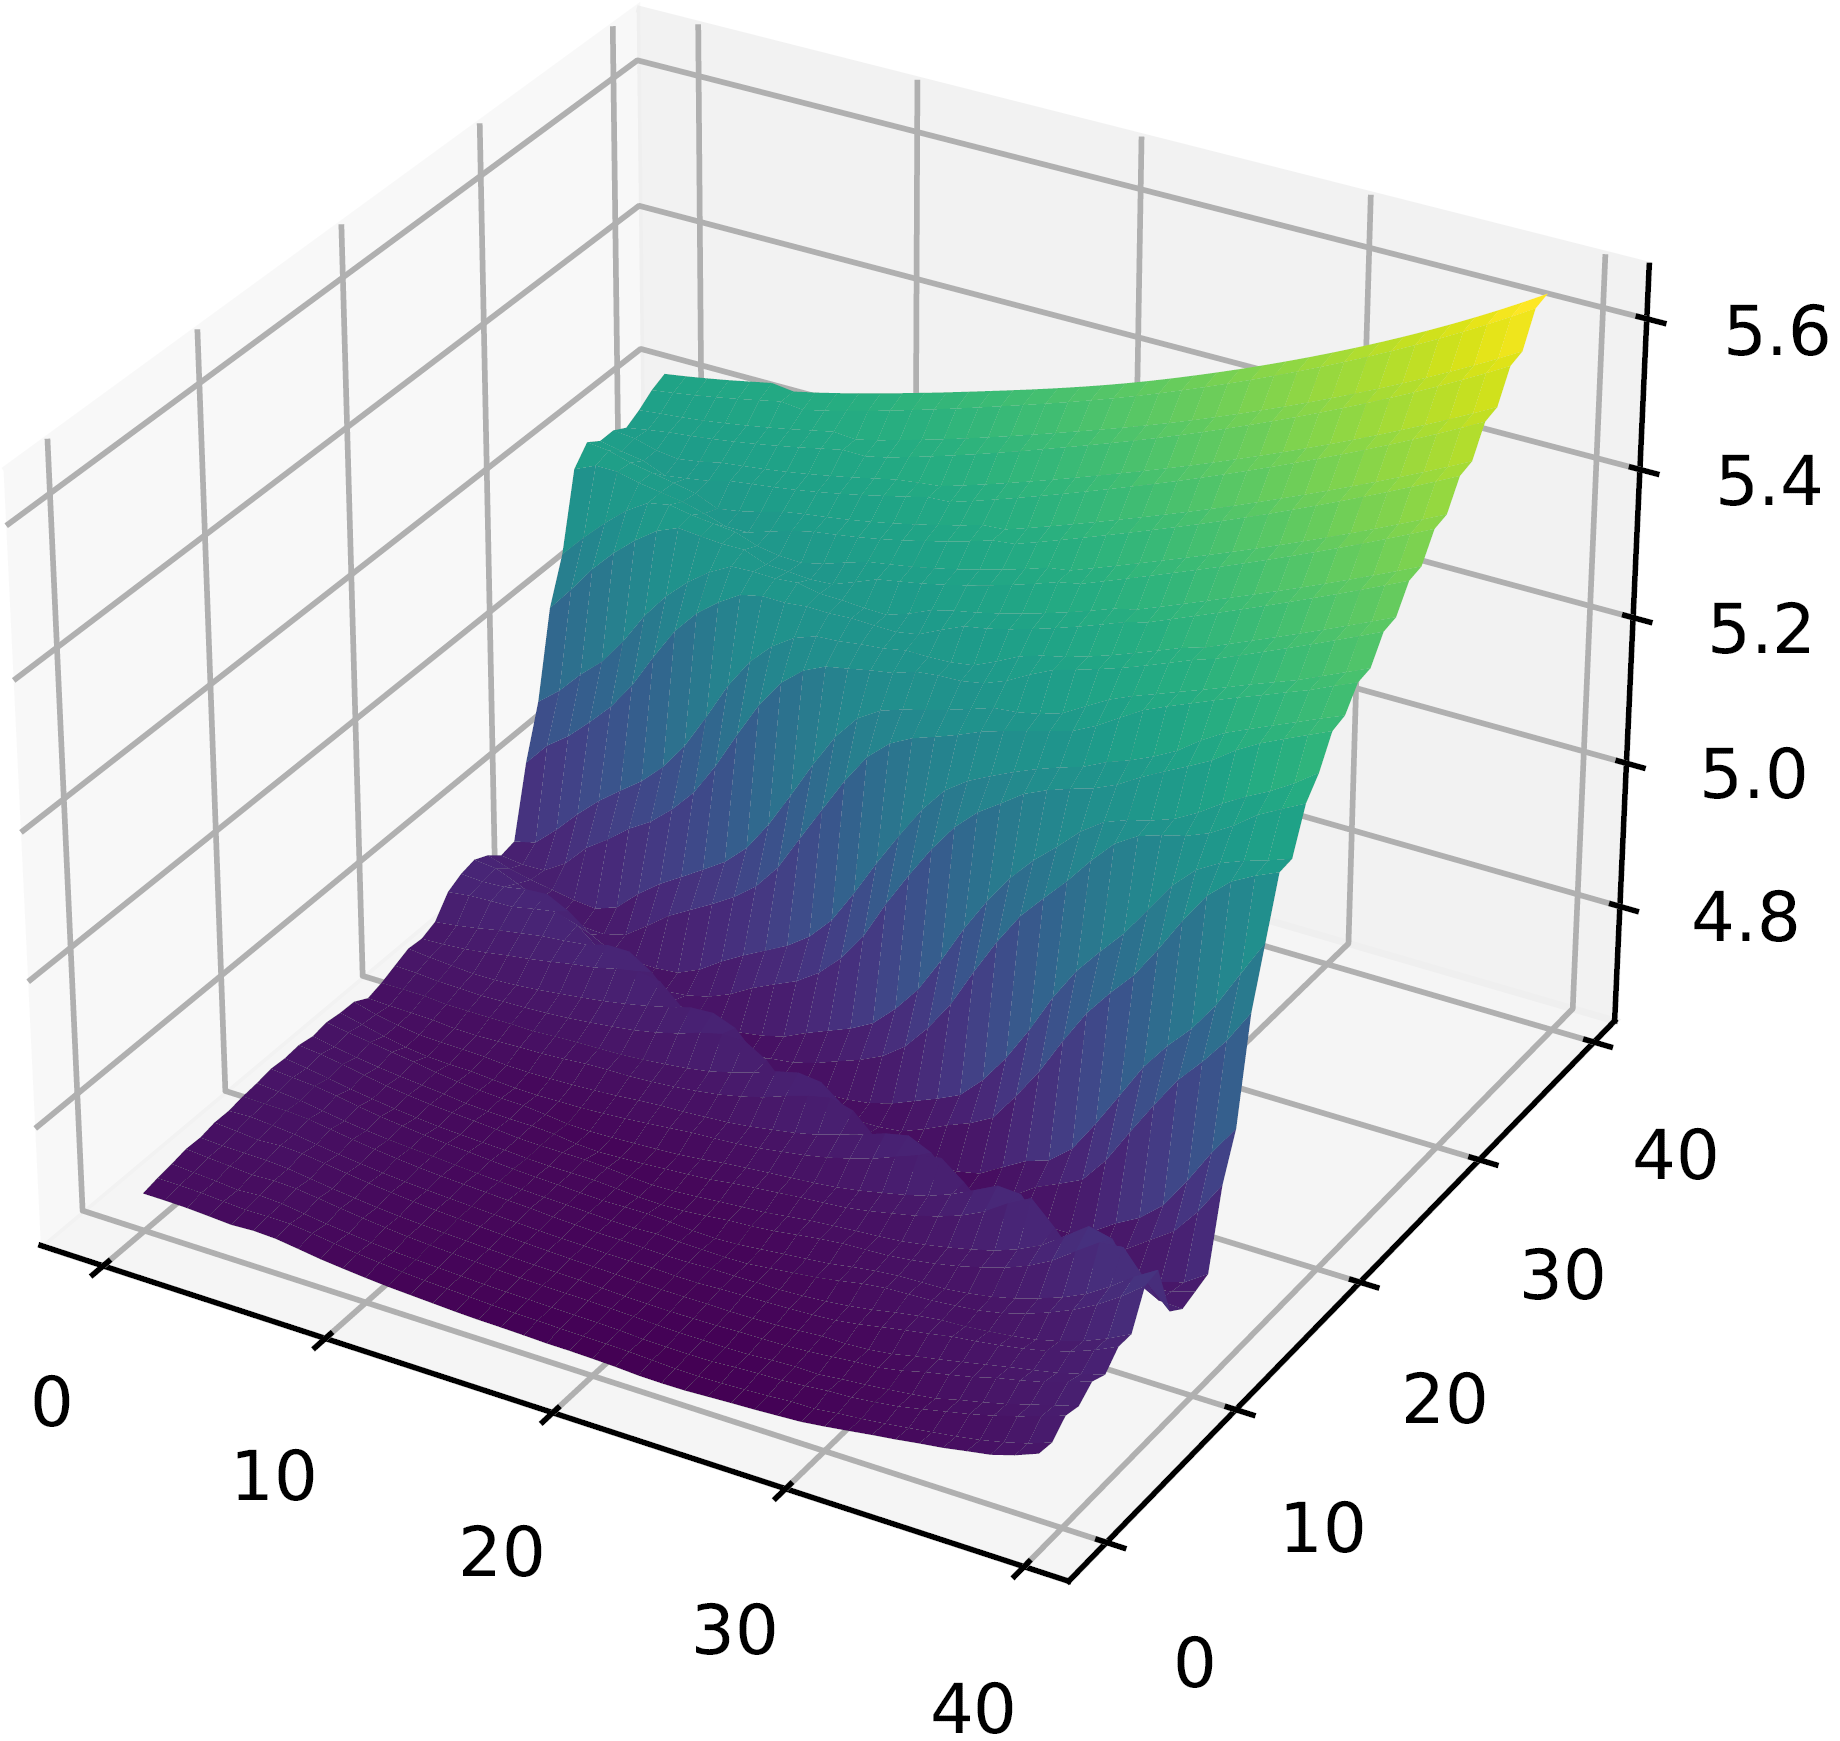} & \hspace{-0.15in}
    \includegraphics[width=0.16\textwidth]{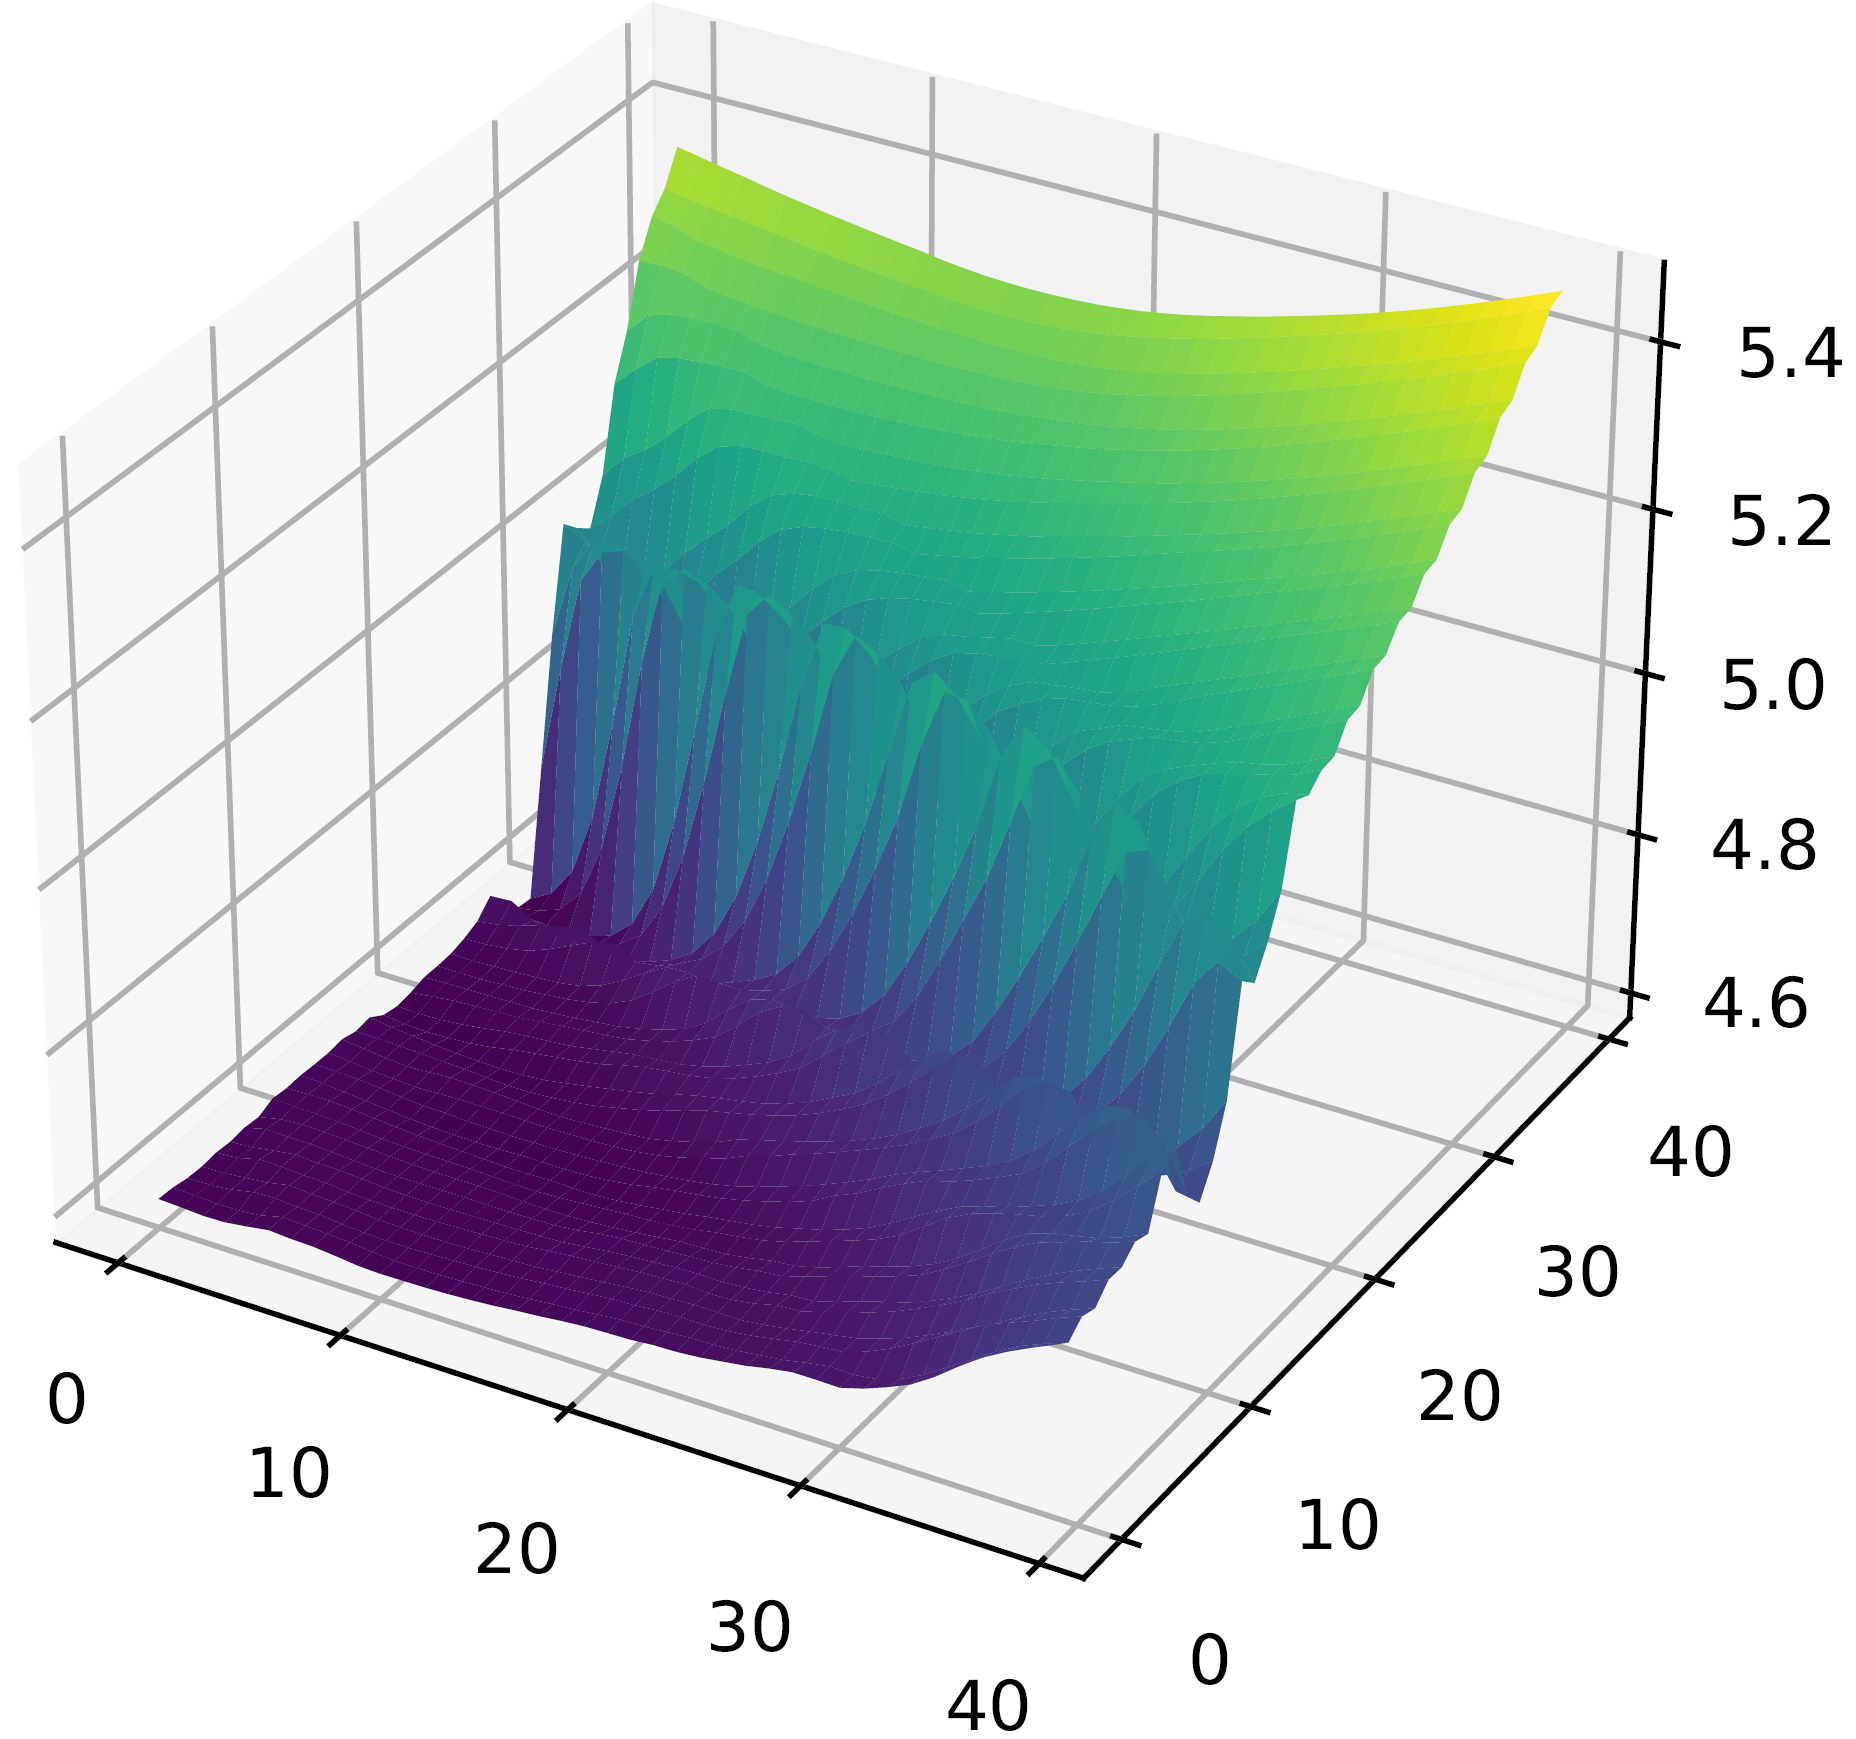} & \hspace{-0.15in}
    \includegraphics[width=0.16\textwidth]{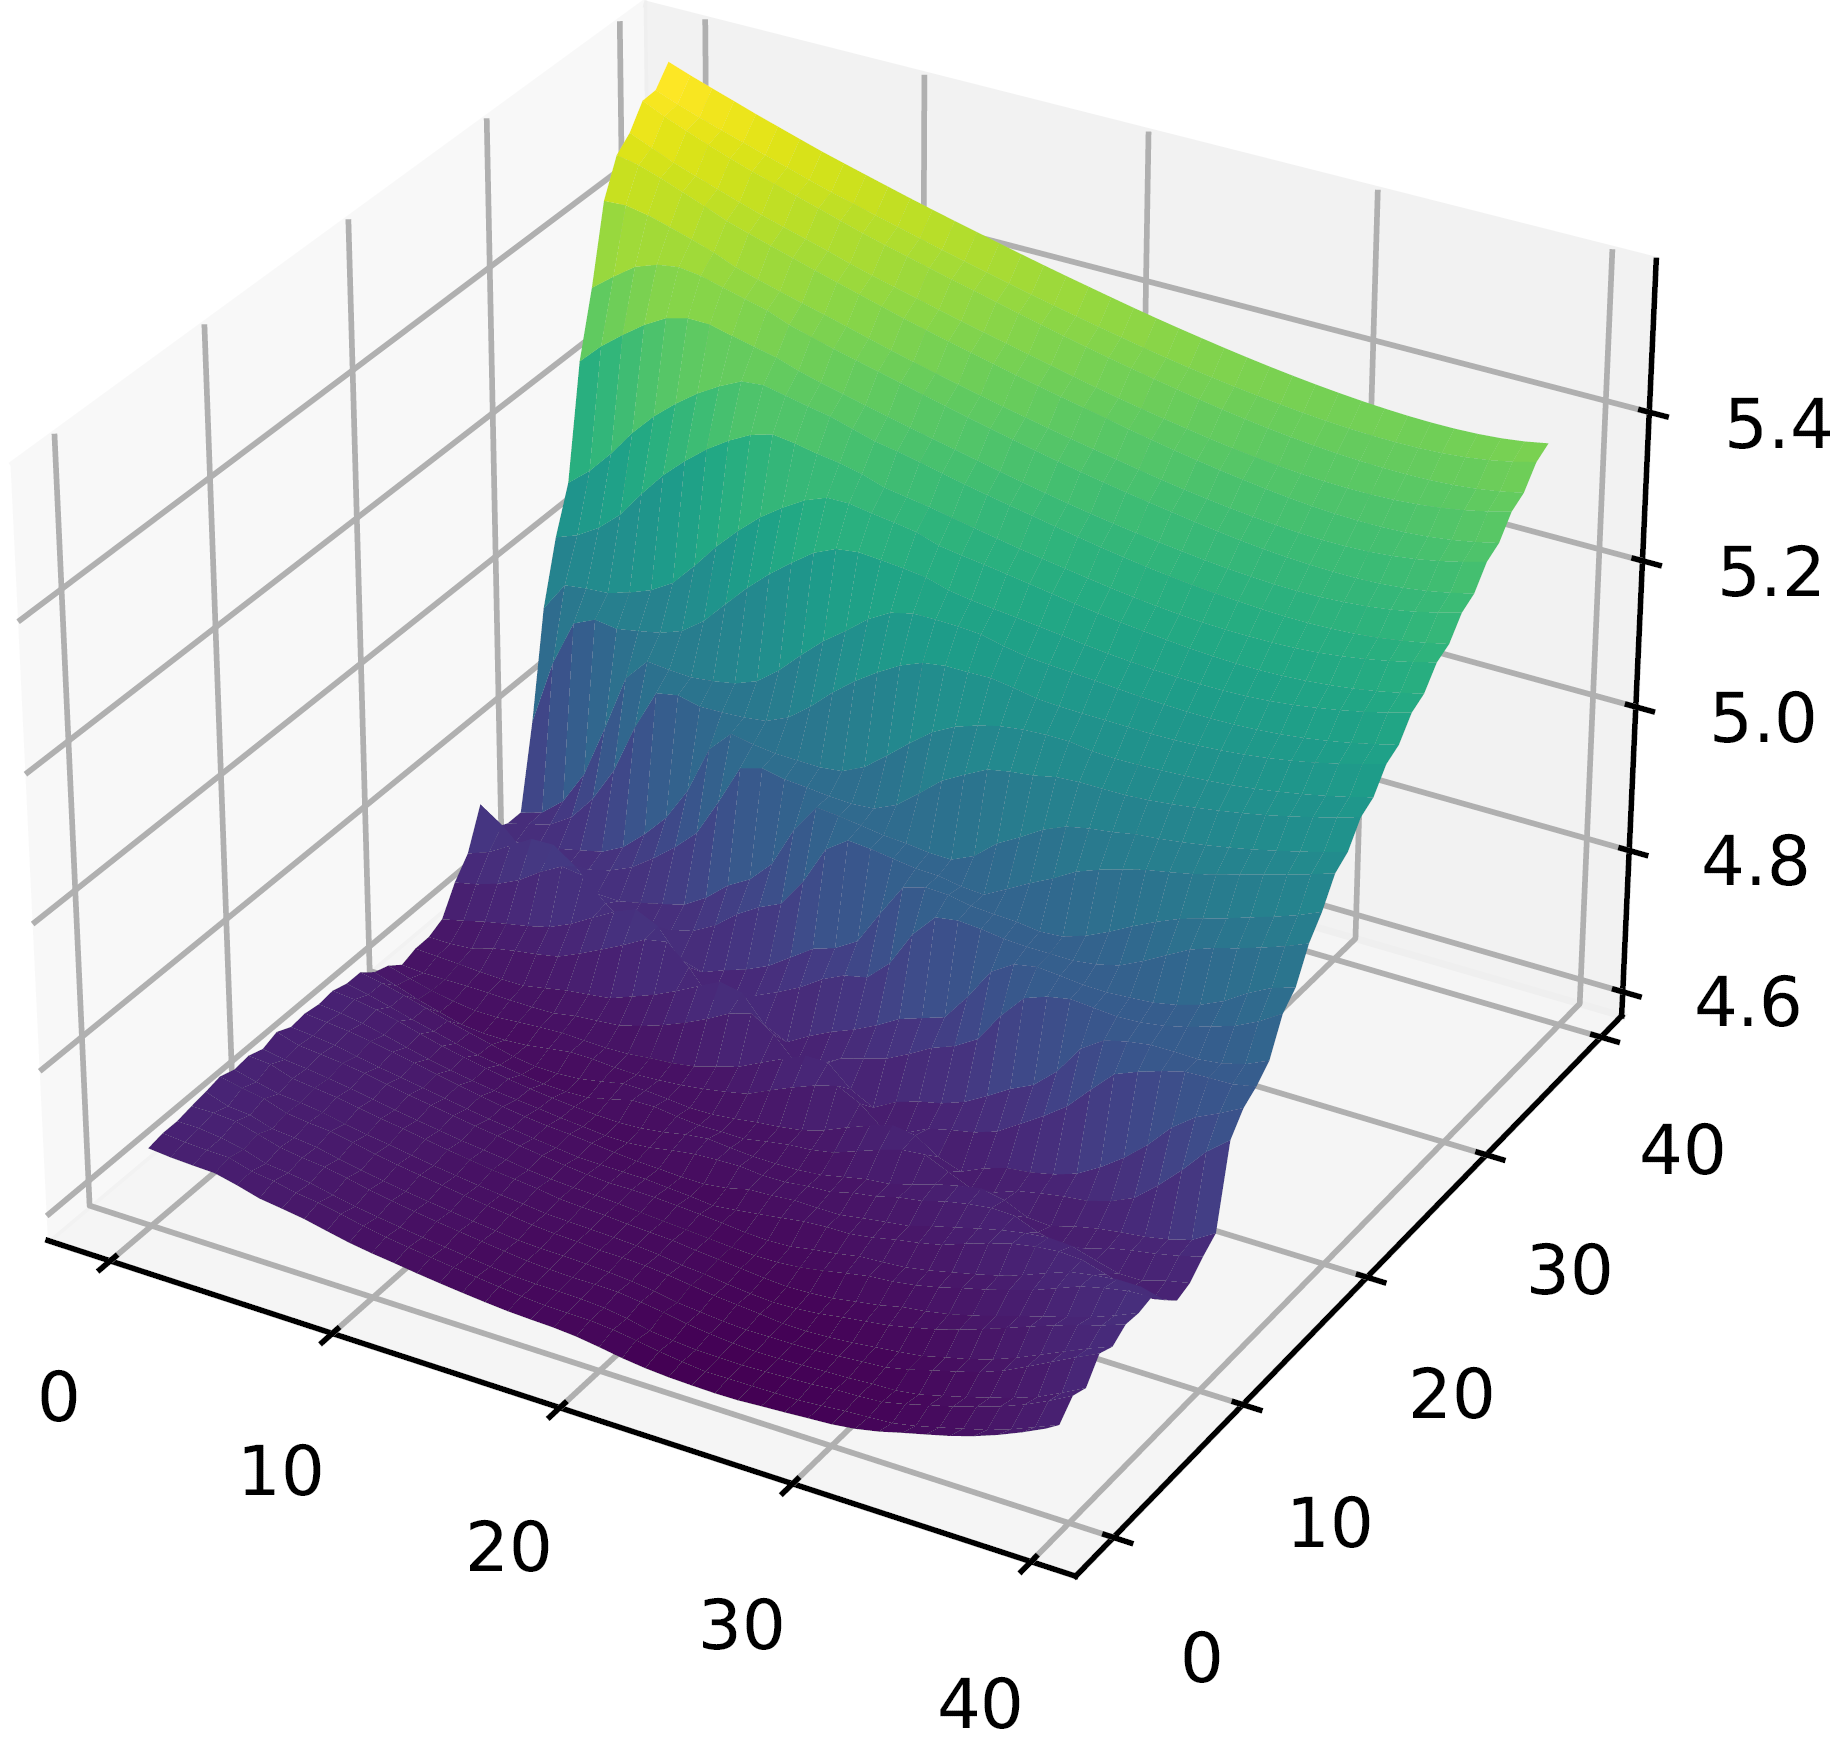} \\
\hspace{-0.15in}\rowlegend{~~~~$t=17$}
    \includegraphics[width=0.16\textwidth]{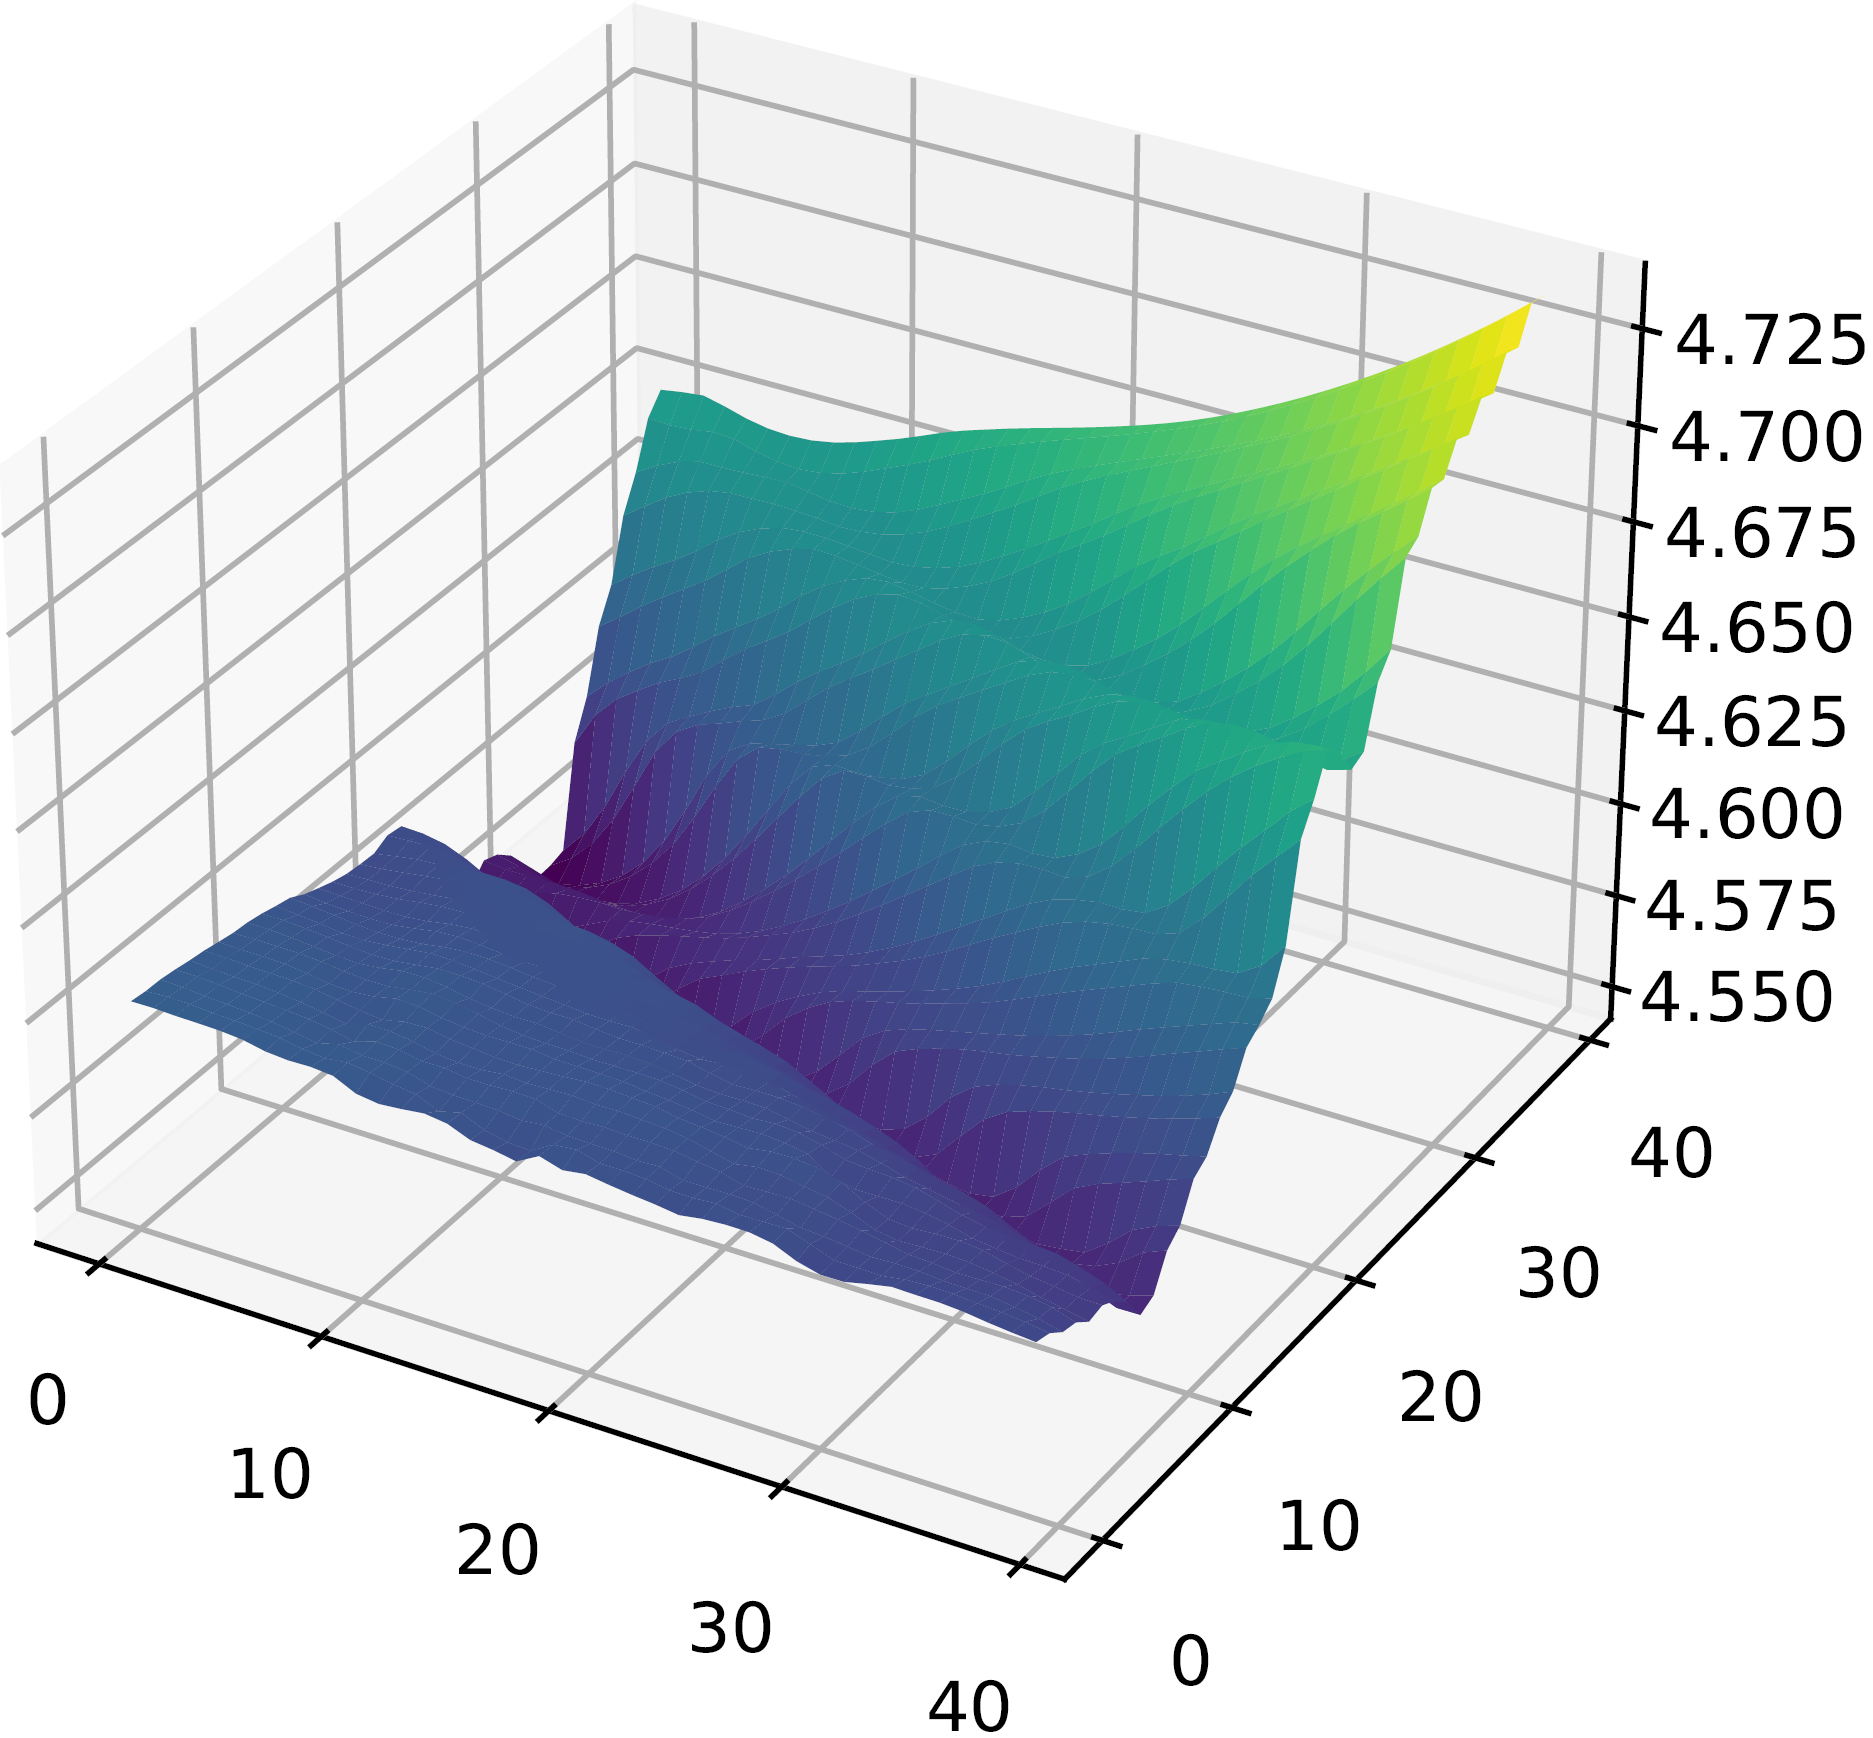} & \hspace{-0.15in}
    \includegraphics[width=0.16\textwidth]{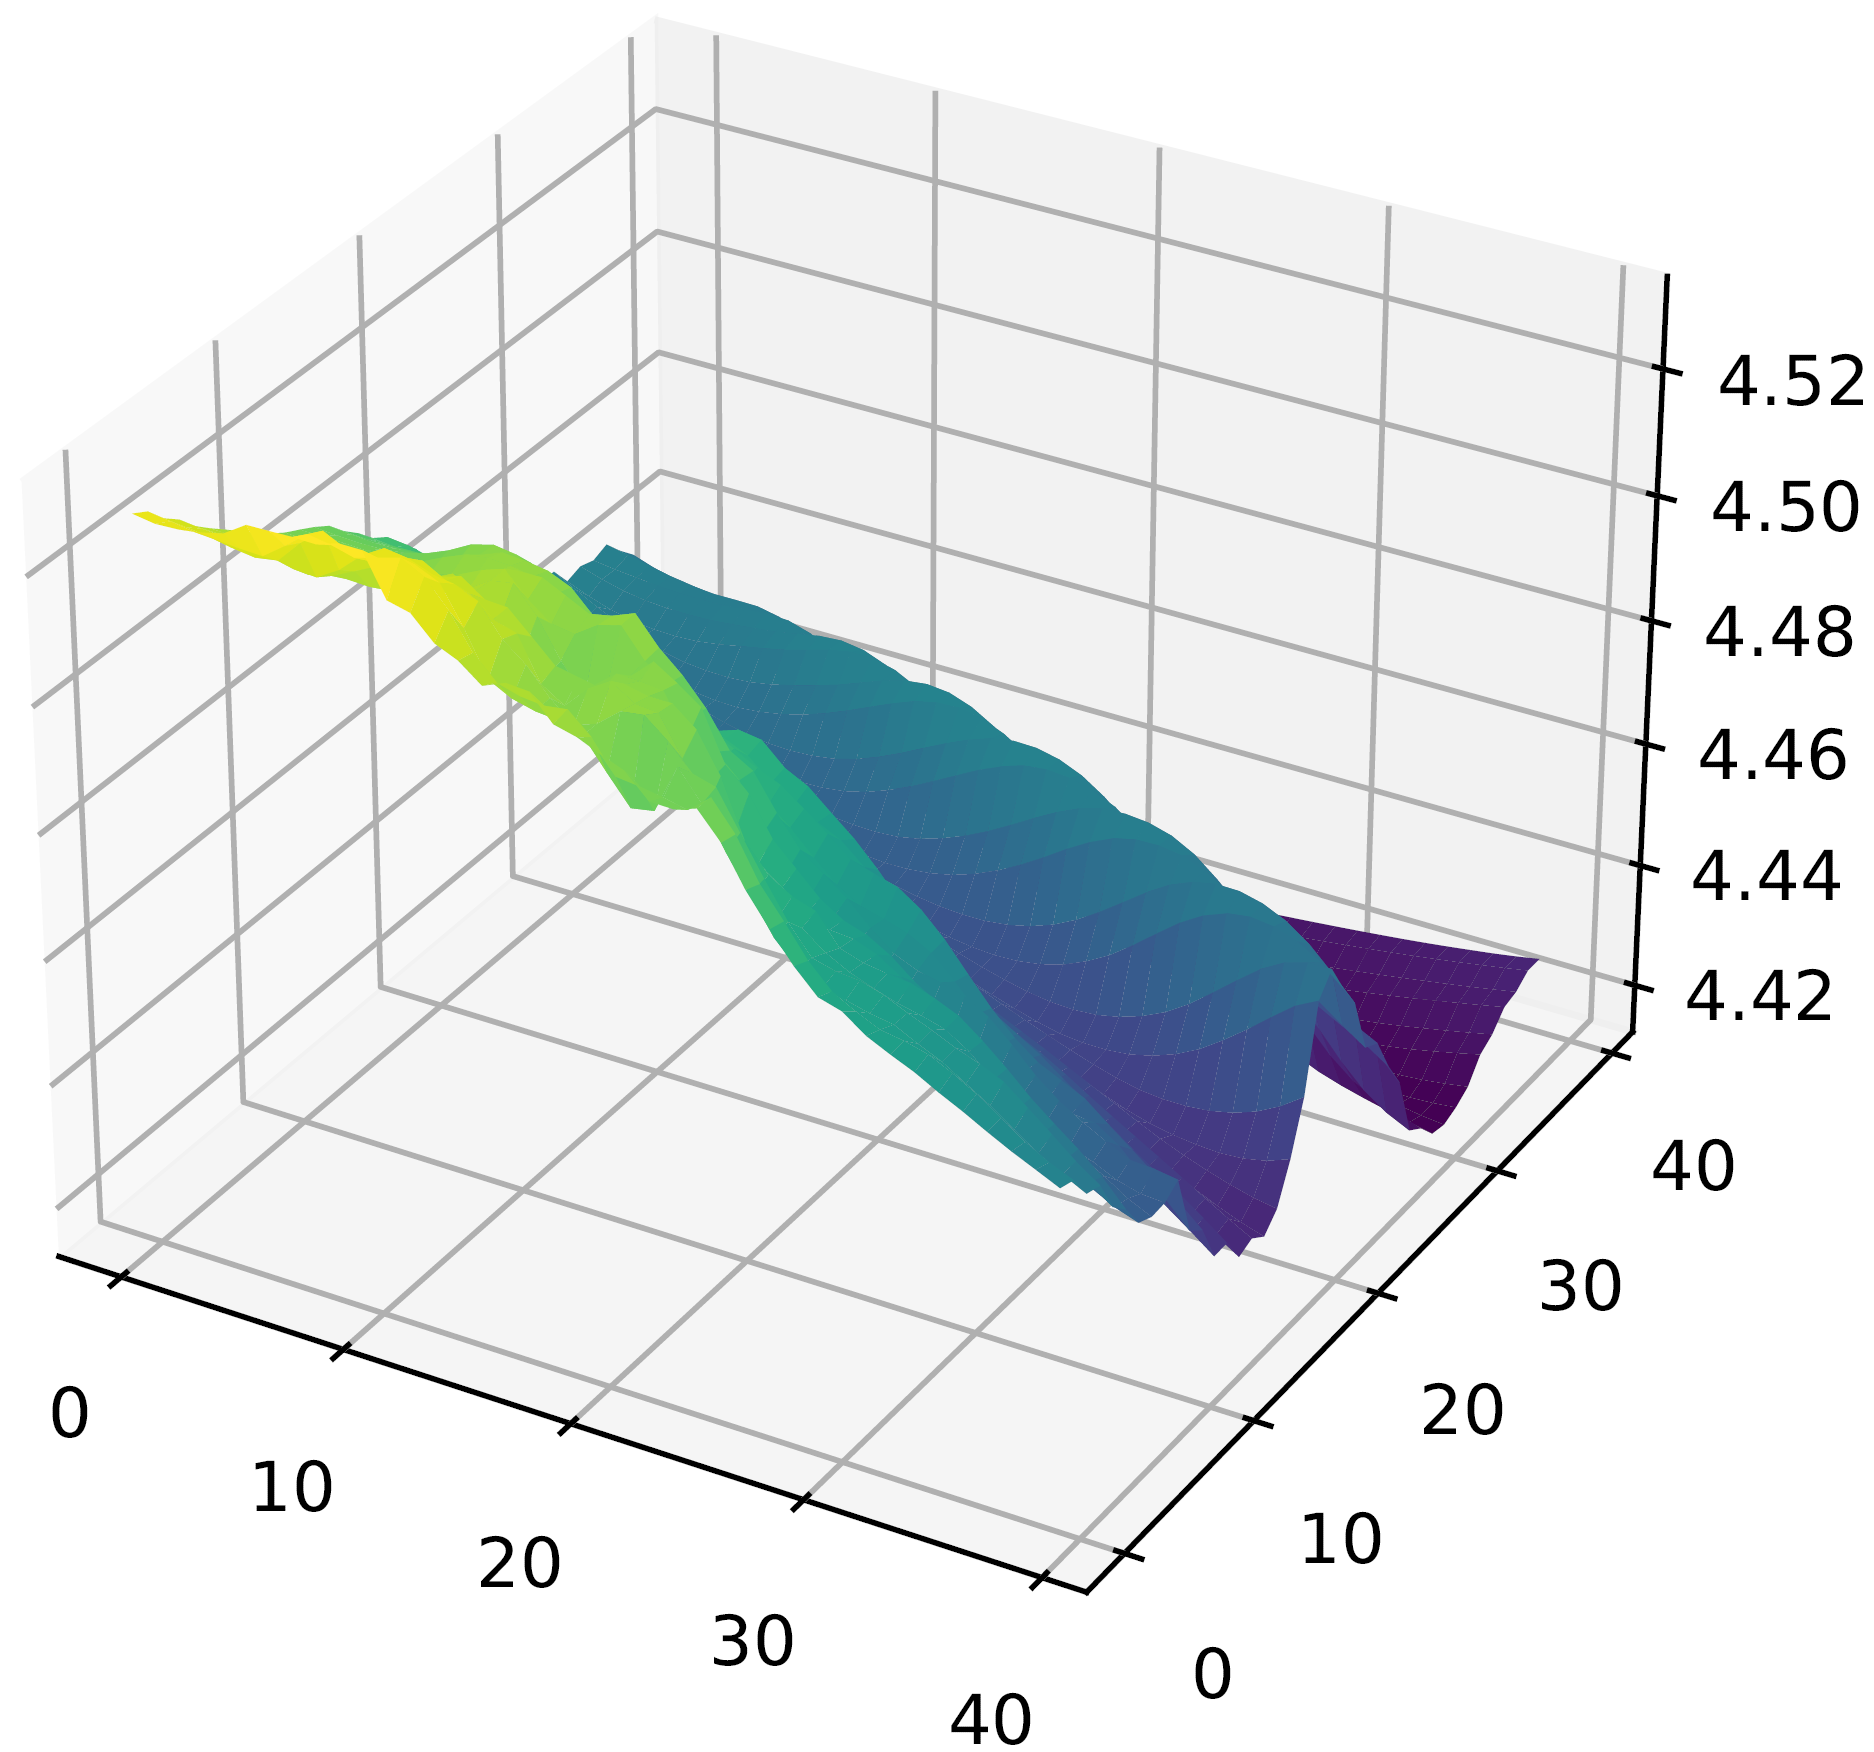} & \hspace{-0.15in}
    \includegraphics[width=0.16\textwidth]{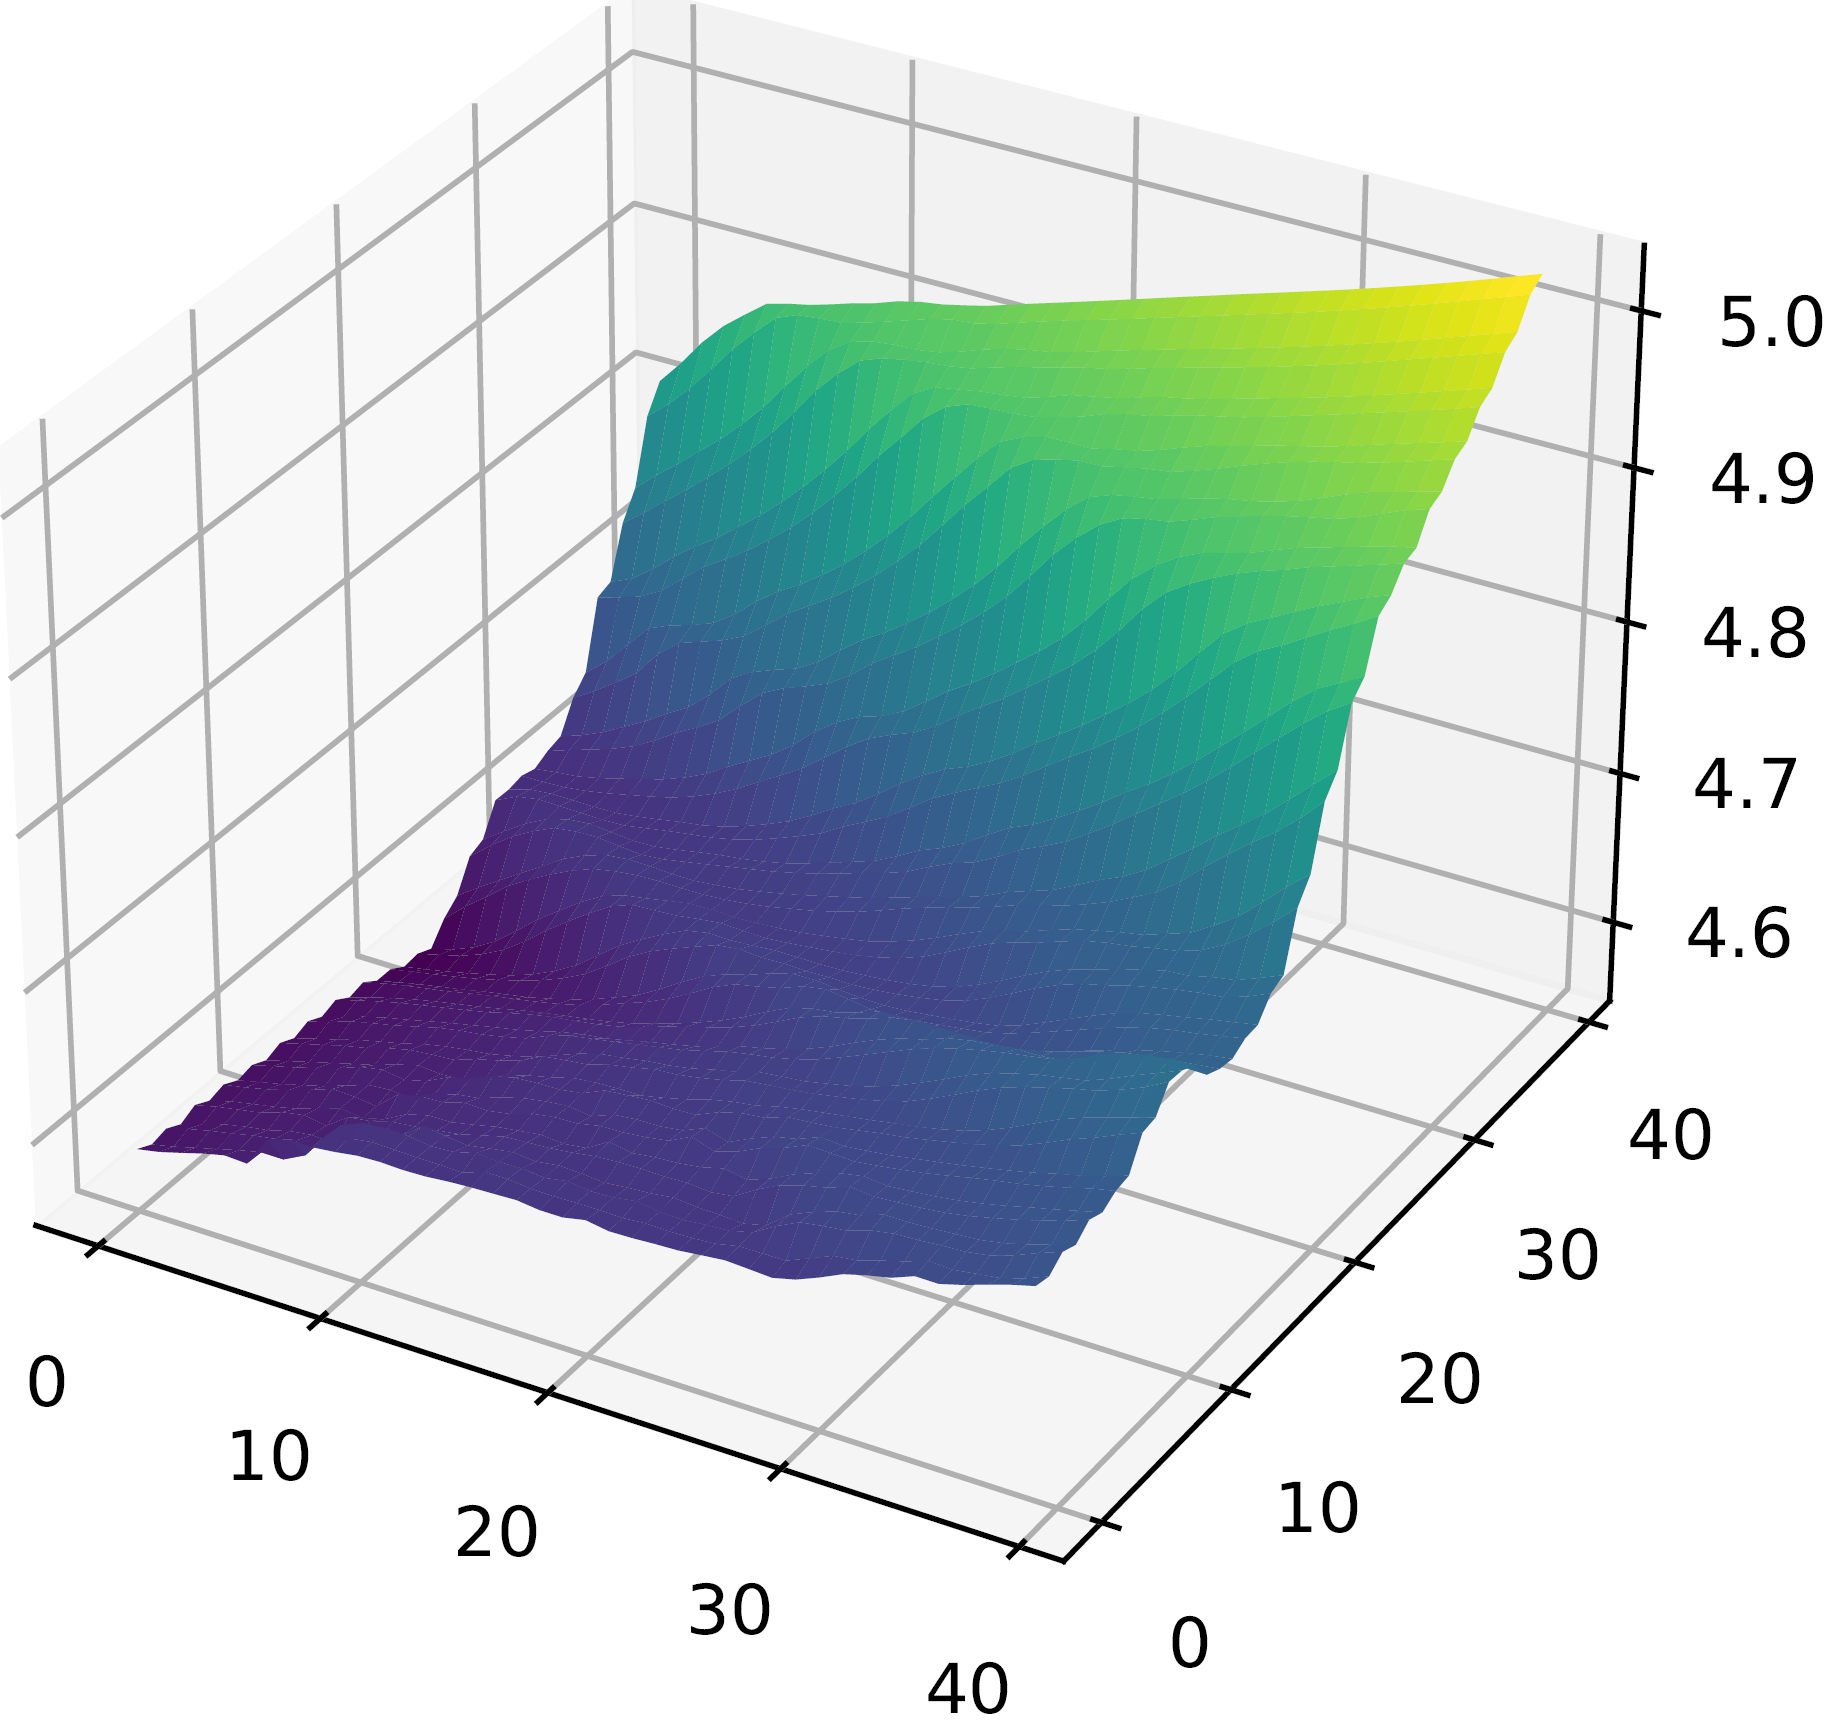} & \hspace{-0.15in}
    \includegraphics[width=0.16\textwidth]{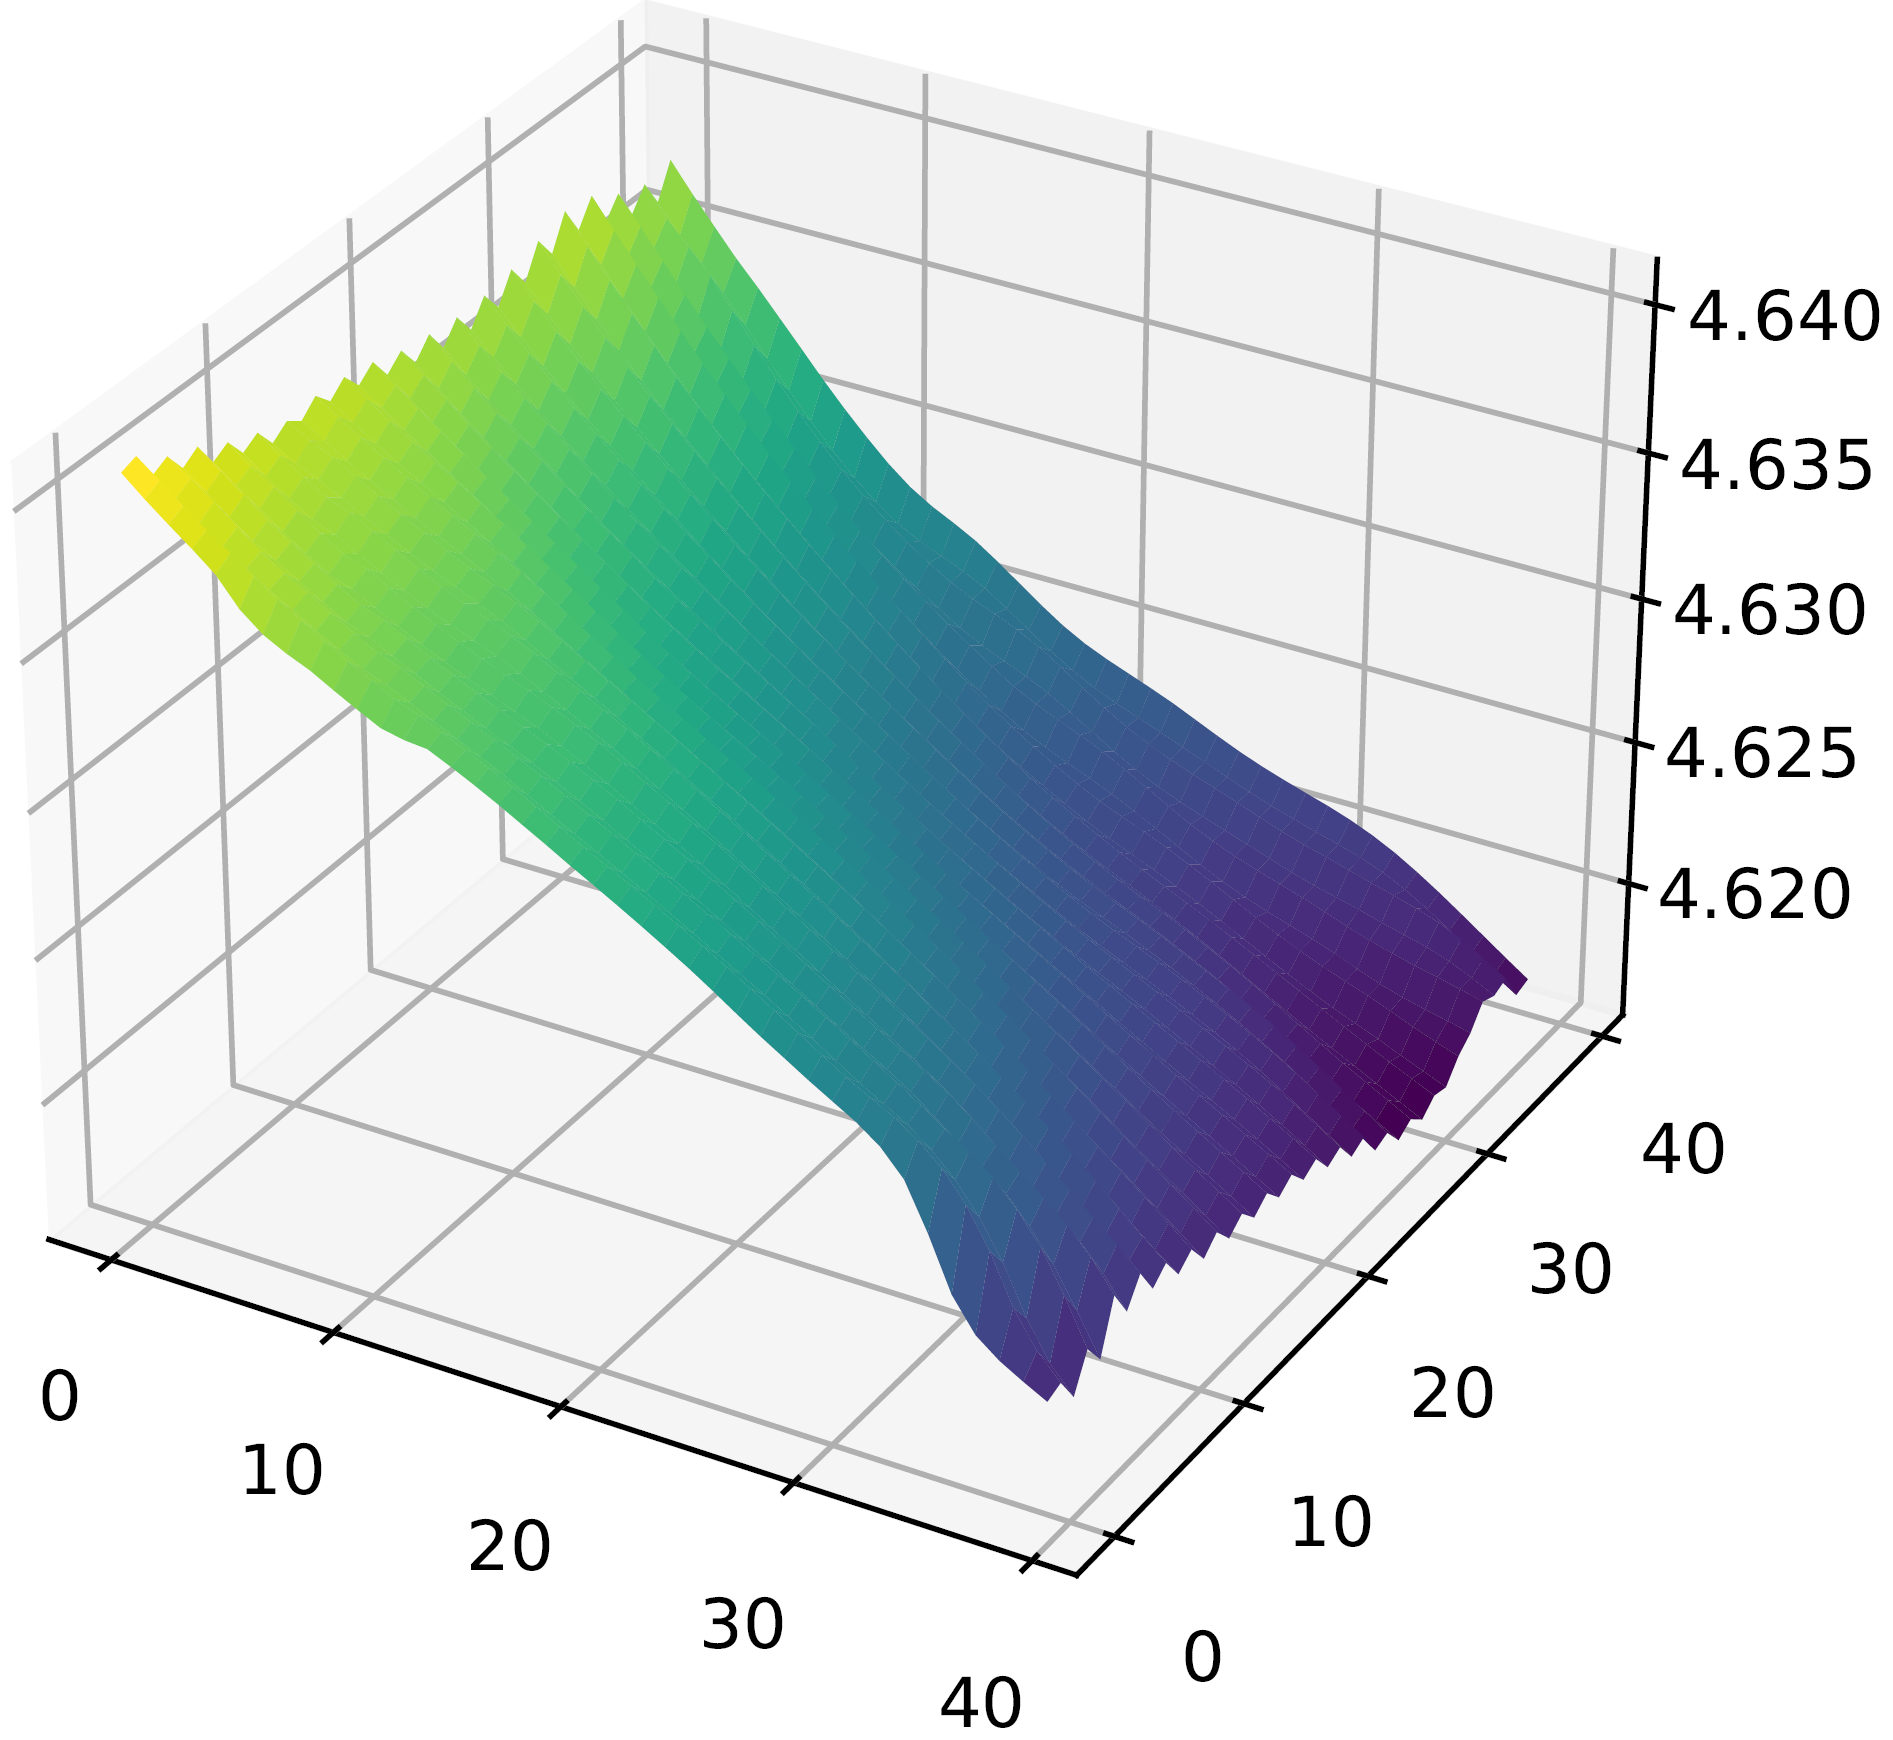} & \hspace{-0.15in}
    \includegraphics[width=0.16\textwidth]{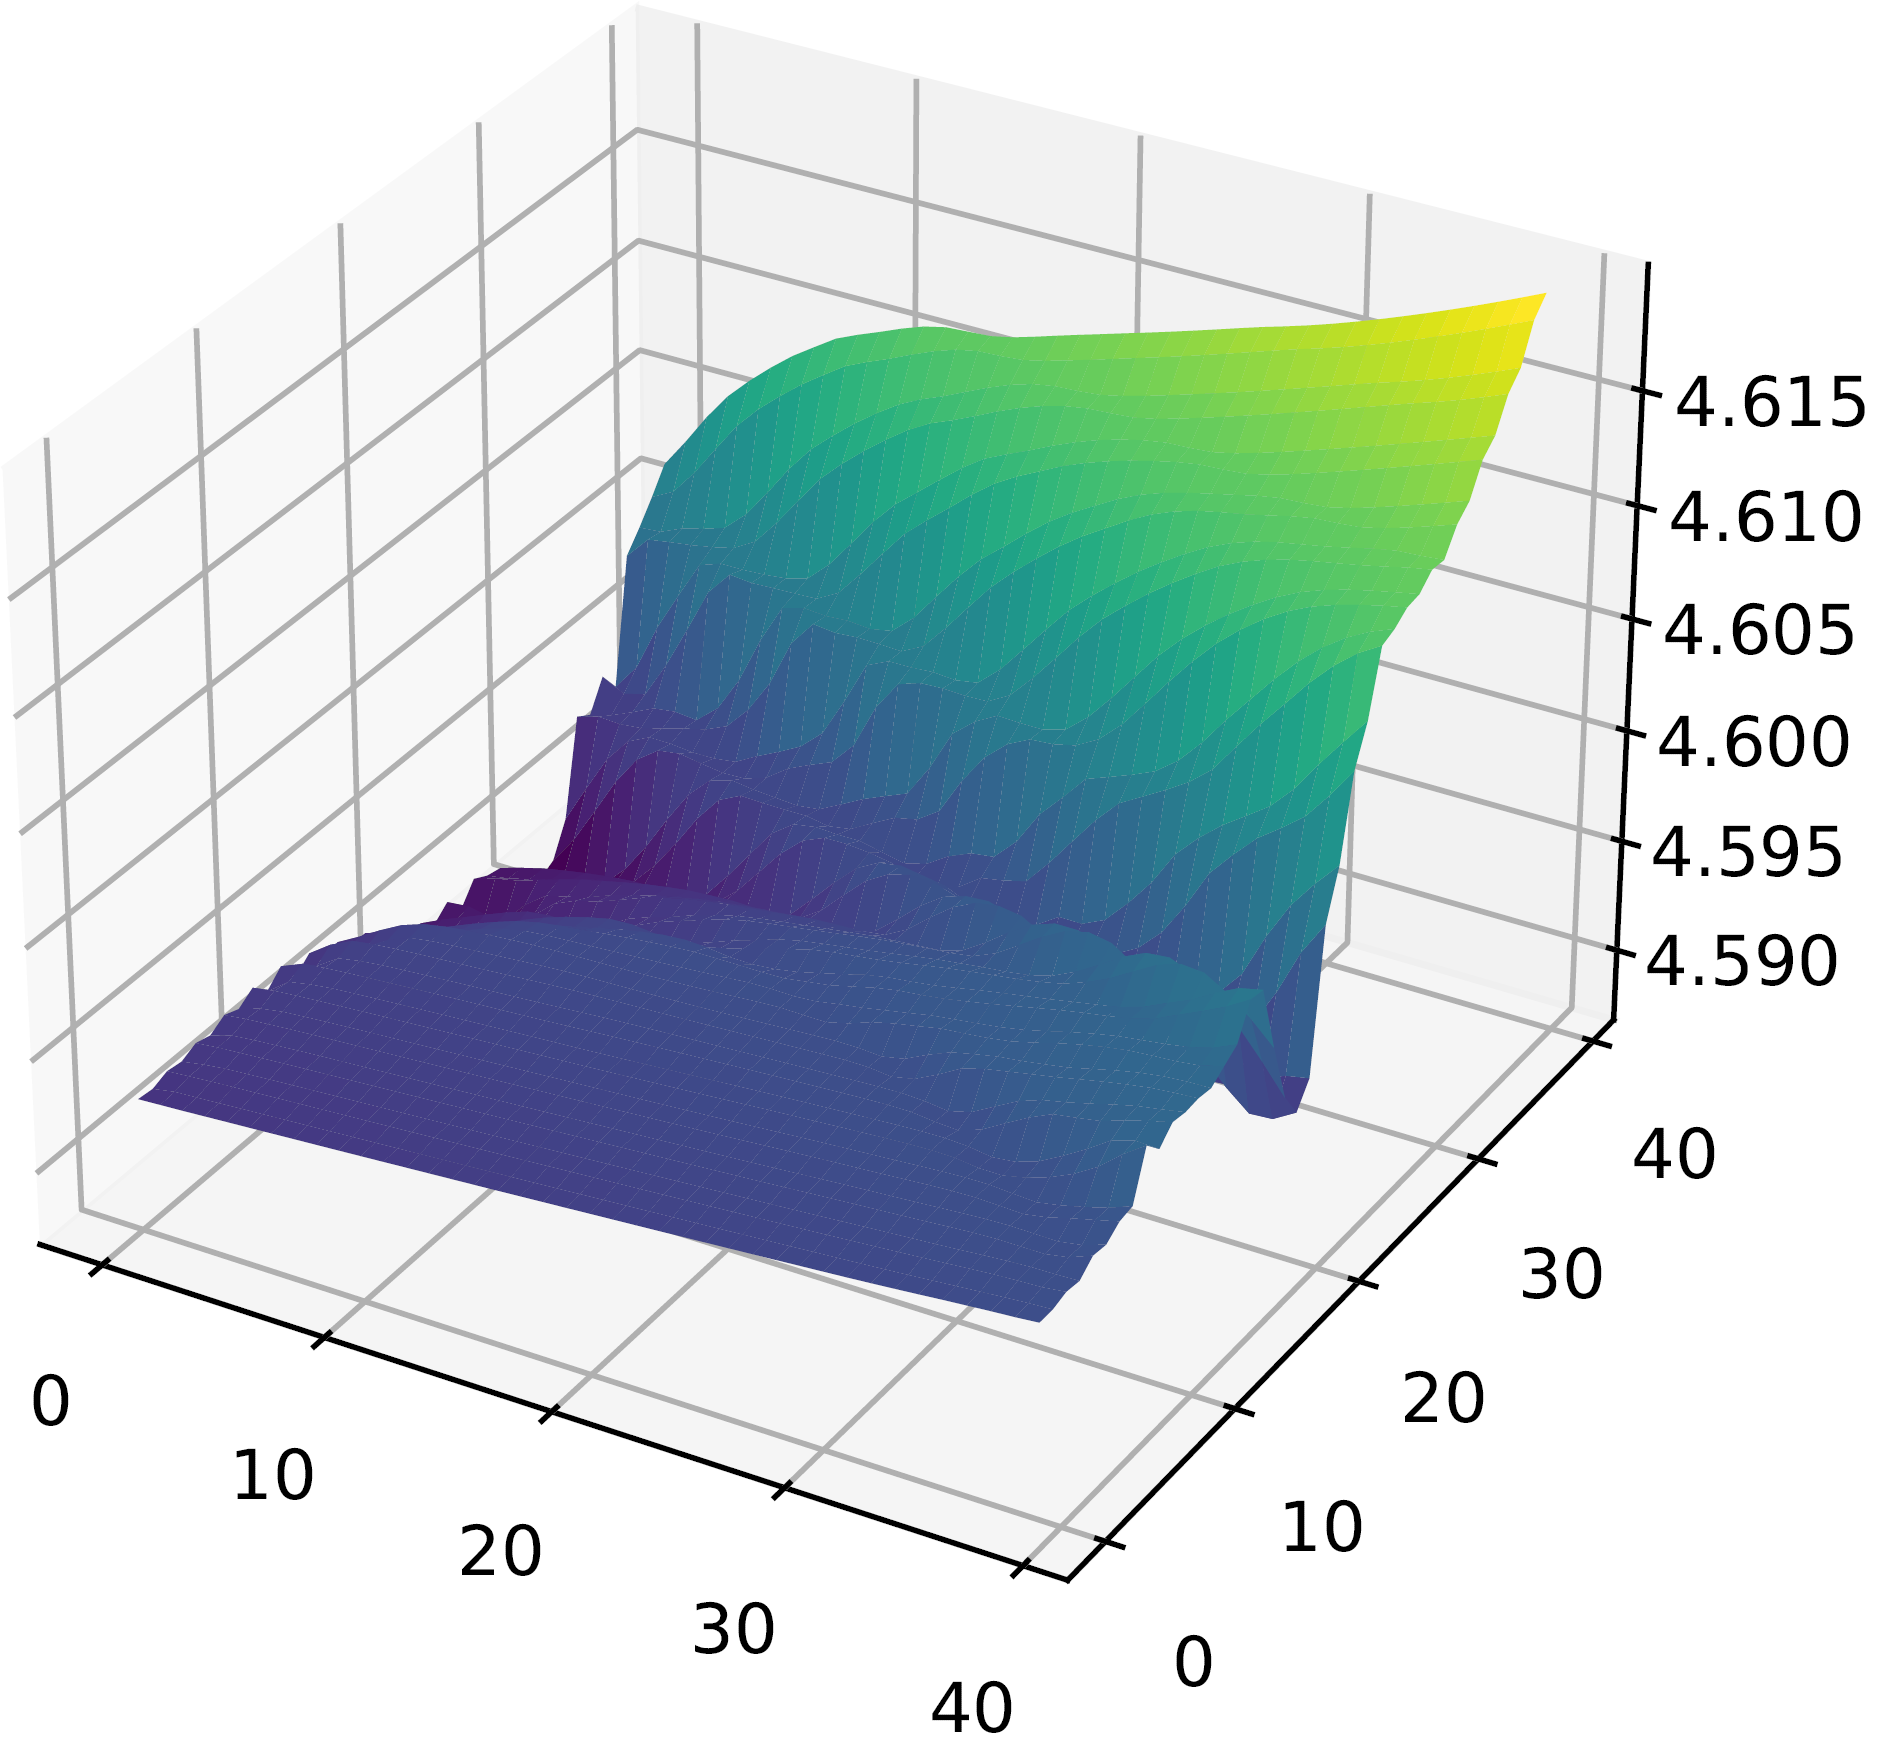} & \hspace{-0.15in}
    \includegraphics[width=0.16\textwidth]{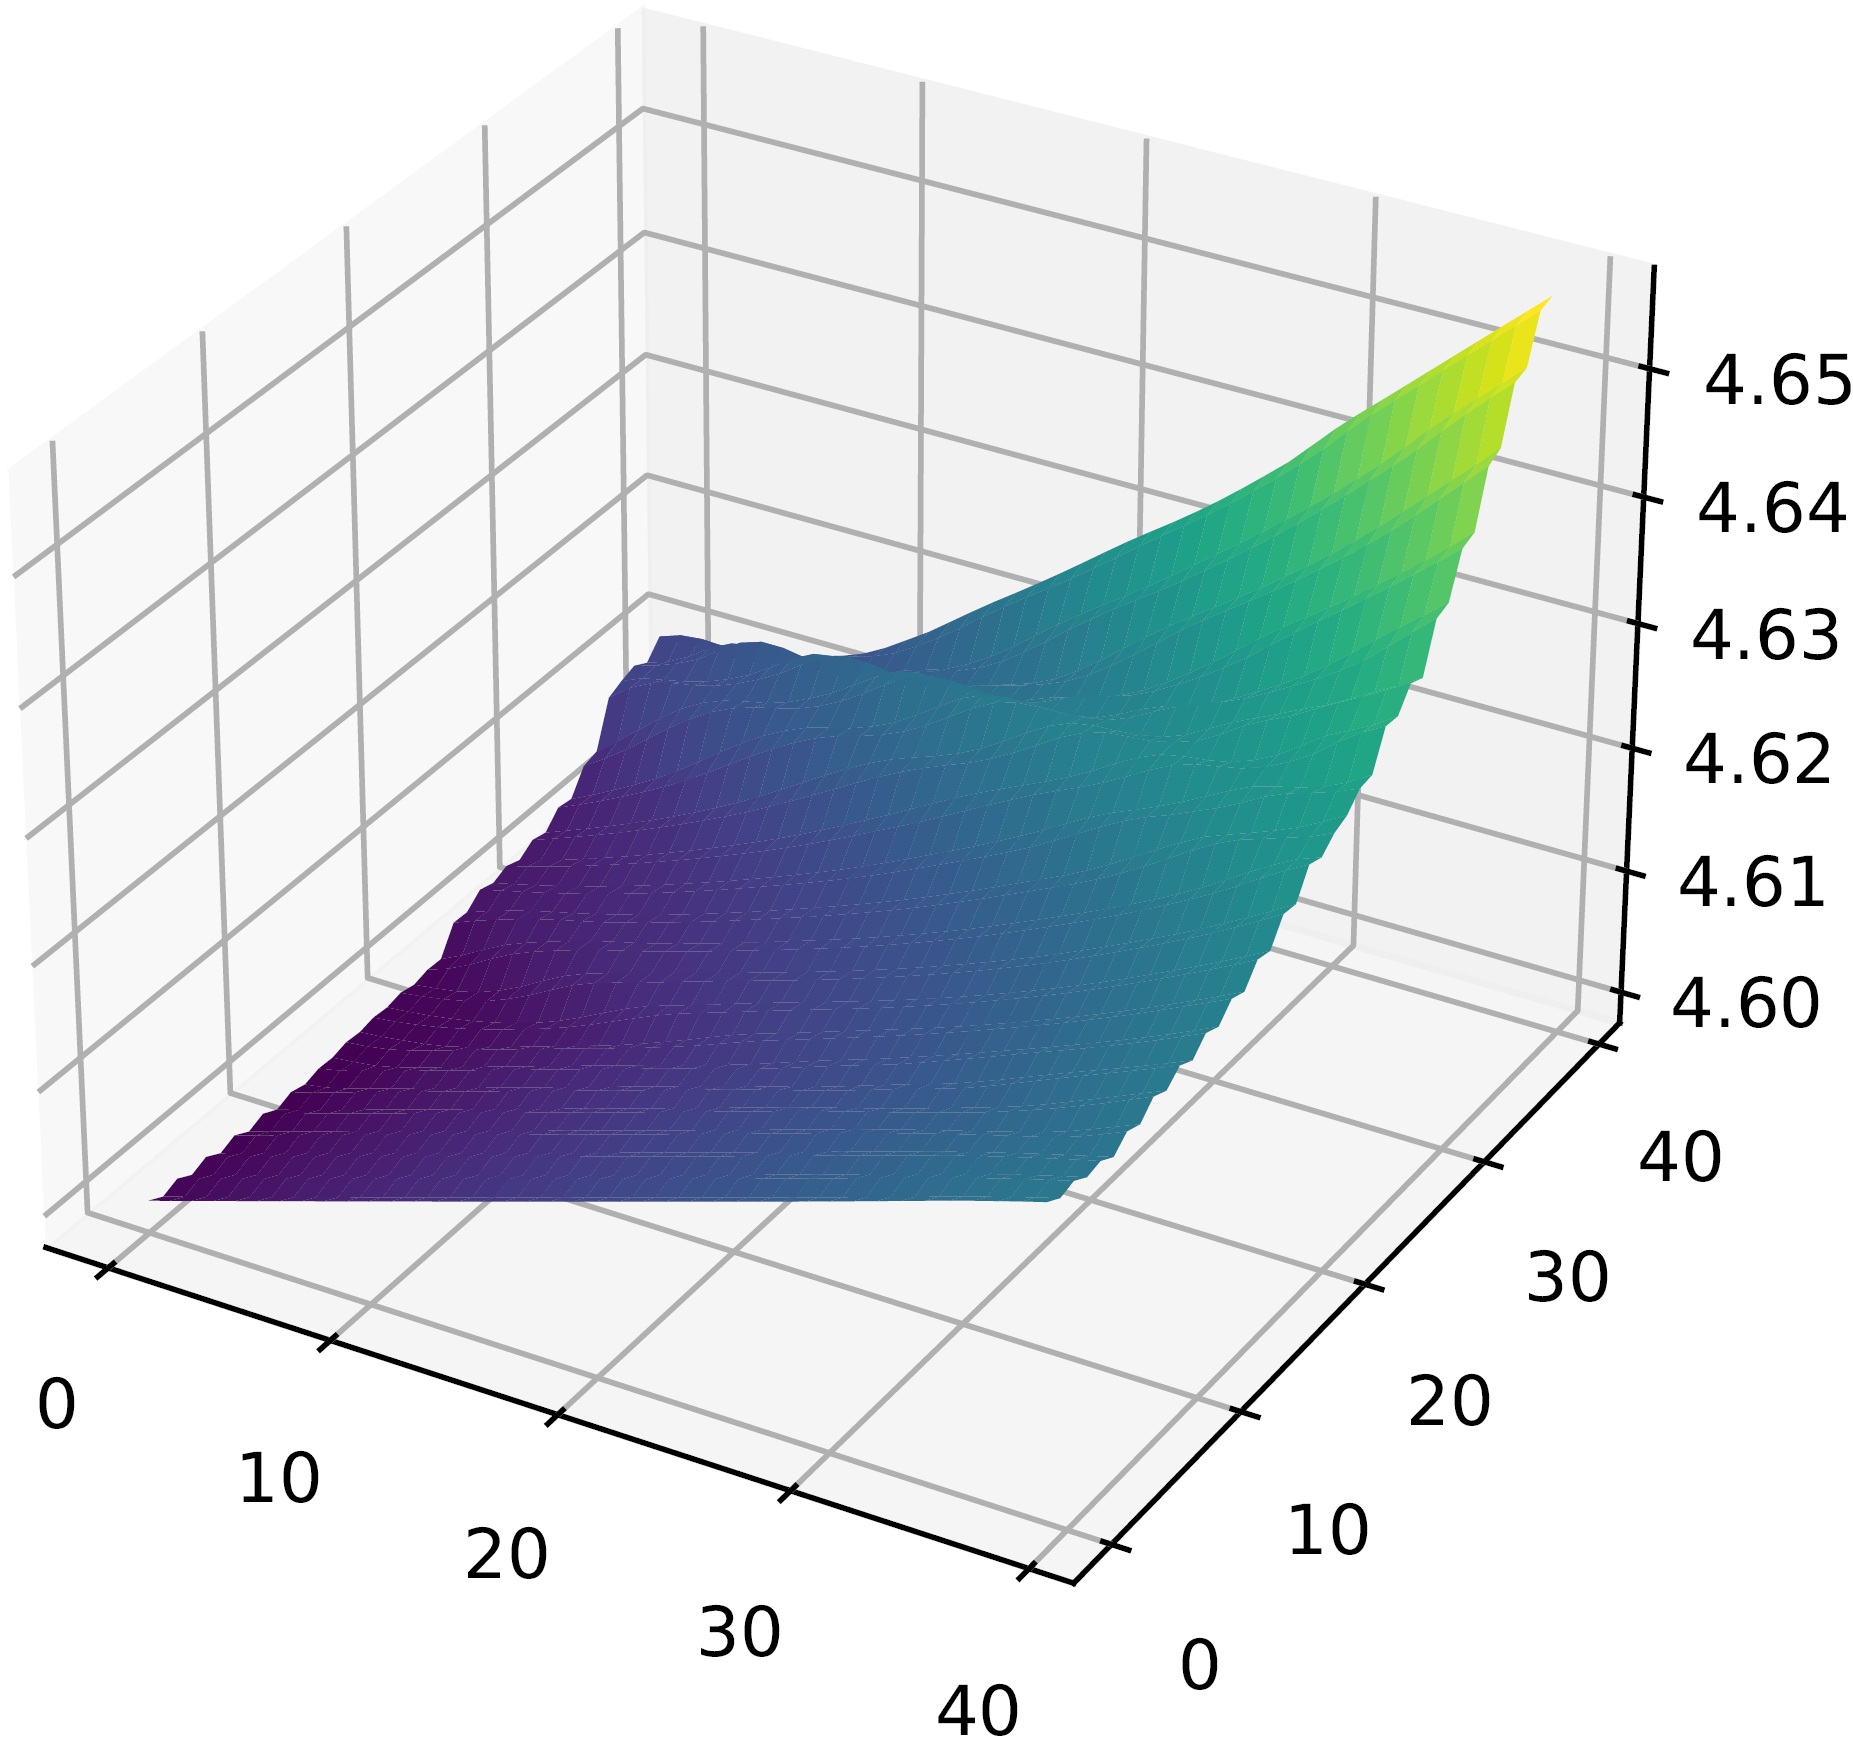} \\
\hspace{-0.15in}\rowlegend{~~~~$t=18$}
    \includegraphics[width=0.16\textwidth]{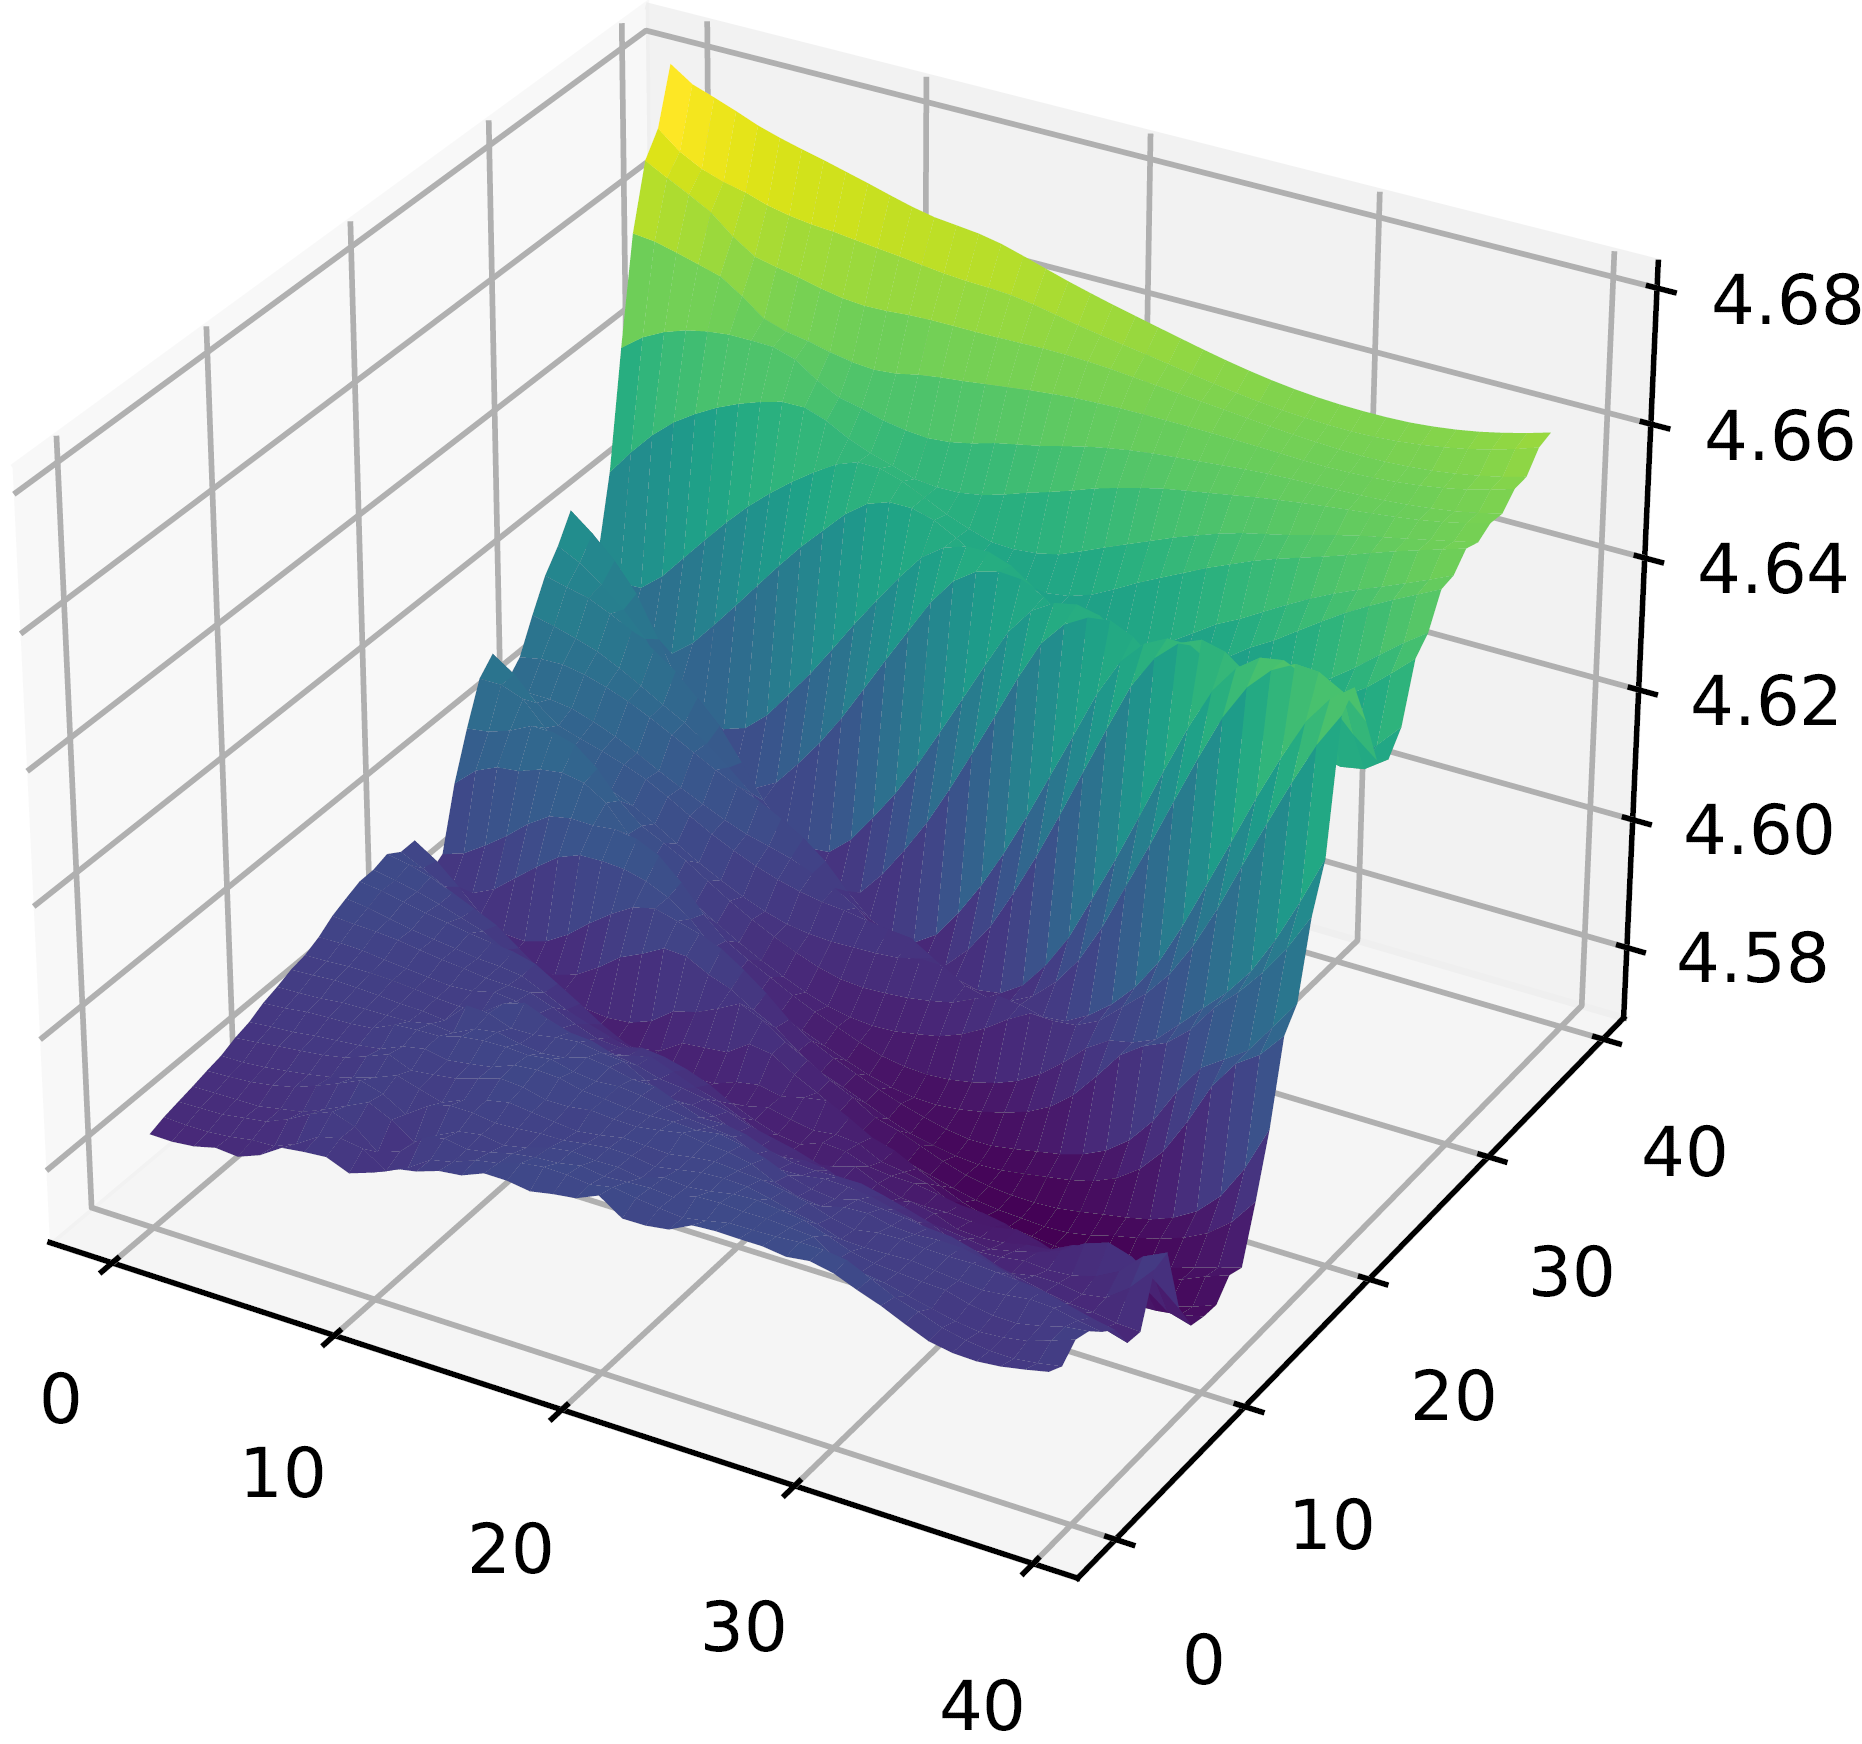} & \hspace{-0.15in}
    \includegraphics[width=0.16\textwidth]{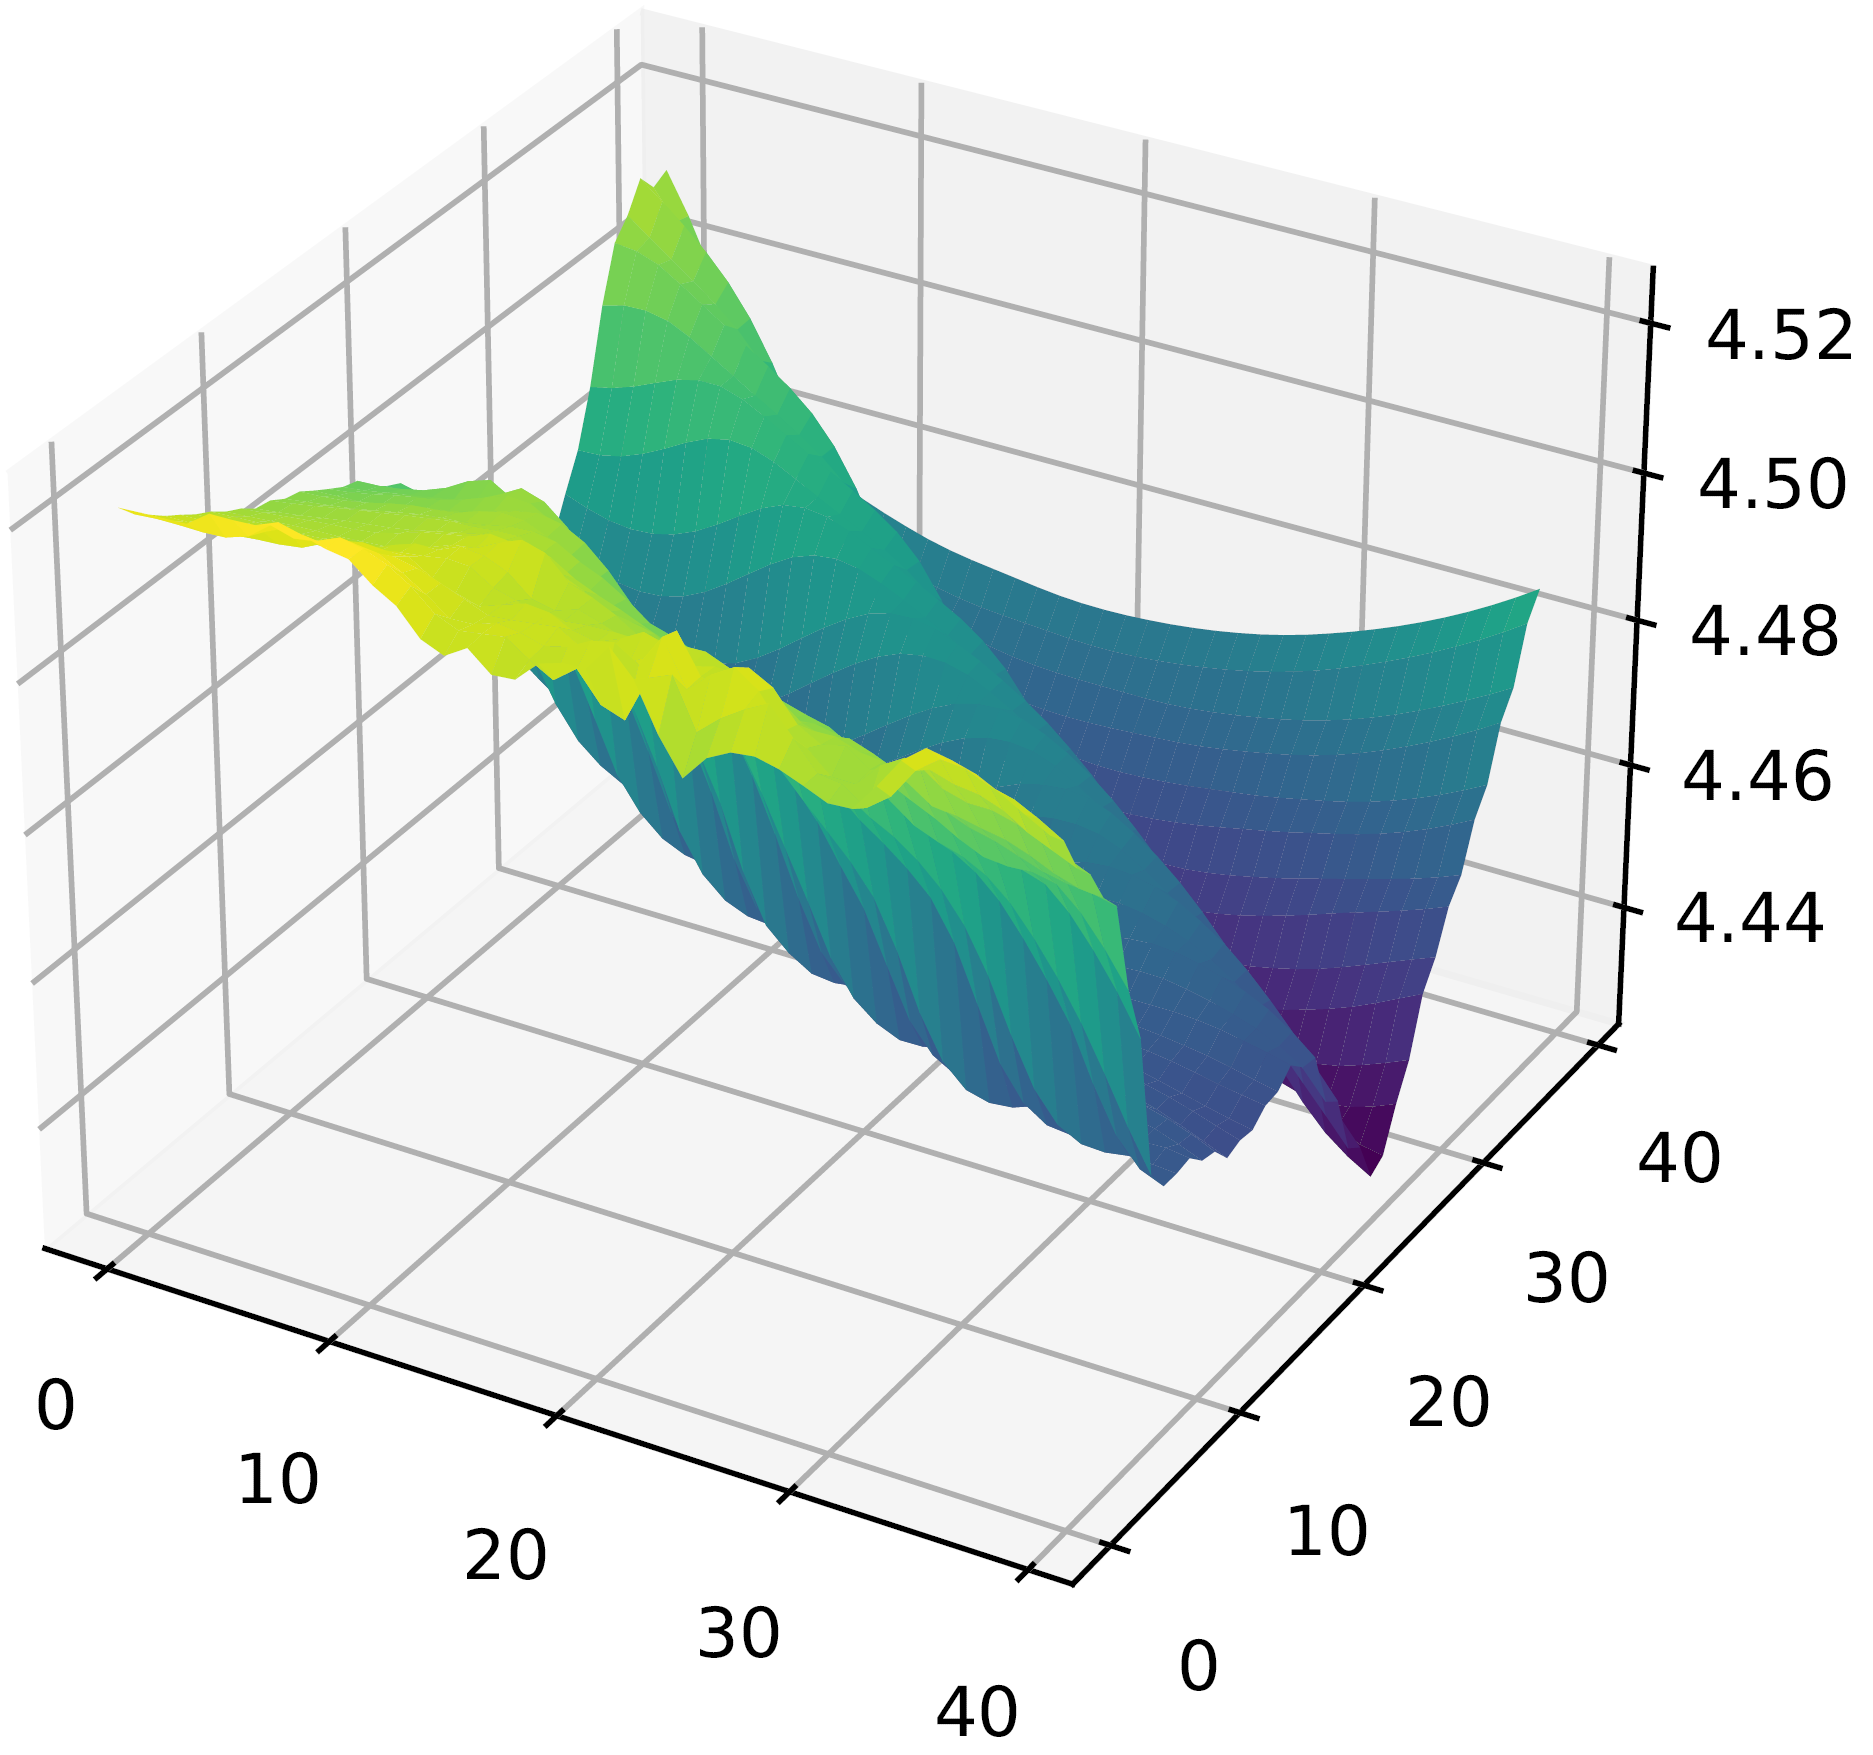} & \hspace{-0.15in}
    \includegraphics[width=0.16\textwidth]{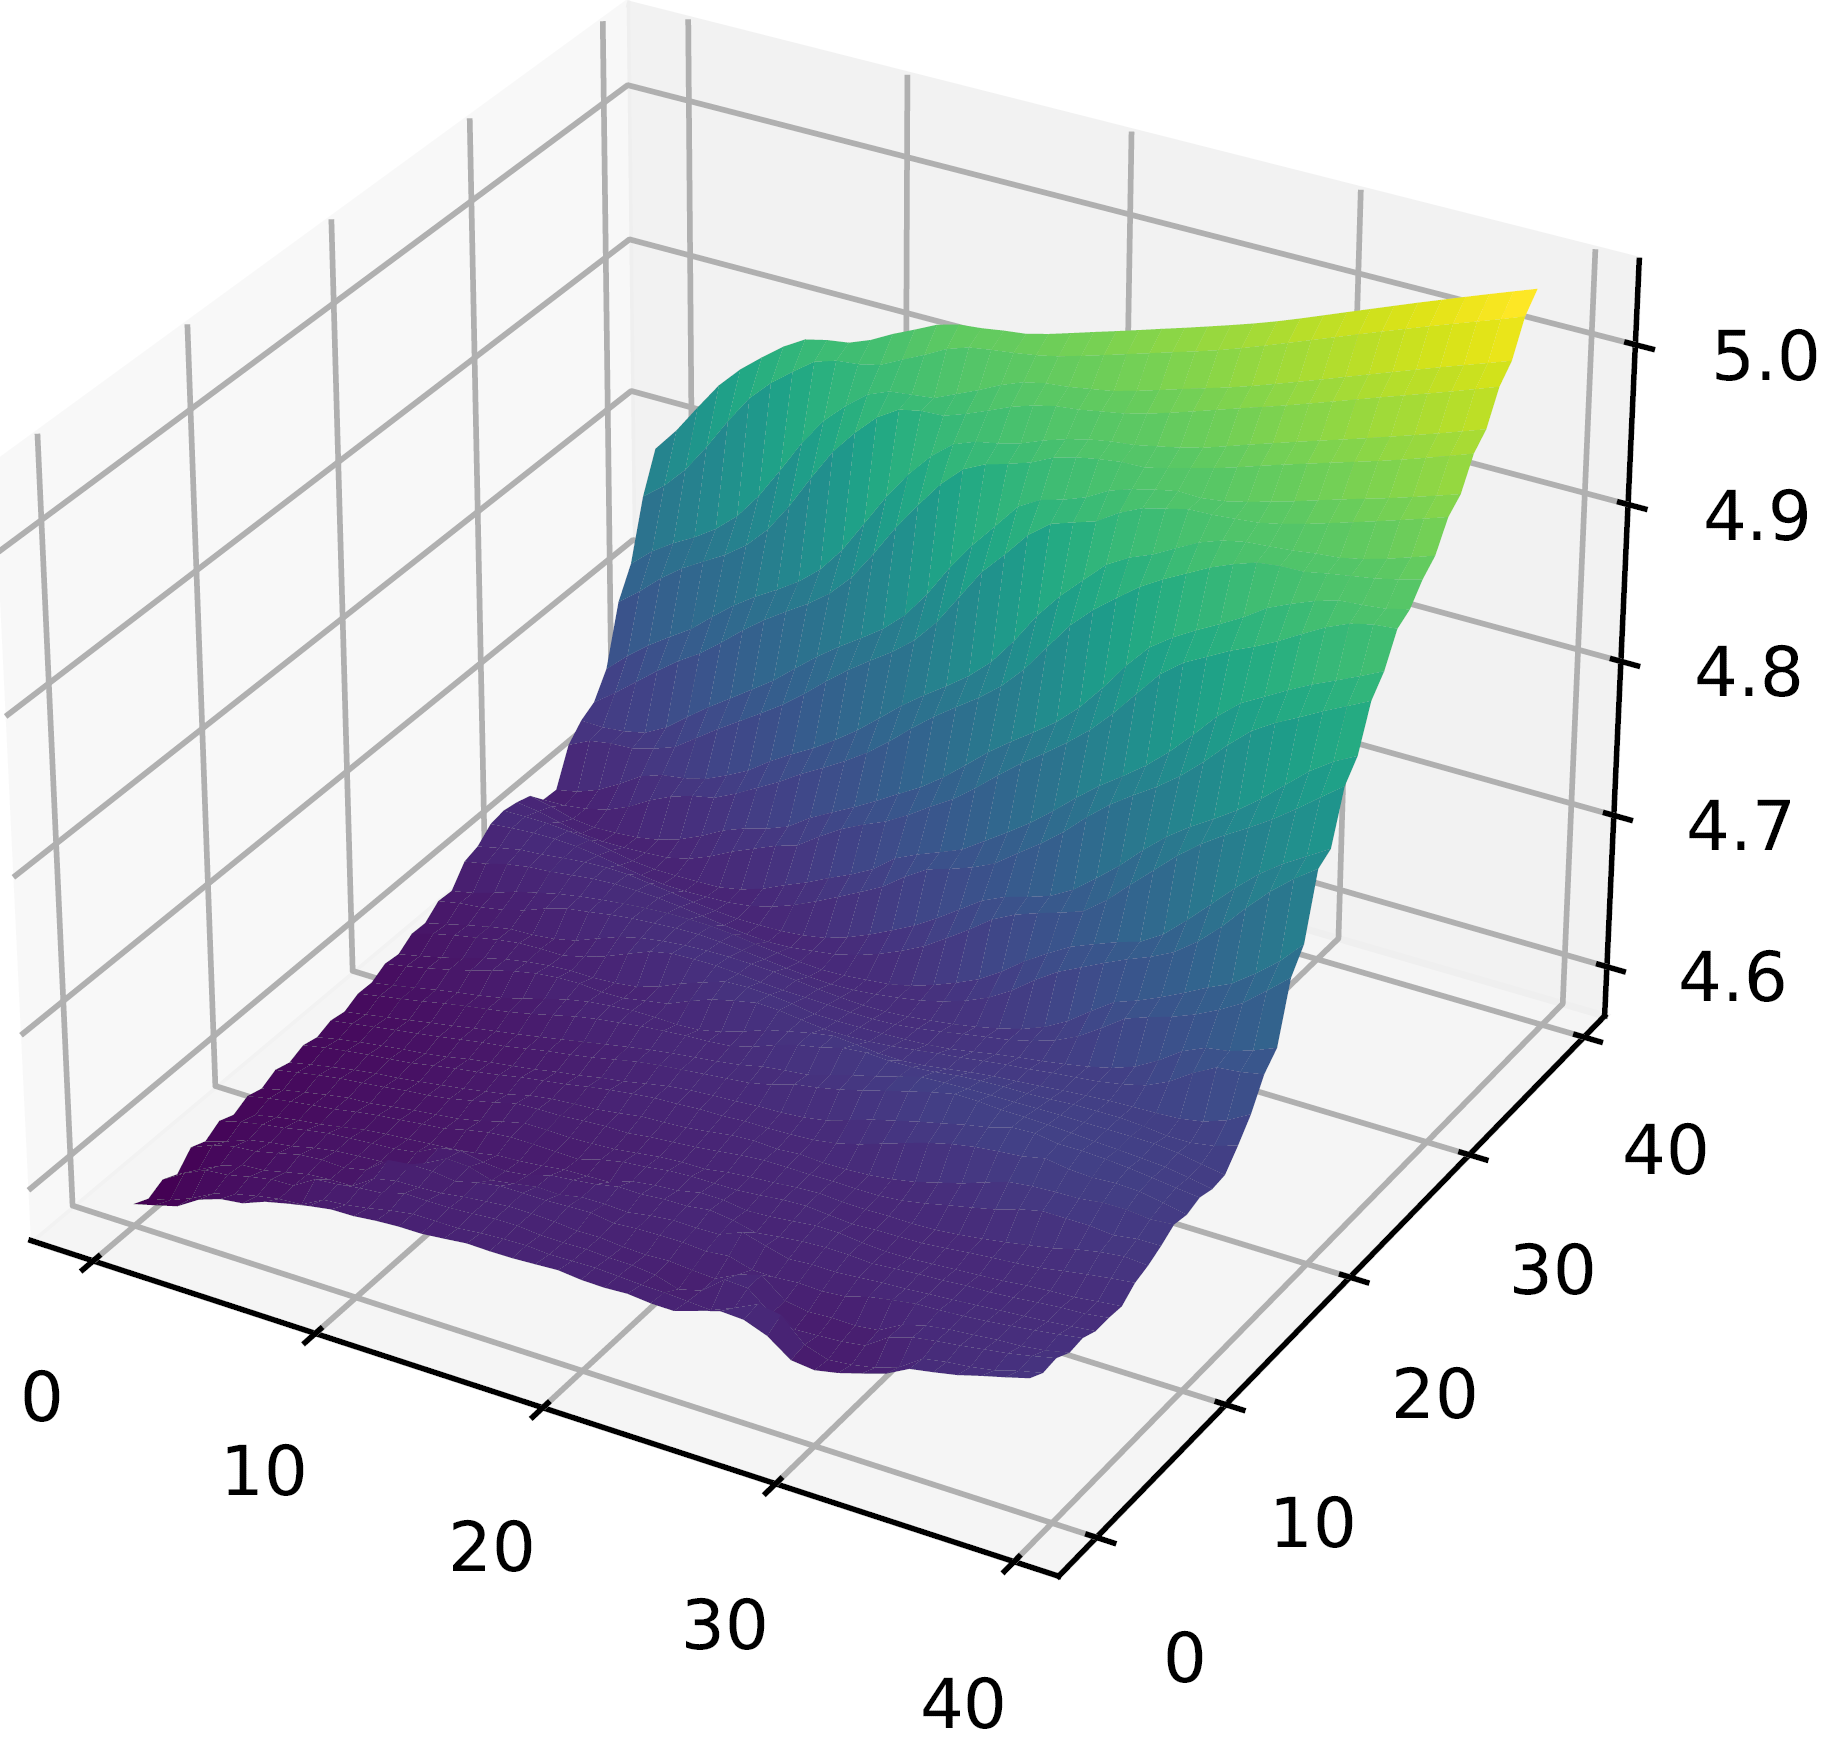} & \hspace{-0.15in}
    \includegraphics[width=0.16\textwidth]{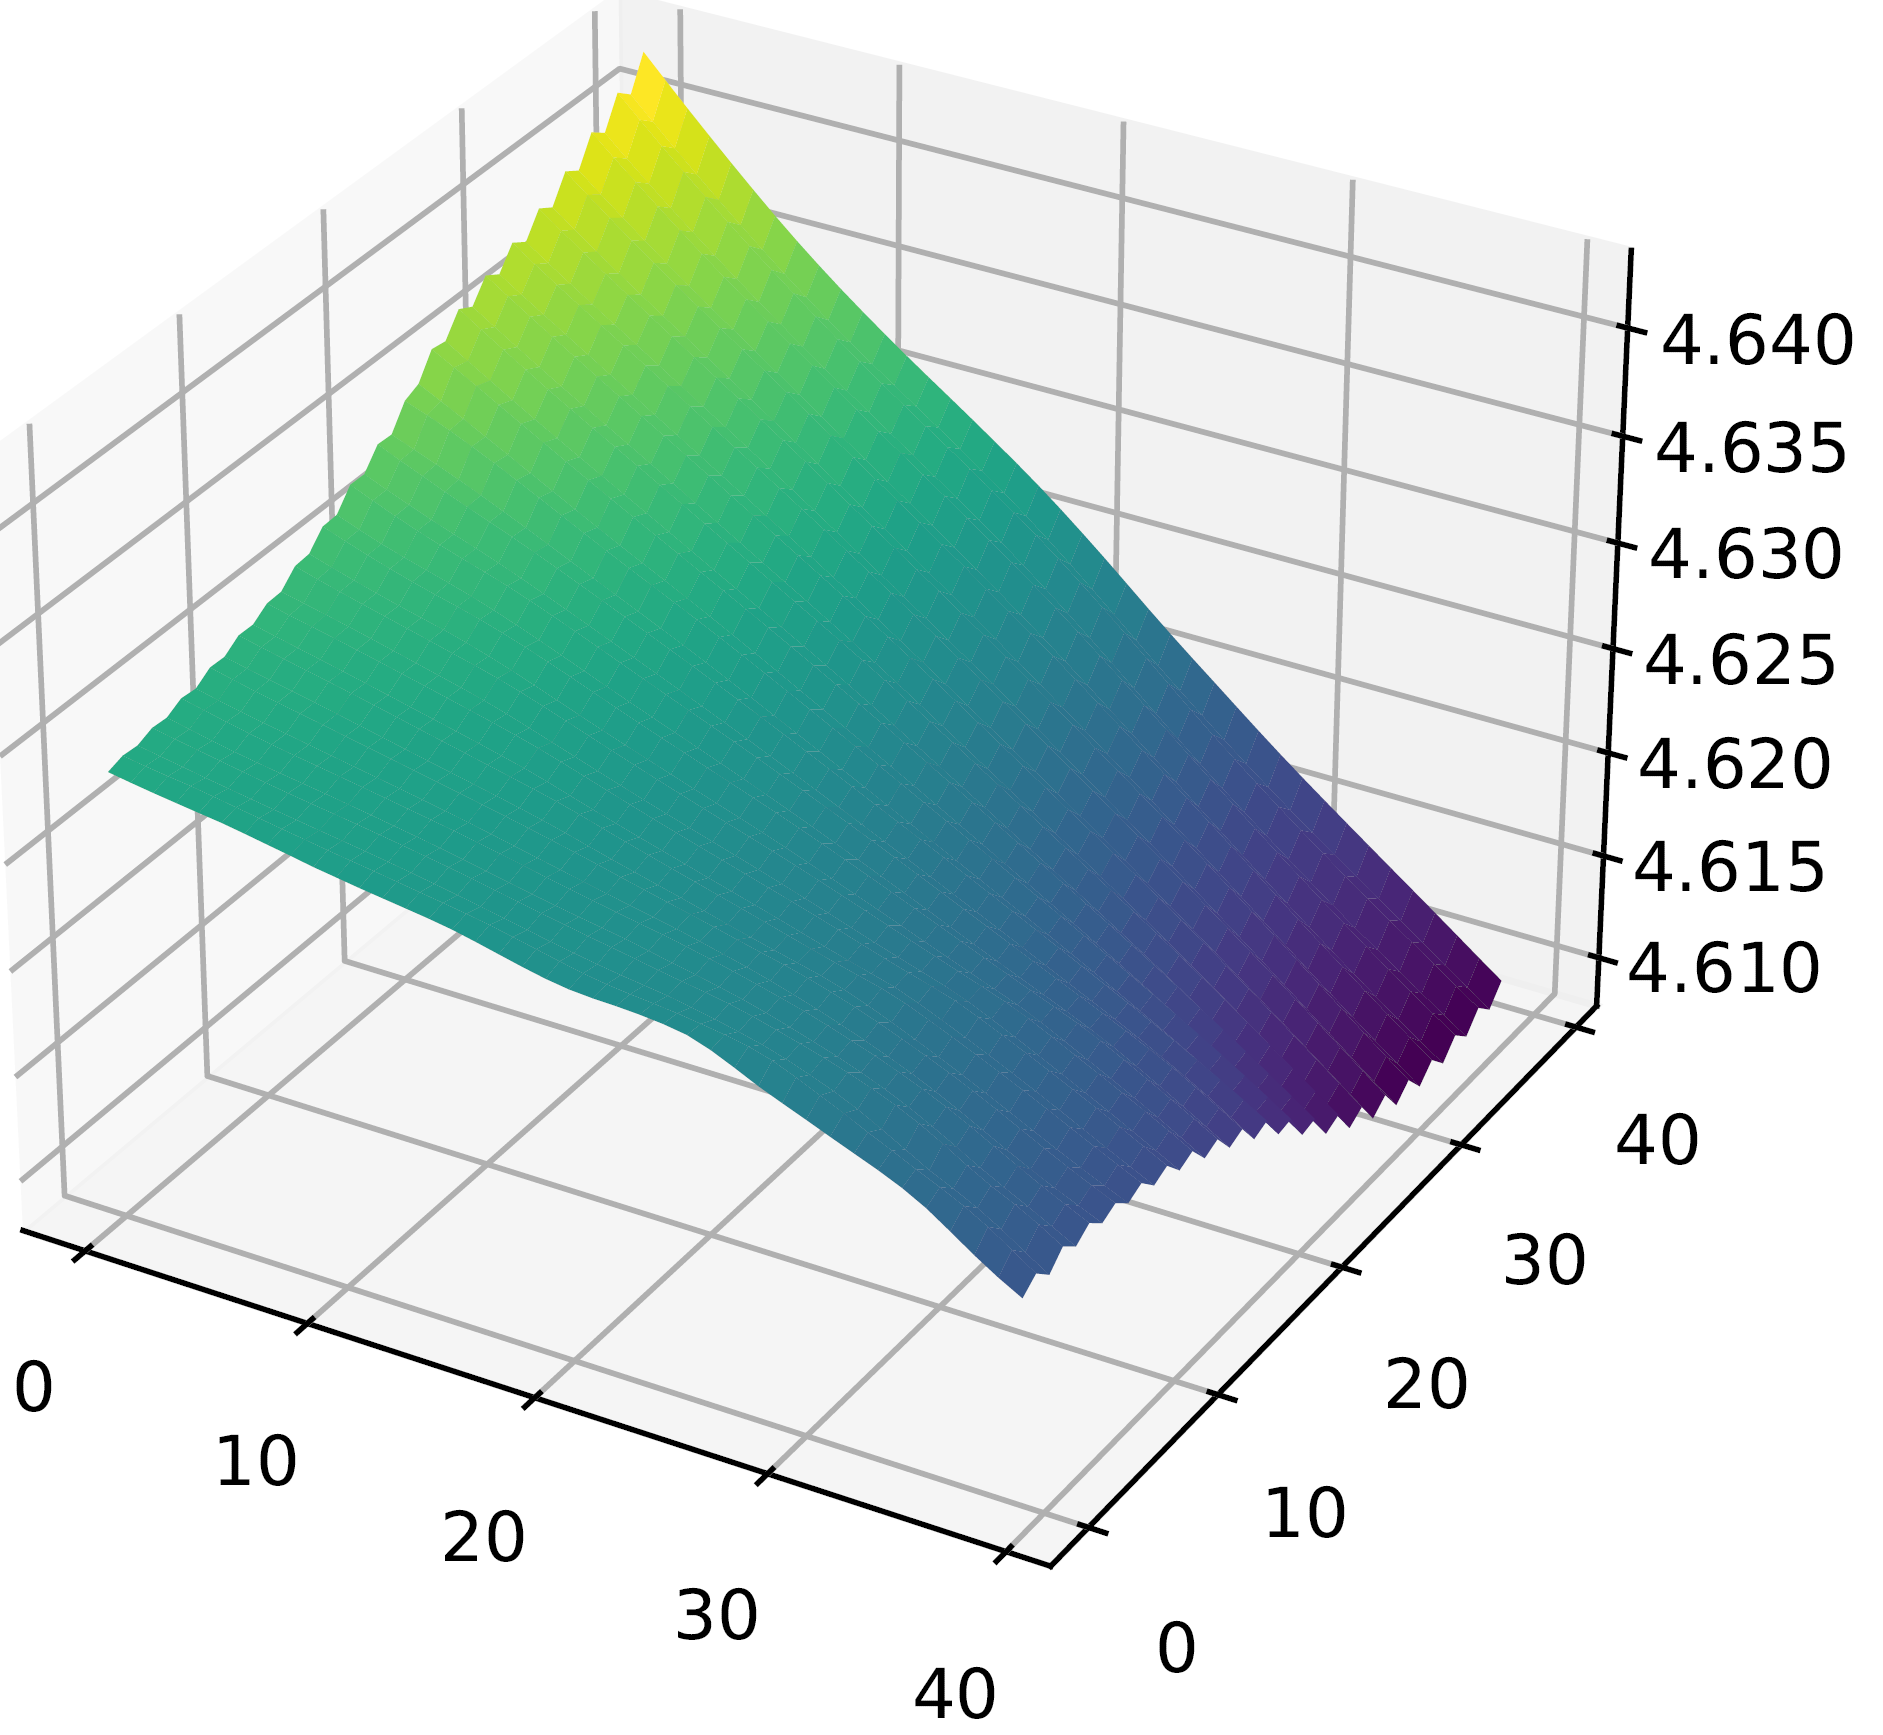} & \hspace{-0.15in}
    \includegraphics[width=0.16\textwidth]{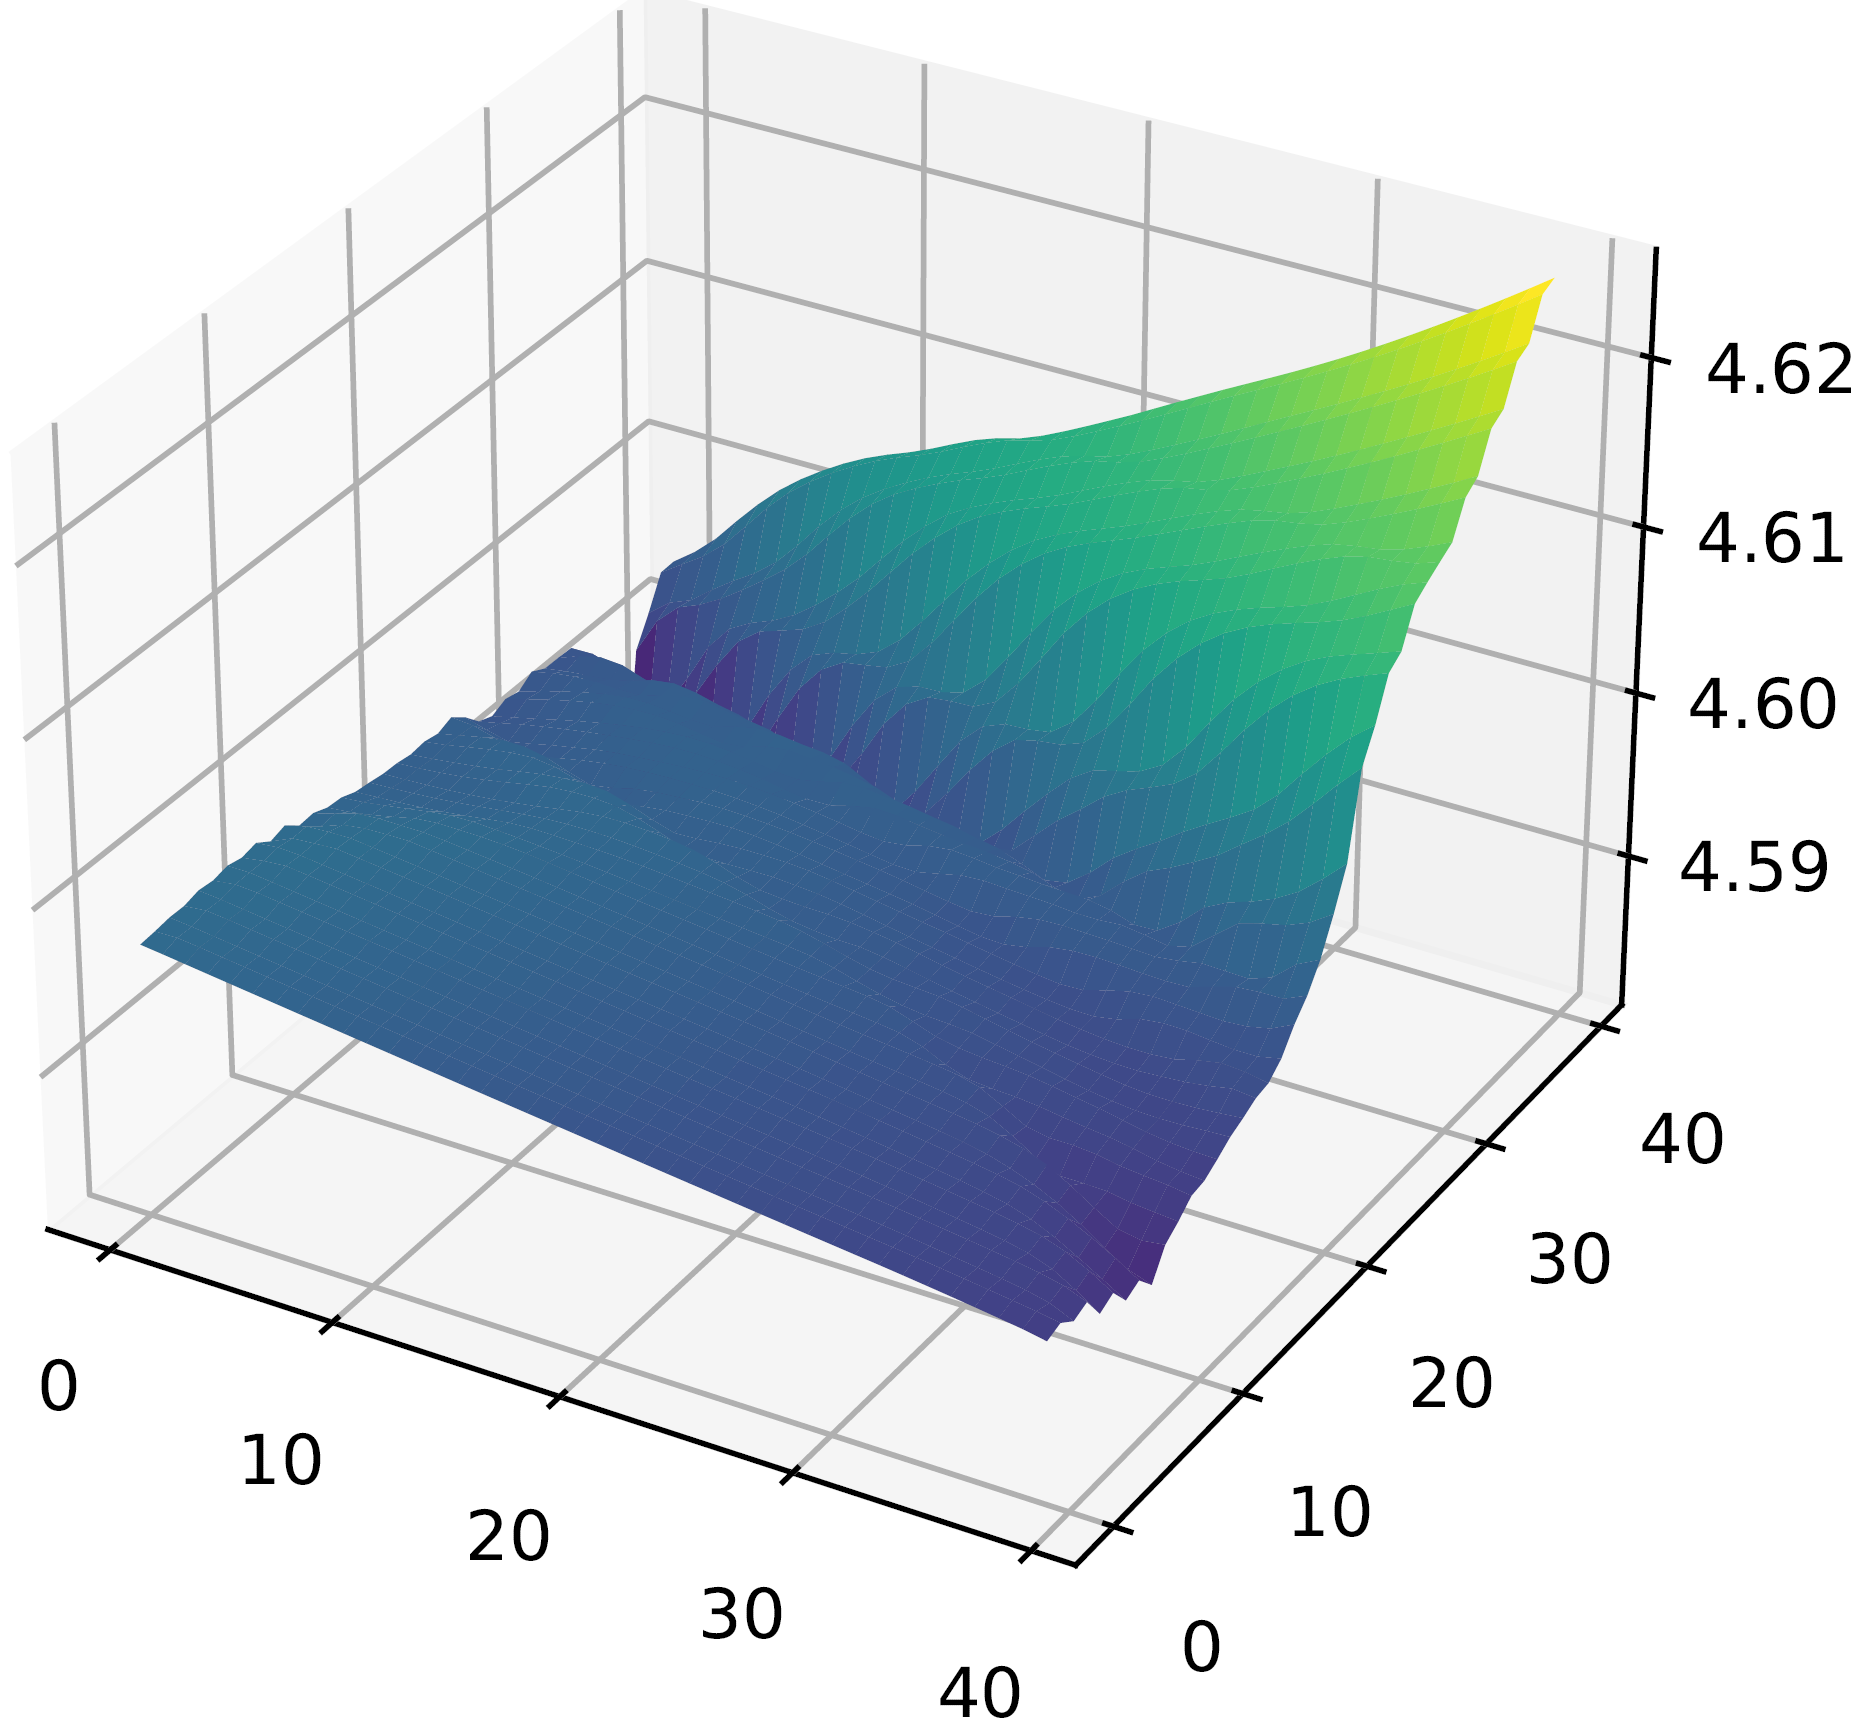} & \hspace{-0.15in} 
    \includegraphics[width=0.16\textwidth]{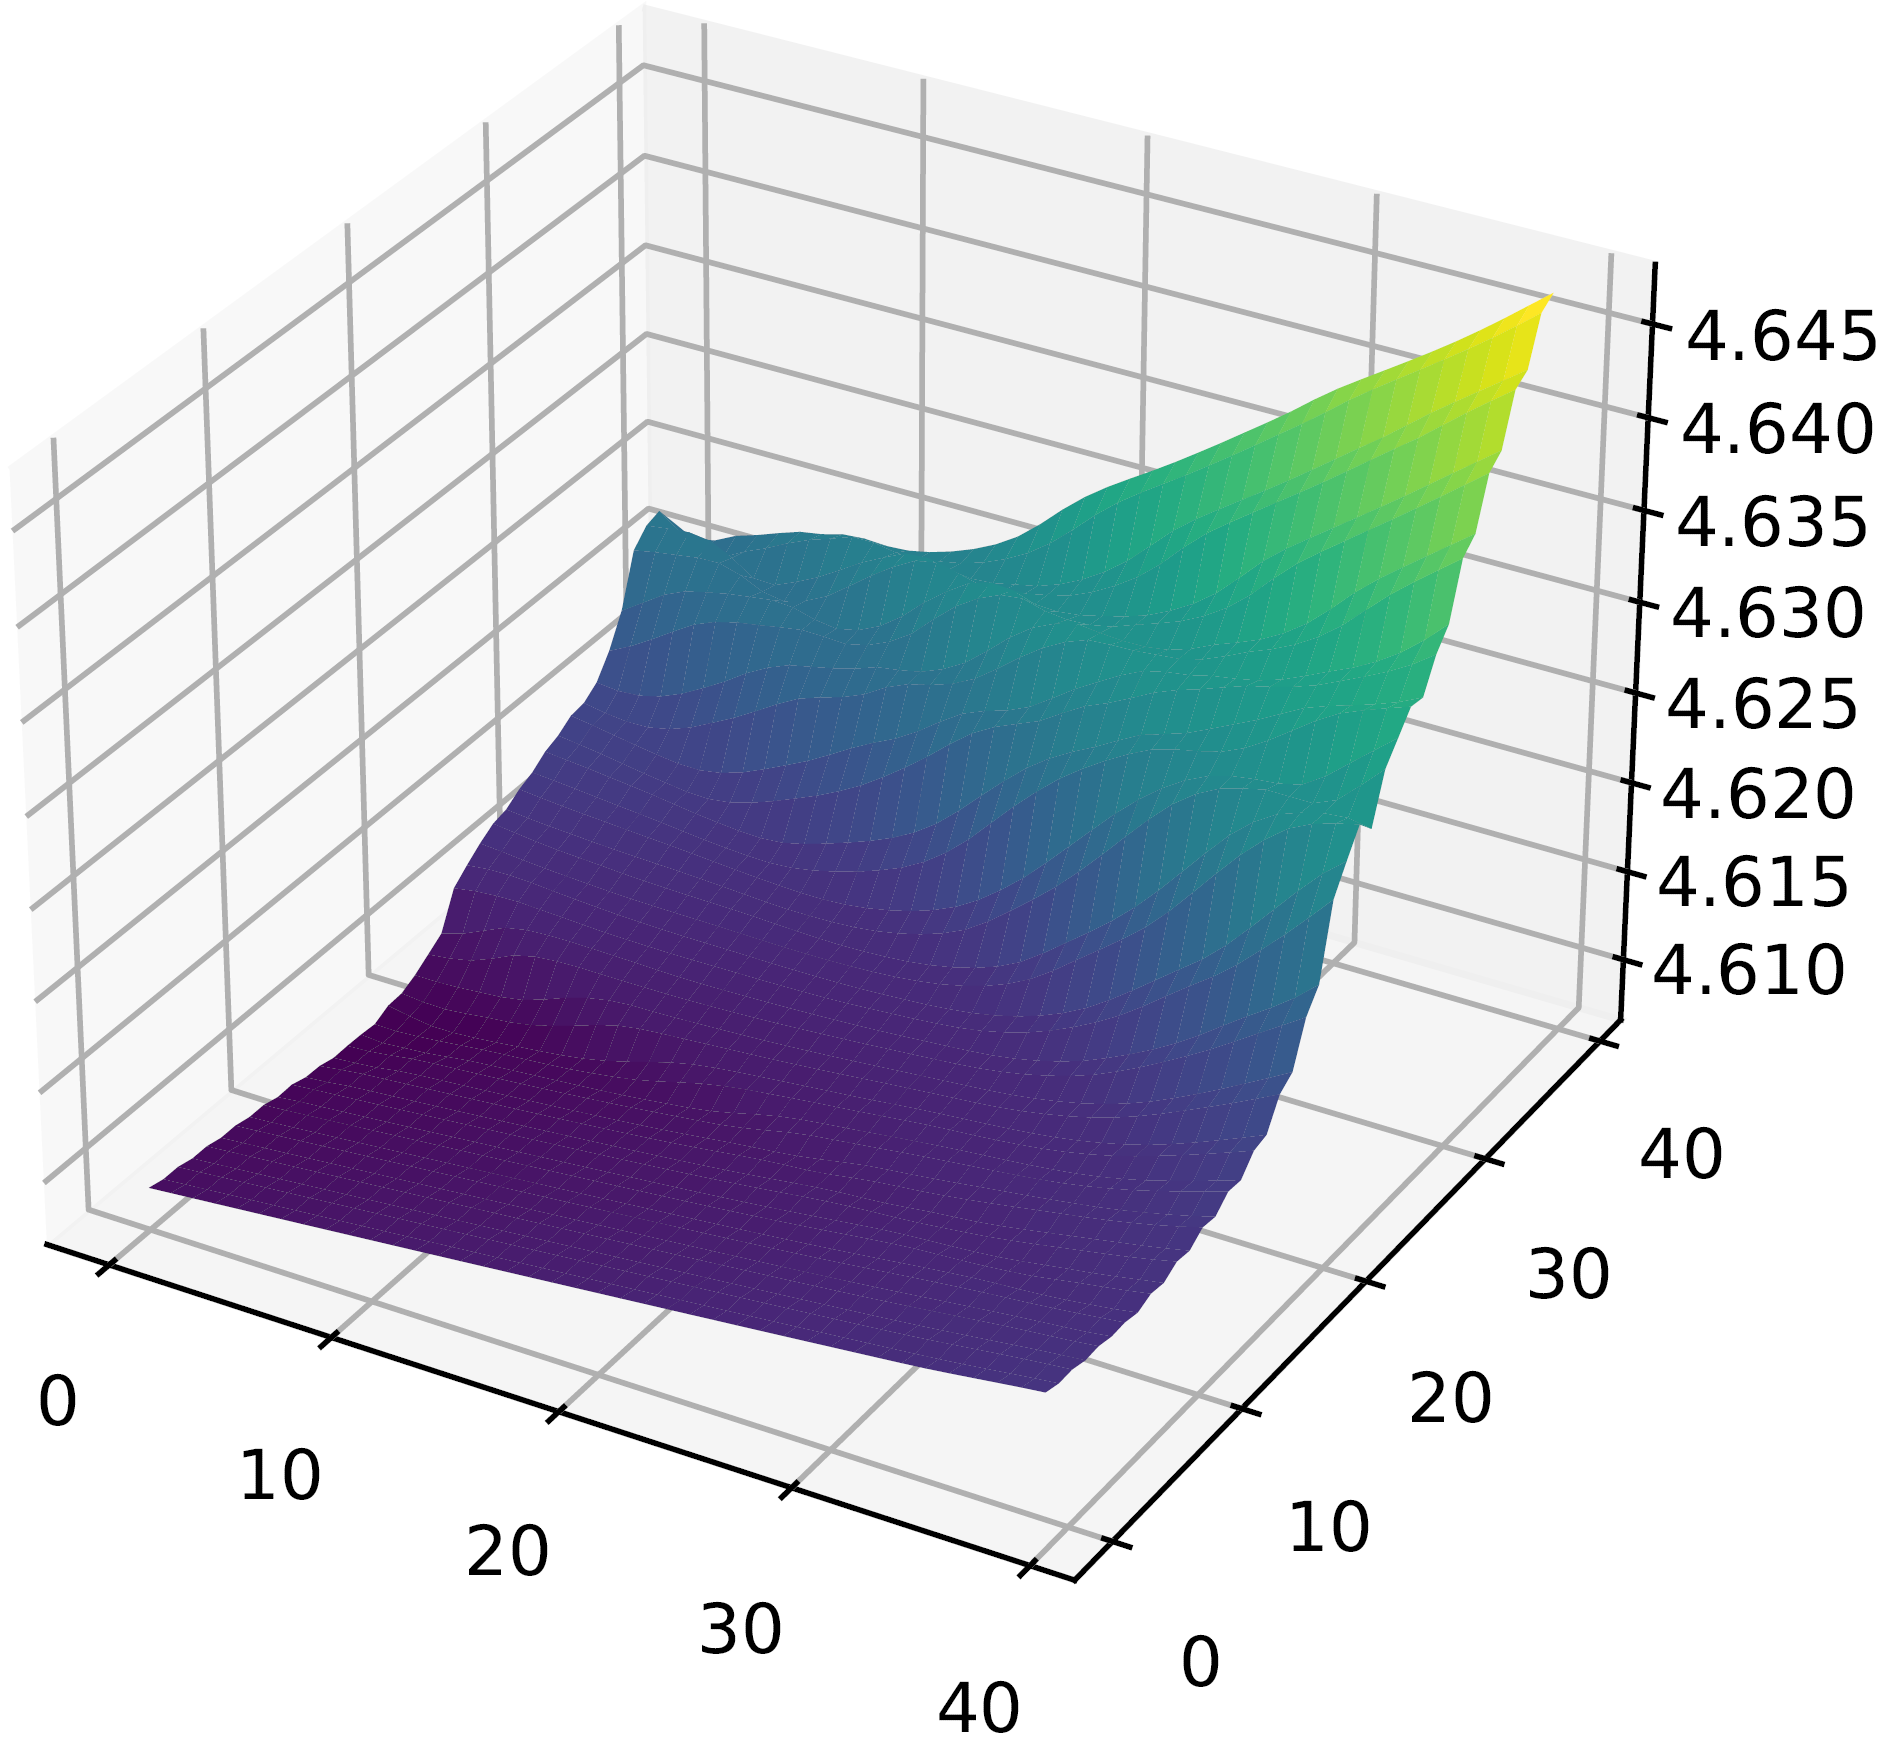} \\
\hspace{-0.15in}\rowlegend{~~~~$t=19$}    
    \includegraphics[width=0.16\textwidth]{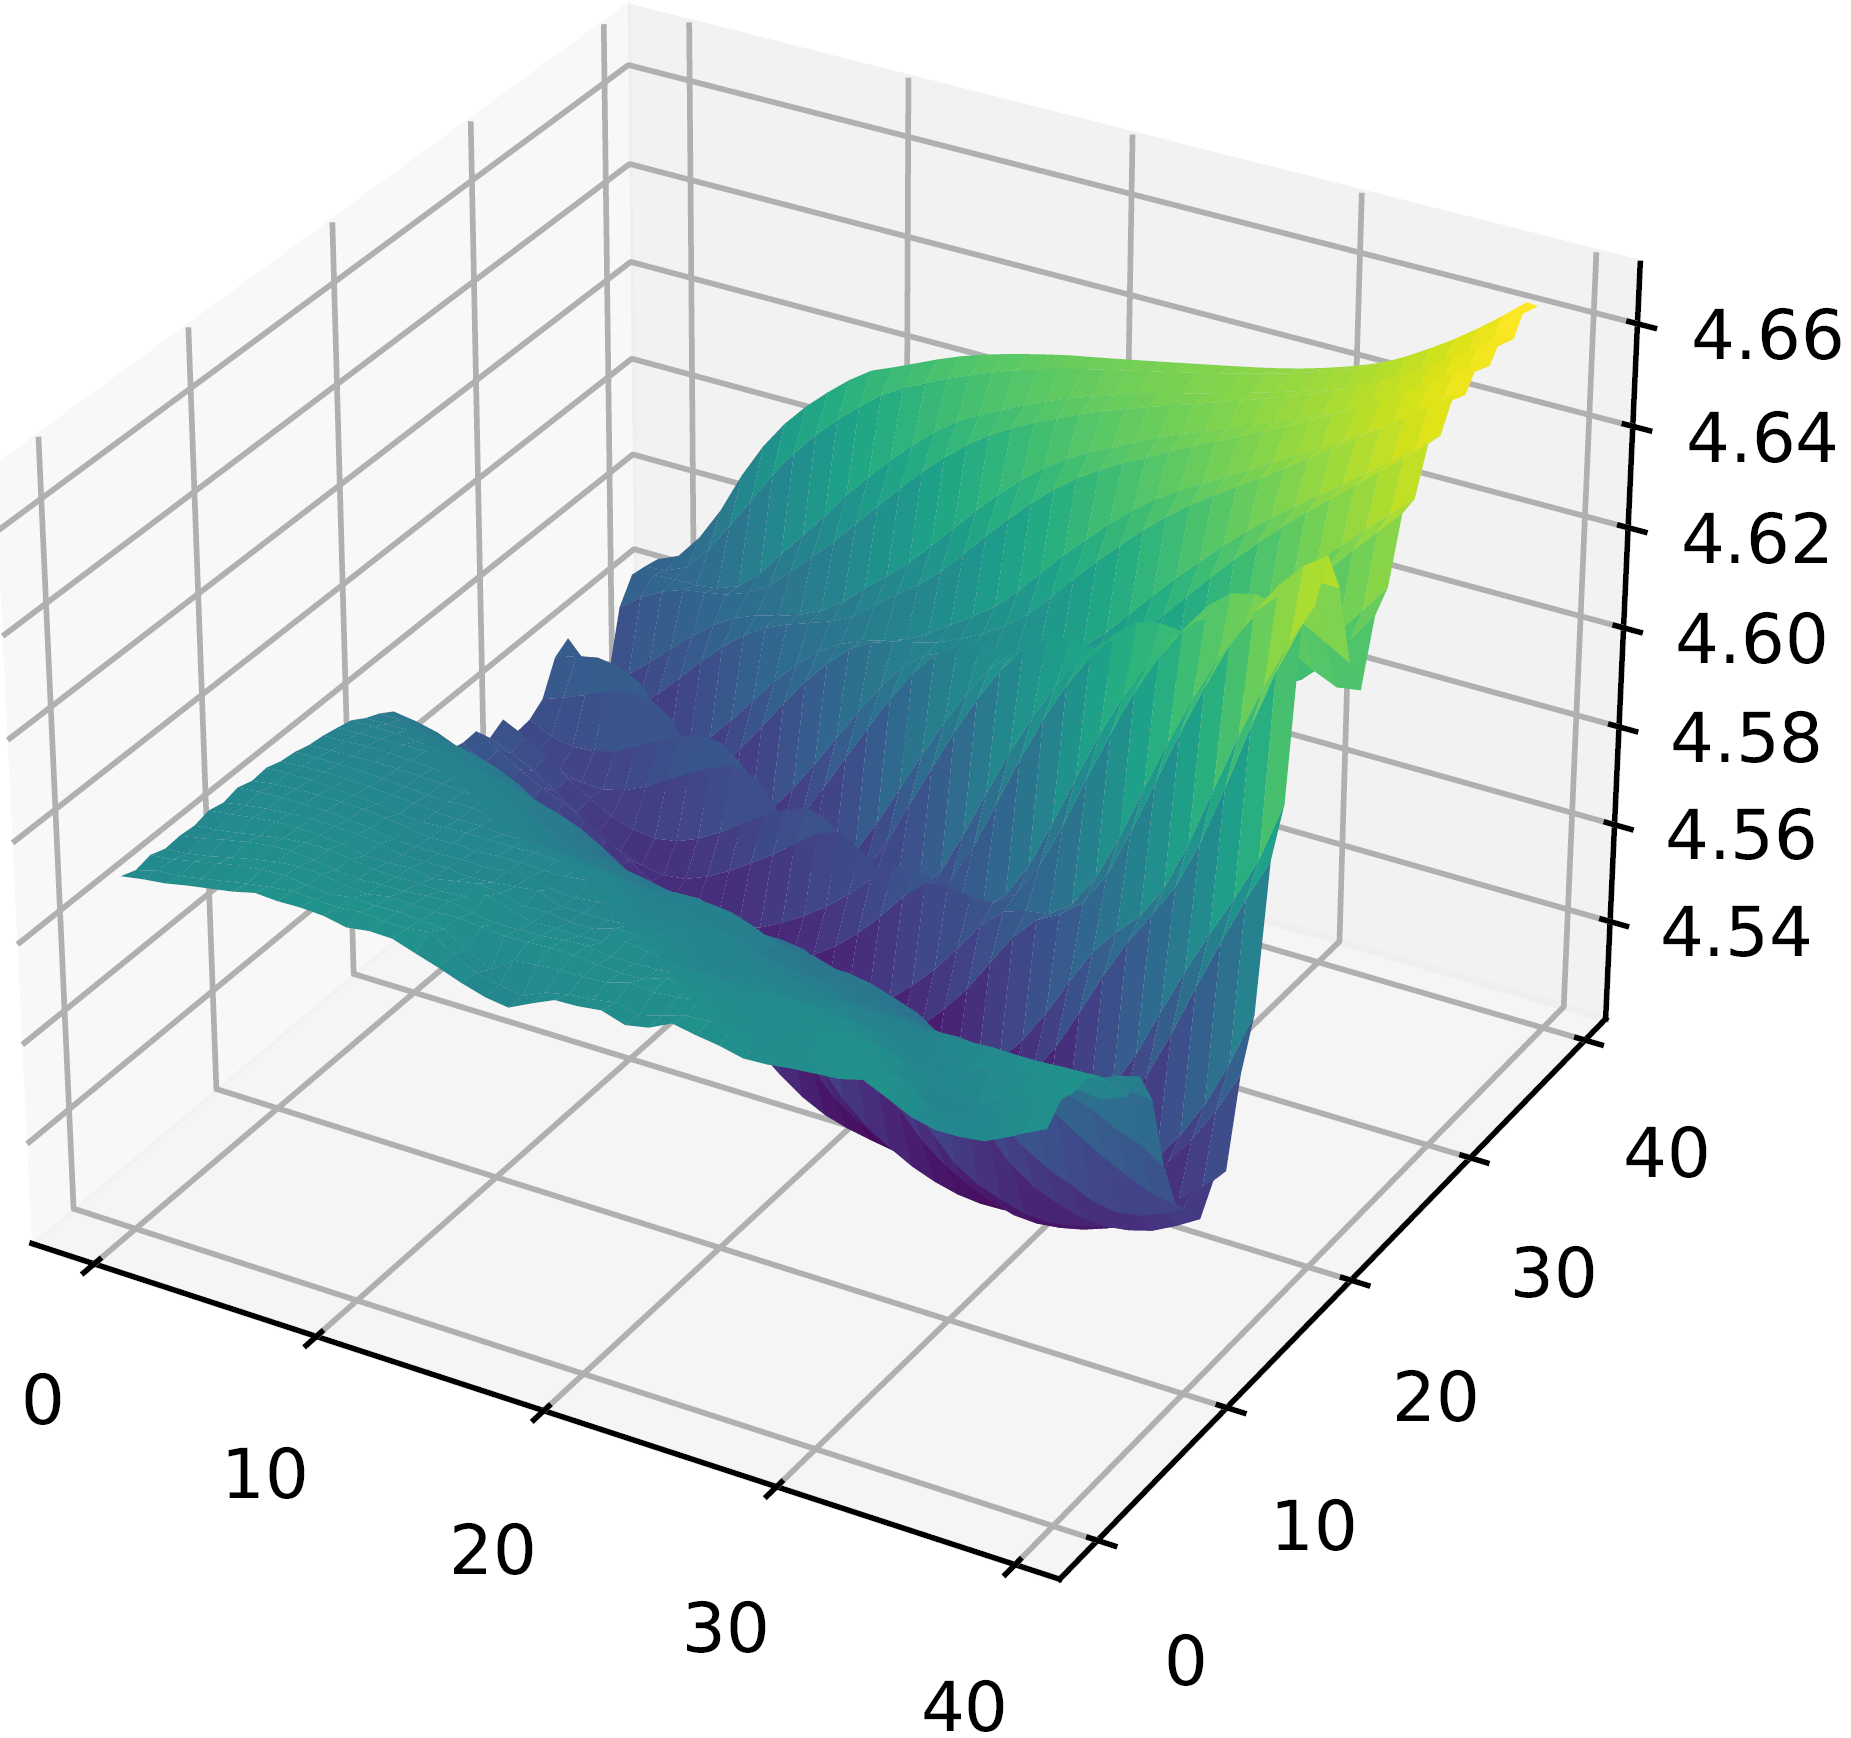} & \hspace{-0.15in}
    \includegraphics[width=0.16\textwidth]{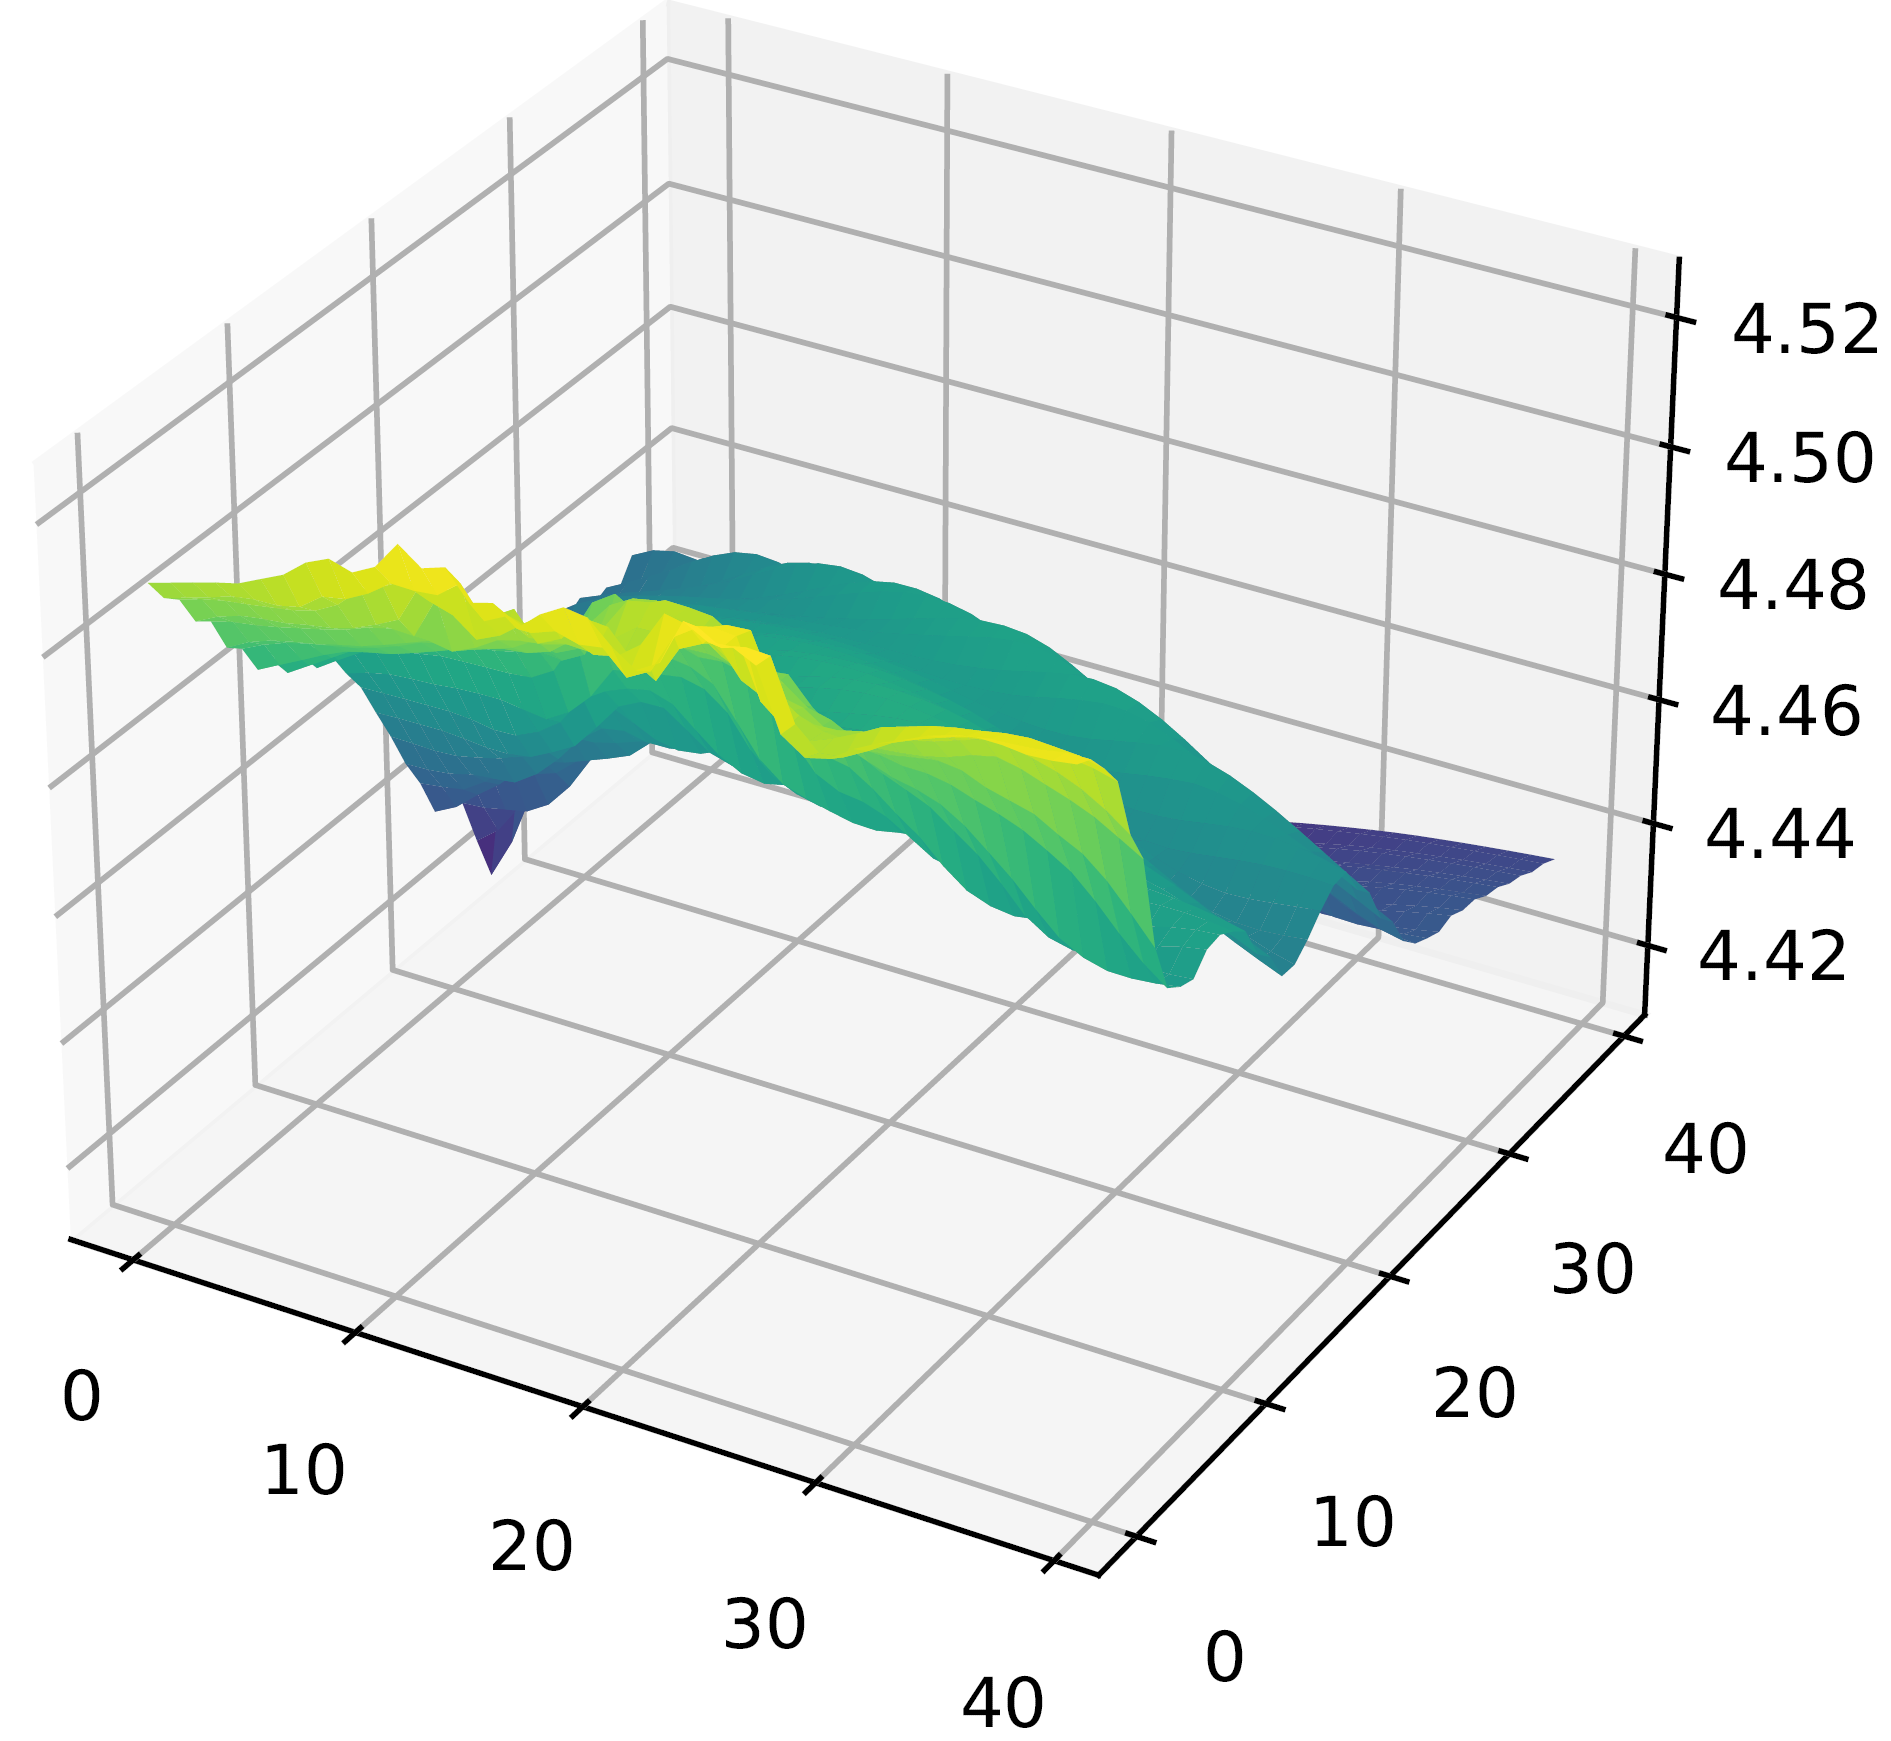} & \hspace{-0.15in}
    \includegraphics[width=0.16\textwidth]{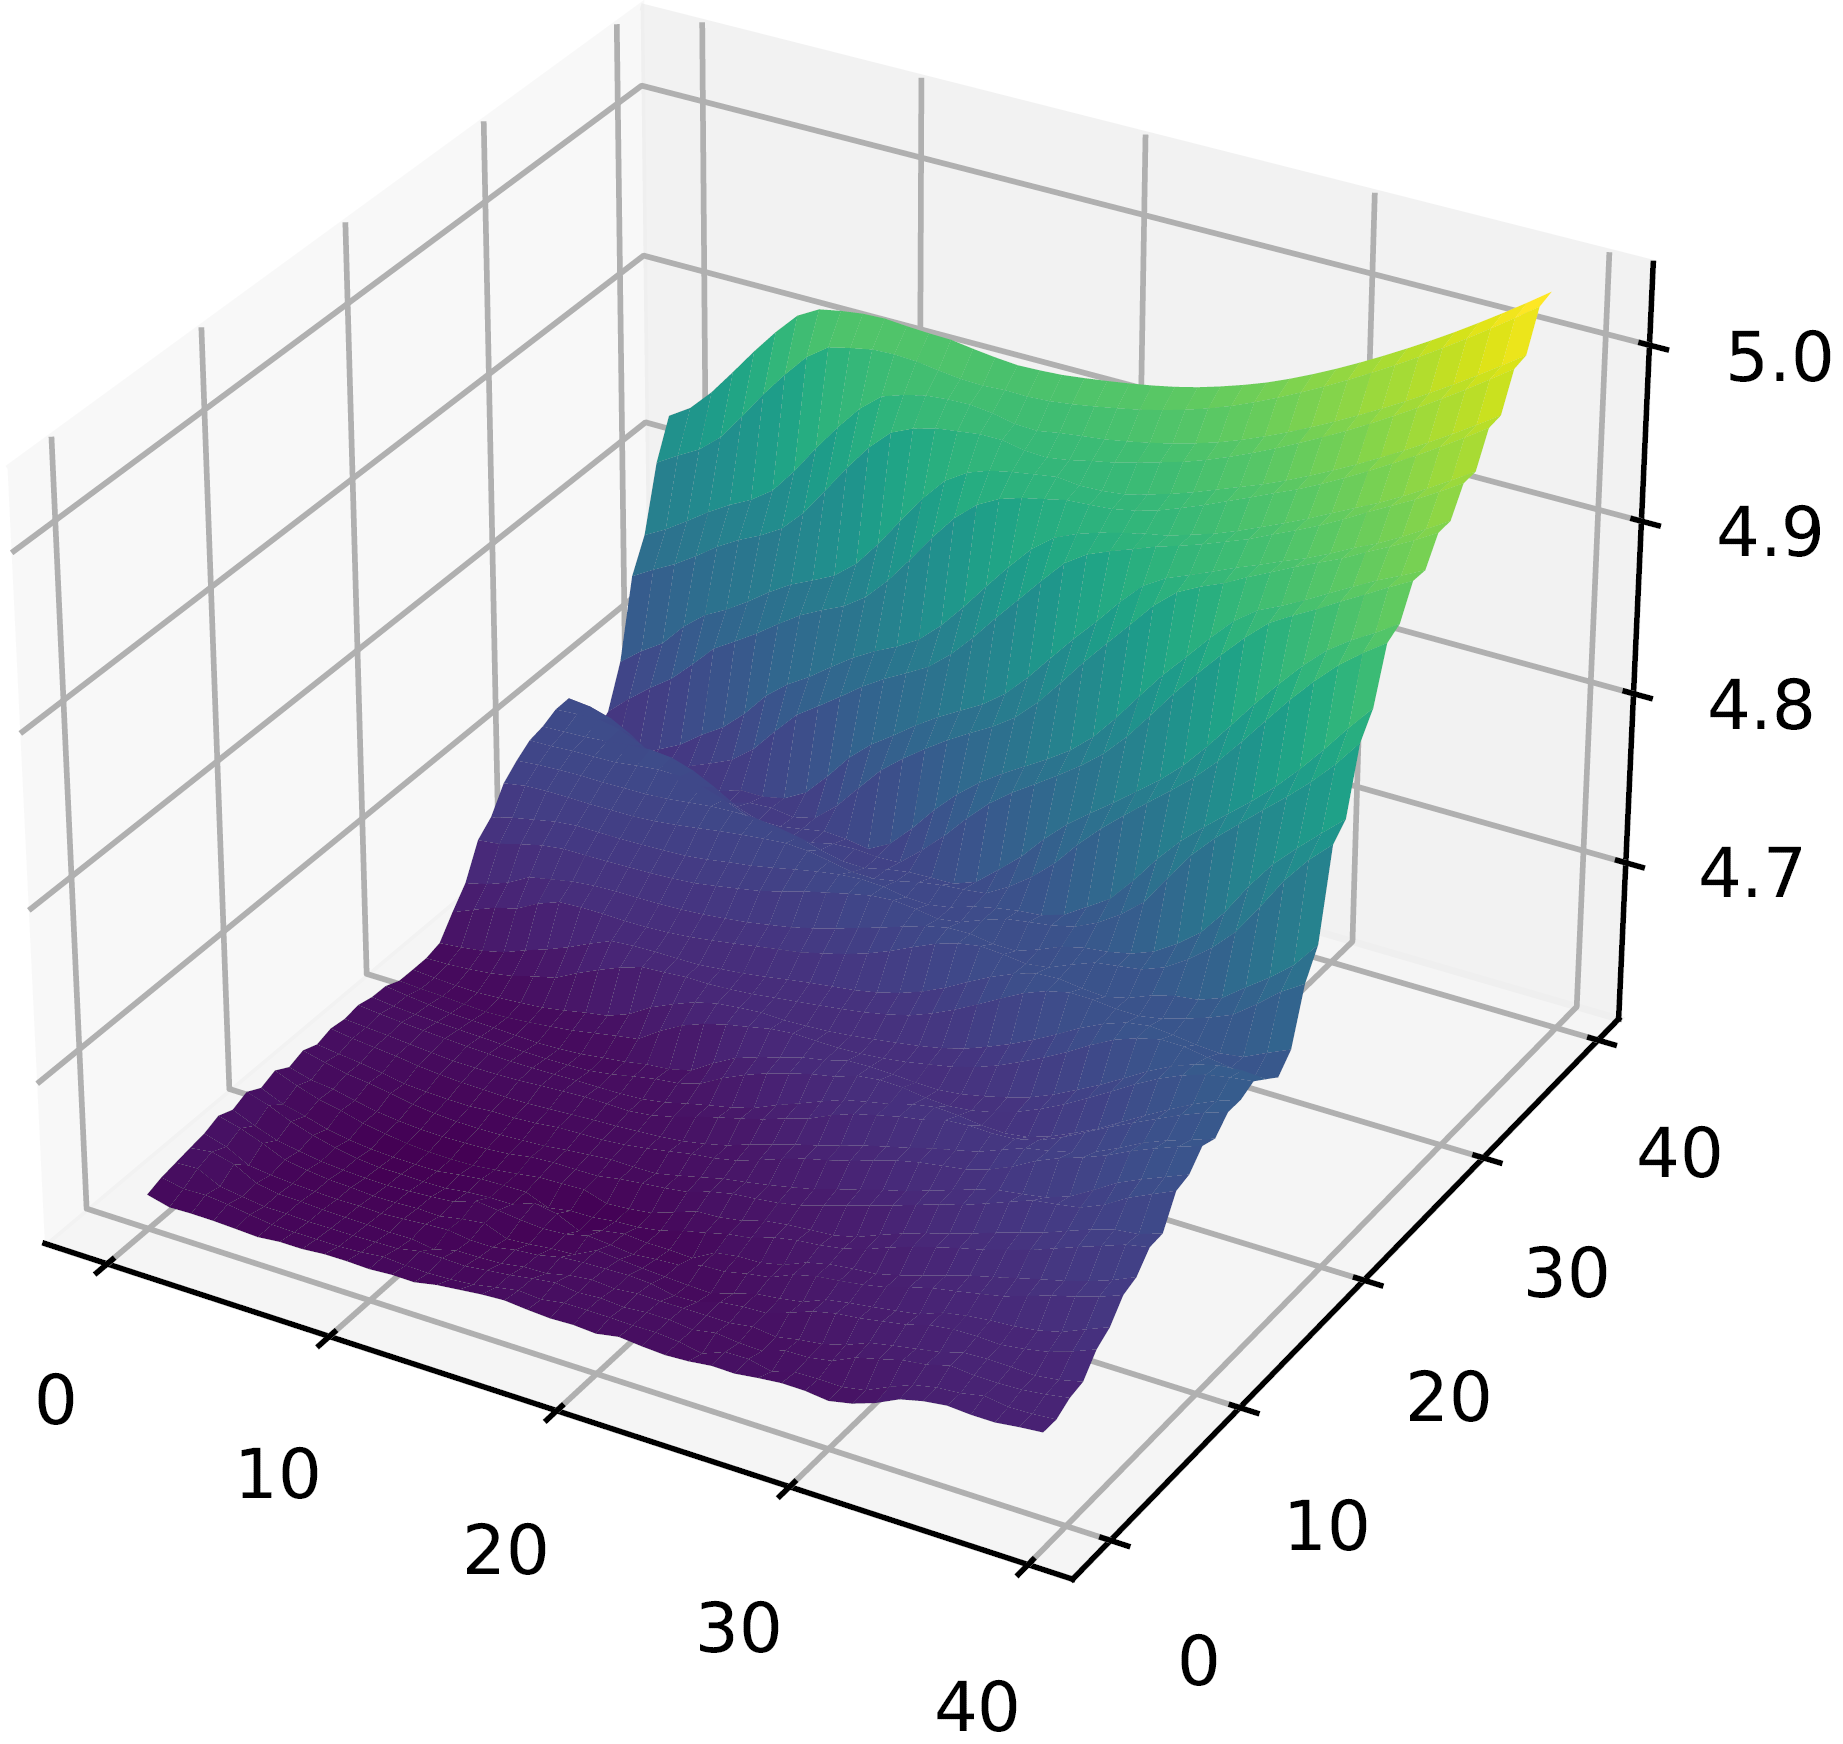} & \hspace{-0.15in}
    \includegraphics[width=0.16\textwidth]{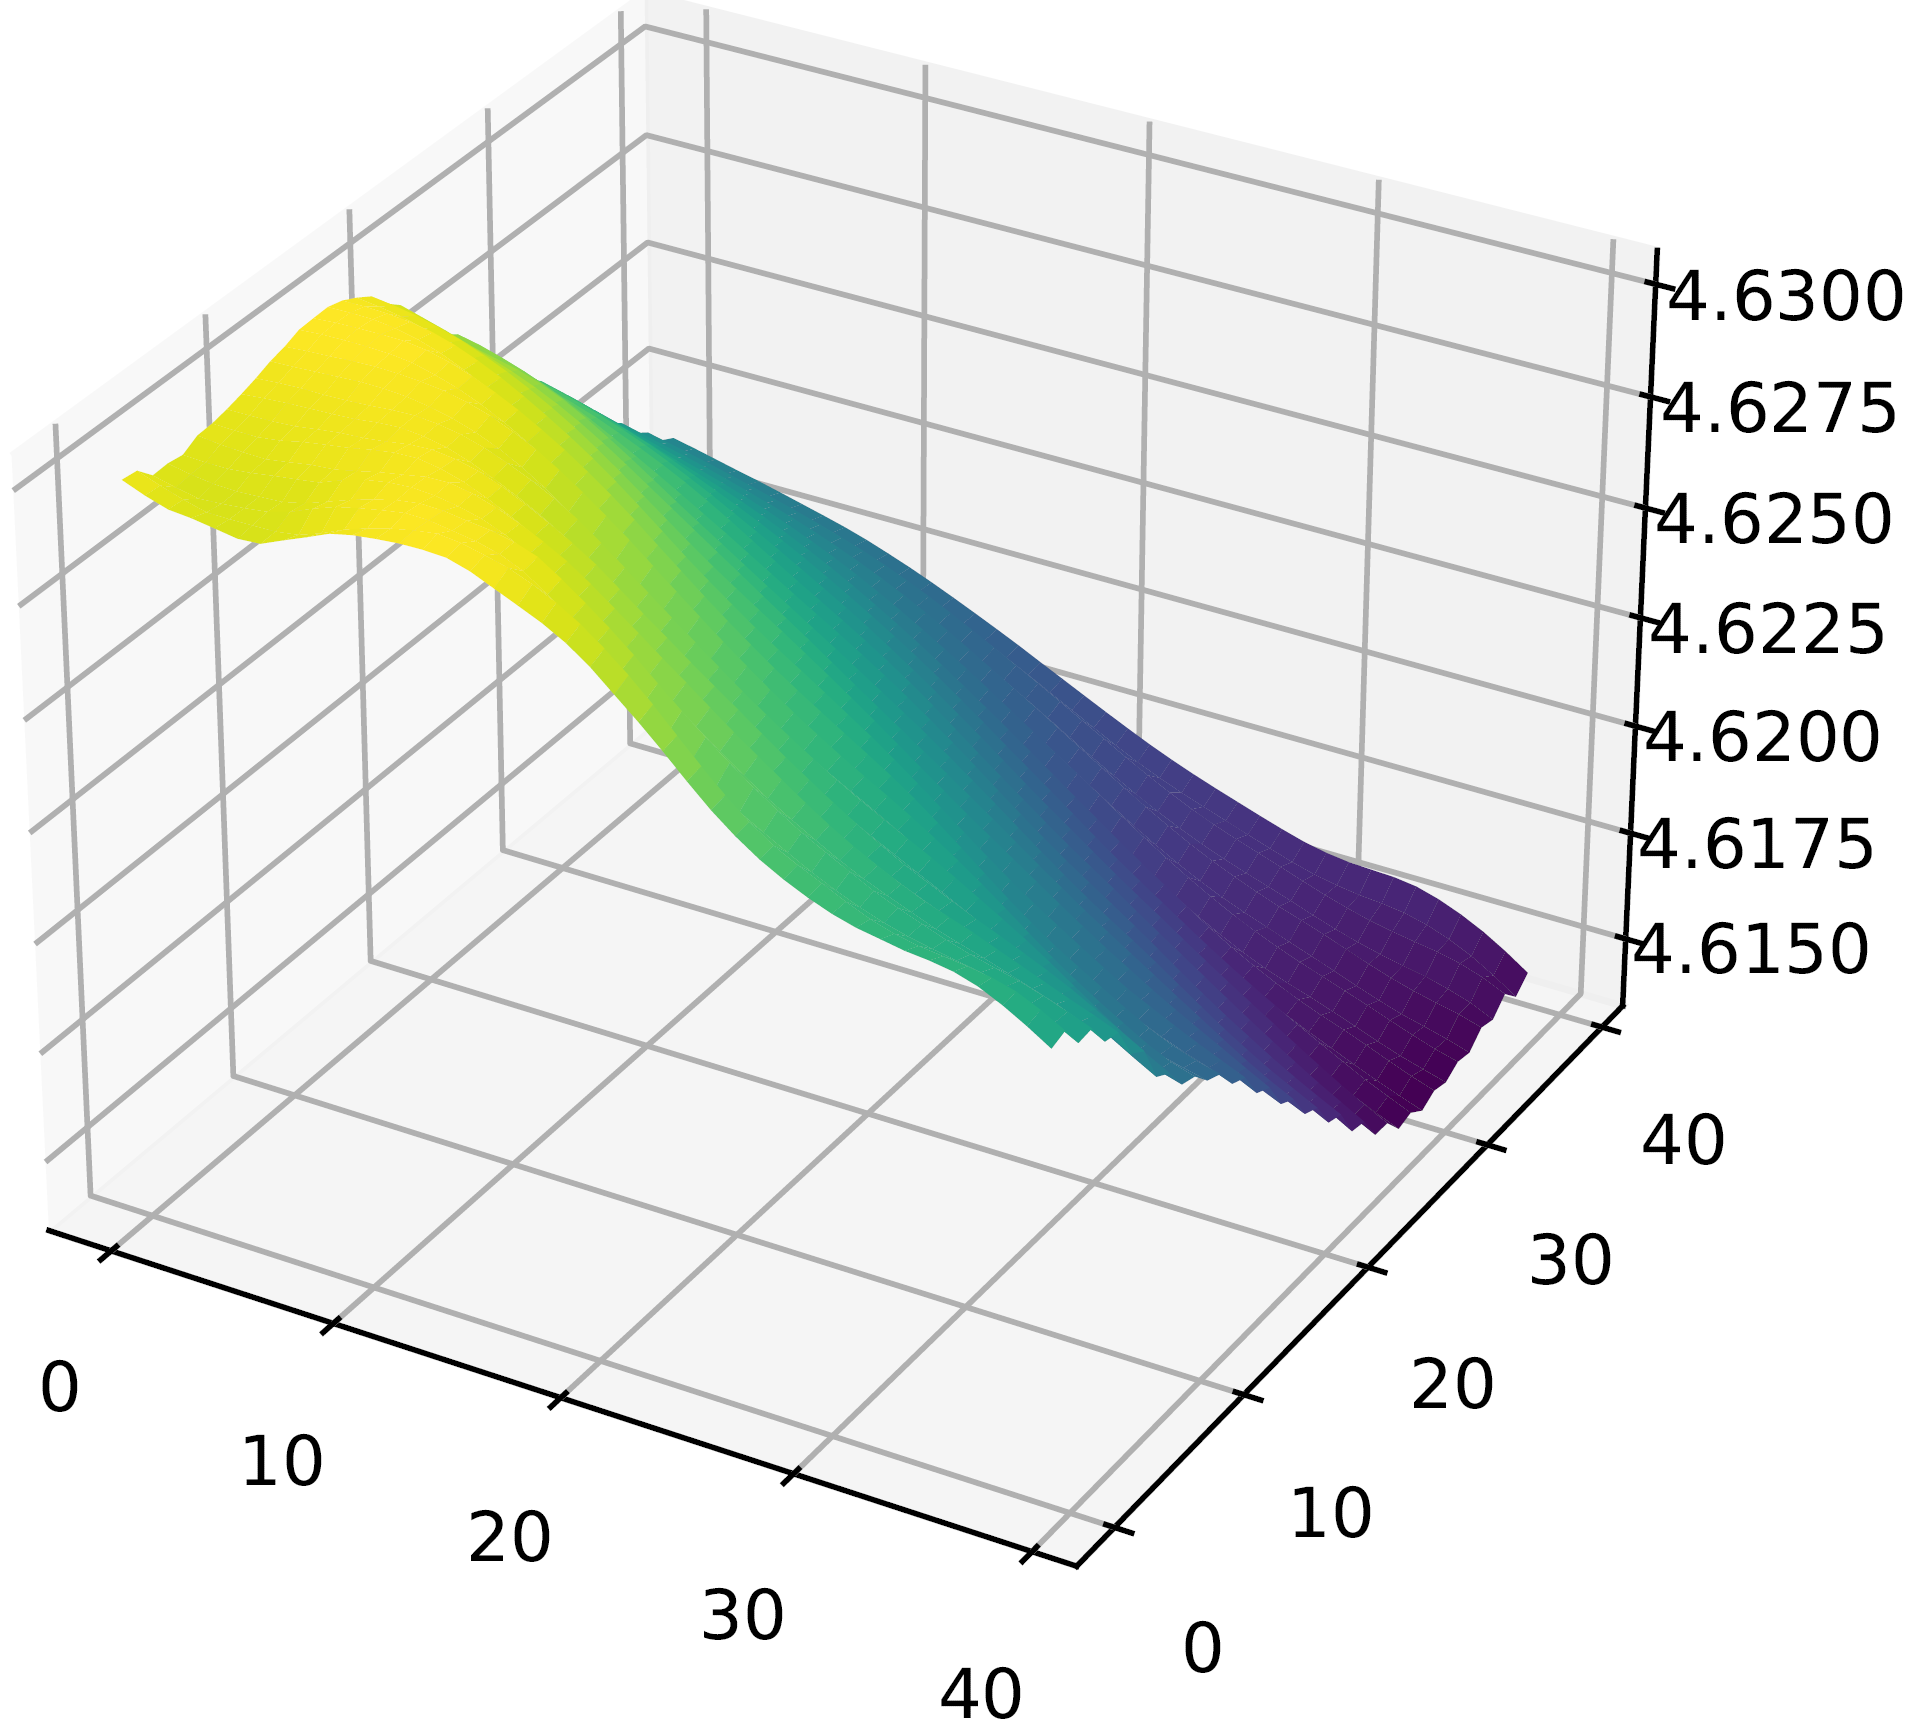} & \hspace{-0.15in}
    \includegraphics[width=0.16\textwidth]{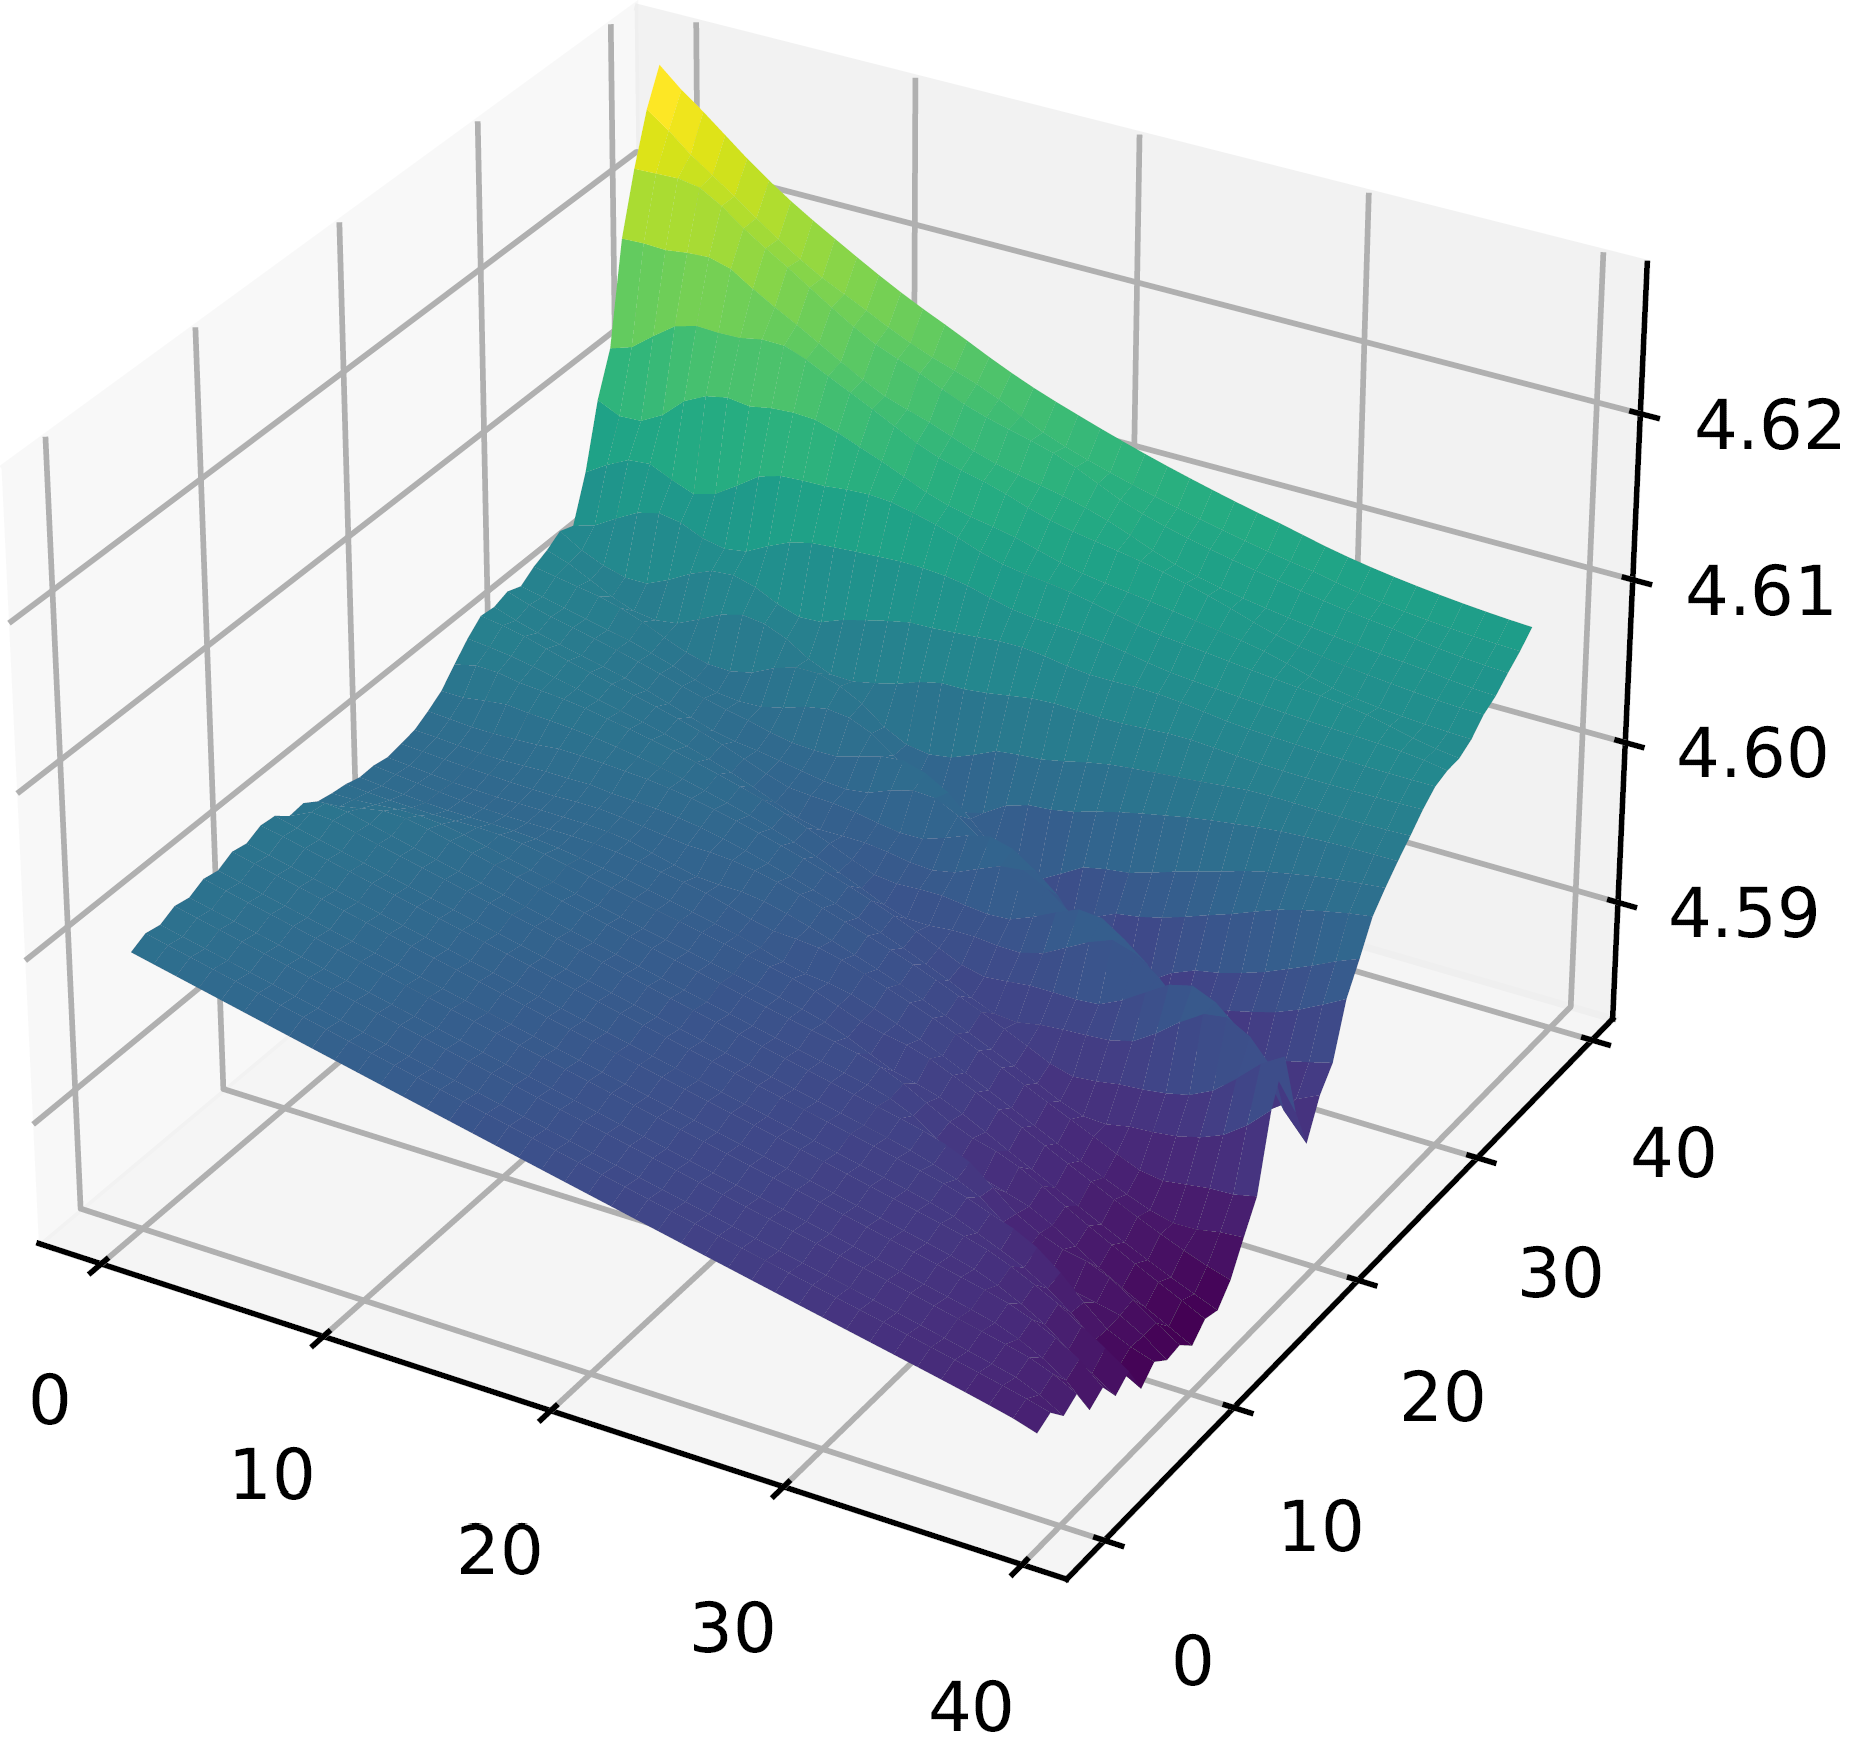} & \hspace{-0.15in}
    \includegraphics[width=0.16\textwidth]{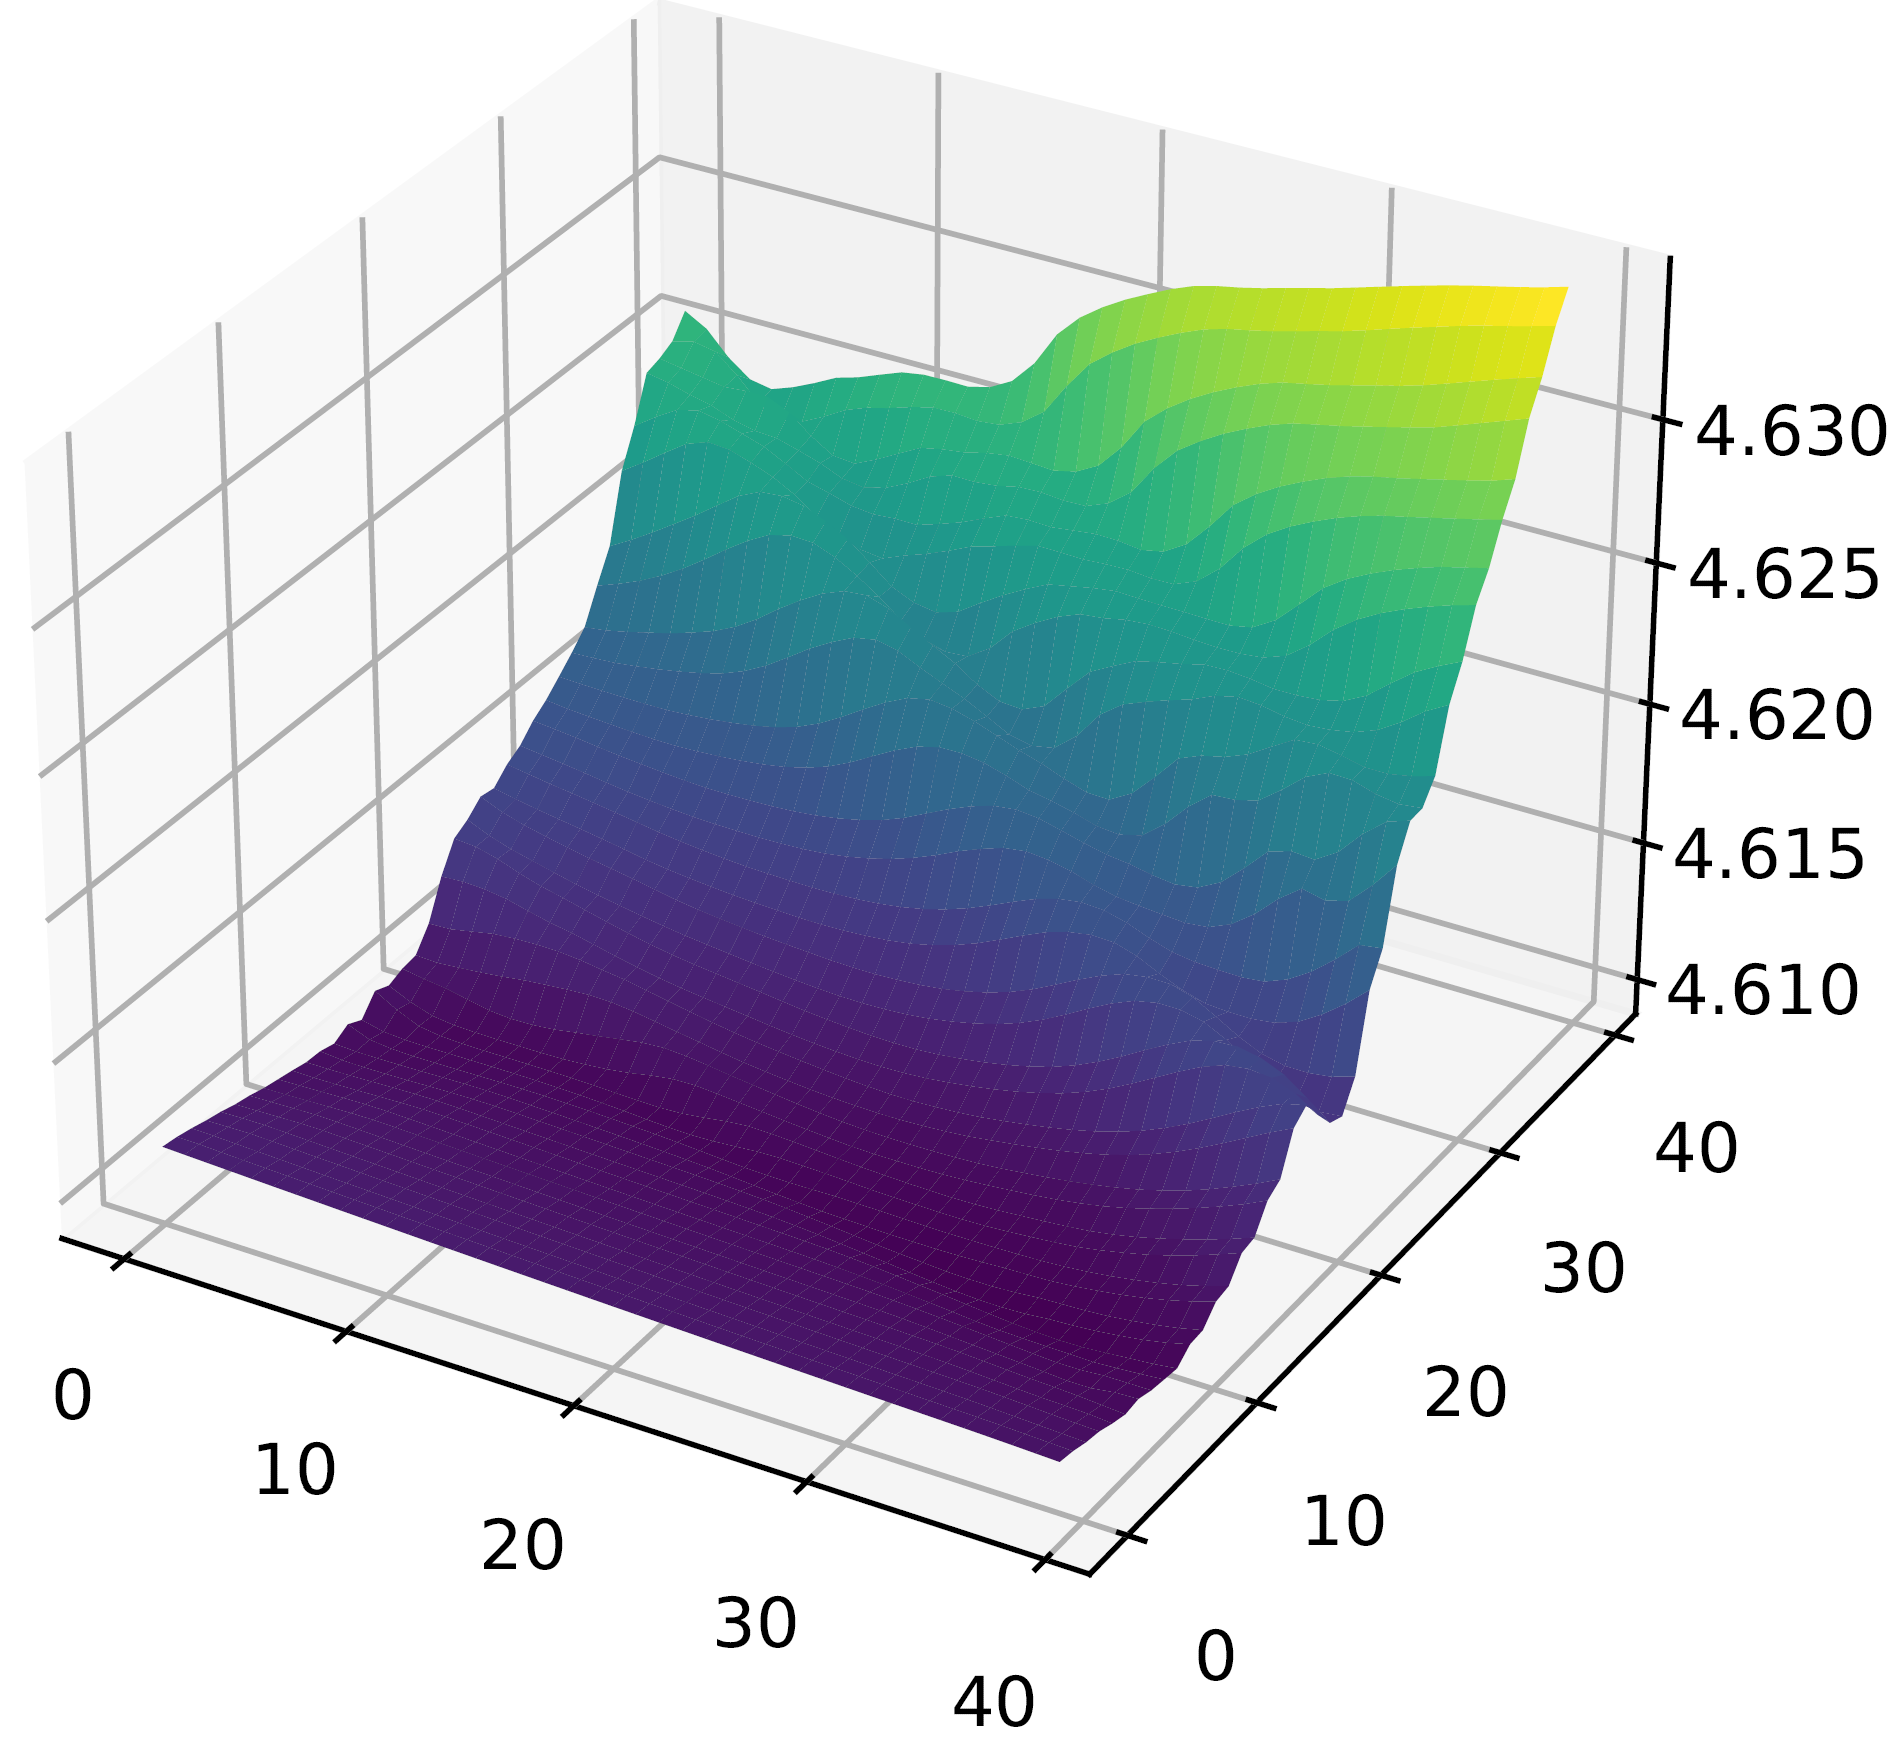} \\
%\vspace{-0.15in}
\hspace{-0.15in}\specialcell{\textsc{Scl-Finetune}\\{\scriptsize Acc:$00.00\pm 0.00$}} & \hspace{-0.15in} \specialcell{\textsc{Scl-Si}\\{\scriptsize Acc:$00.00\pm 0.00$}} & \hspace{-0.15in} \specialcell{\textsc{Scl-Der}\\{\scriptsize Acc:$00.00\pm 0.00$}} & \hspace{-0.15in}
\specialcell{\textsc{Ucl-Finetune}\\{\scriptsize Acc:$00.00\pm 0.00$}} & \hspace{-0.15in} \specialcell{\textsc{Ucl-Si}\\{\scriptsize Acc:$00.00\pm 0.00$}} &  \hspace{-0.15in} 
\specialcell{\textsc{Lump (Ours)}\\{\scriptsize Acc:$00.00\pm 0.00$}}\\
\end{tabular}}
\captionof{figure}{loss landscapes of first task after the completion of training first and last three tasks for split CIFAR-100 ($n=20$).}
\end{minipage}
\end{figure*}
